# Supplementary material for: Measurement of the ratio of branching fractions $\mathcal{B}(B_c^+ \to J/\psi \tau^+ \nu_{\tau})/\mathcal{B}(B_c^+ \to J/\psi \mu^+ \nu_{\mu})$
Source: arXiv:2606.10018 source file (2026-10-01)
Supplement: Supplementary file 1 [file supplementary.tex]

\clearpage

\section{Supplementary material for LHCb-PAPER-2026-018}
\label{sec:Supplementary-App}

\begin{figure}[b]
\centering
    \includegraphics[width=0.3\textwidth]{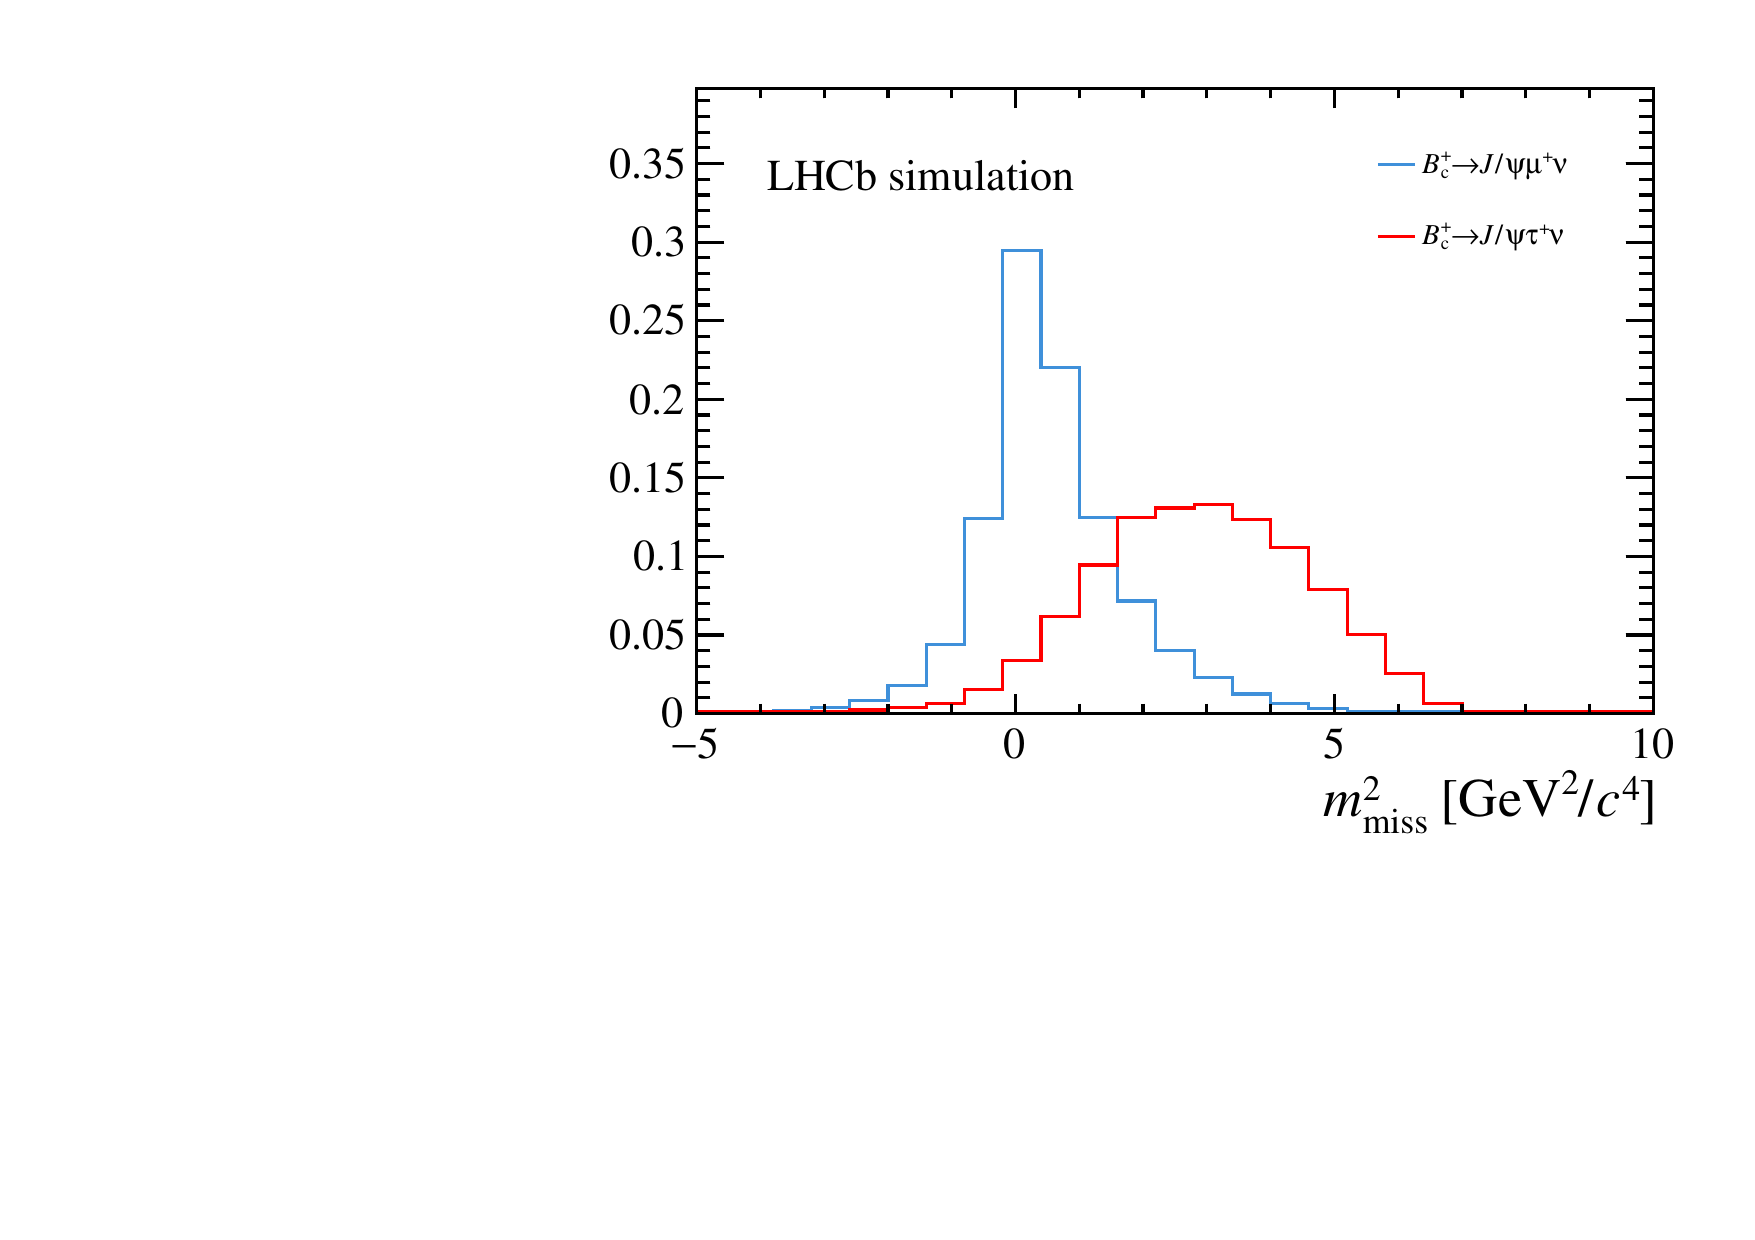}
    \includegraphics[width=0.3\textwidth]{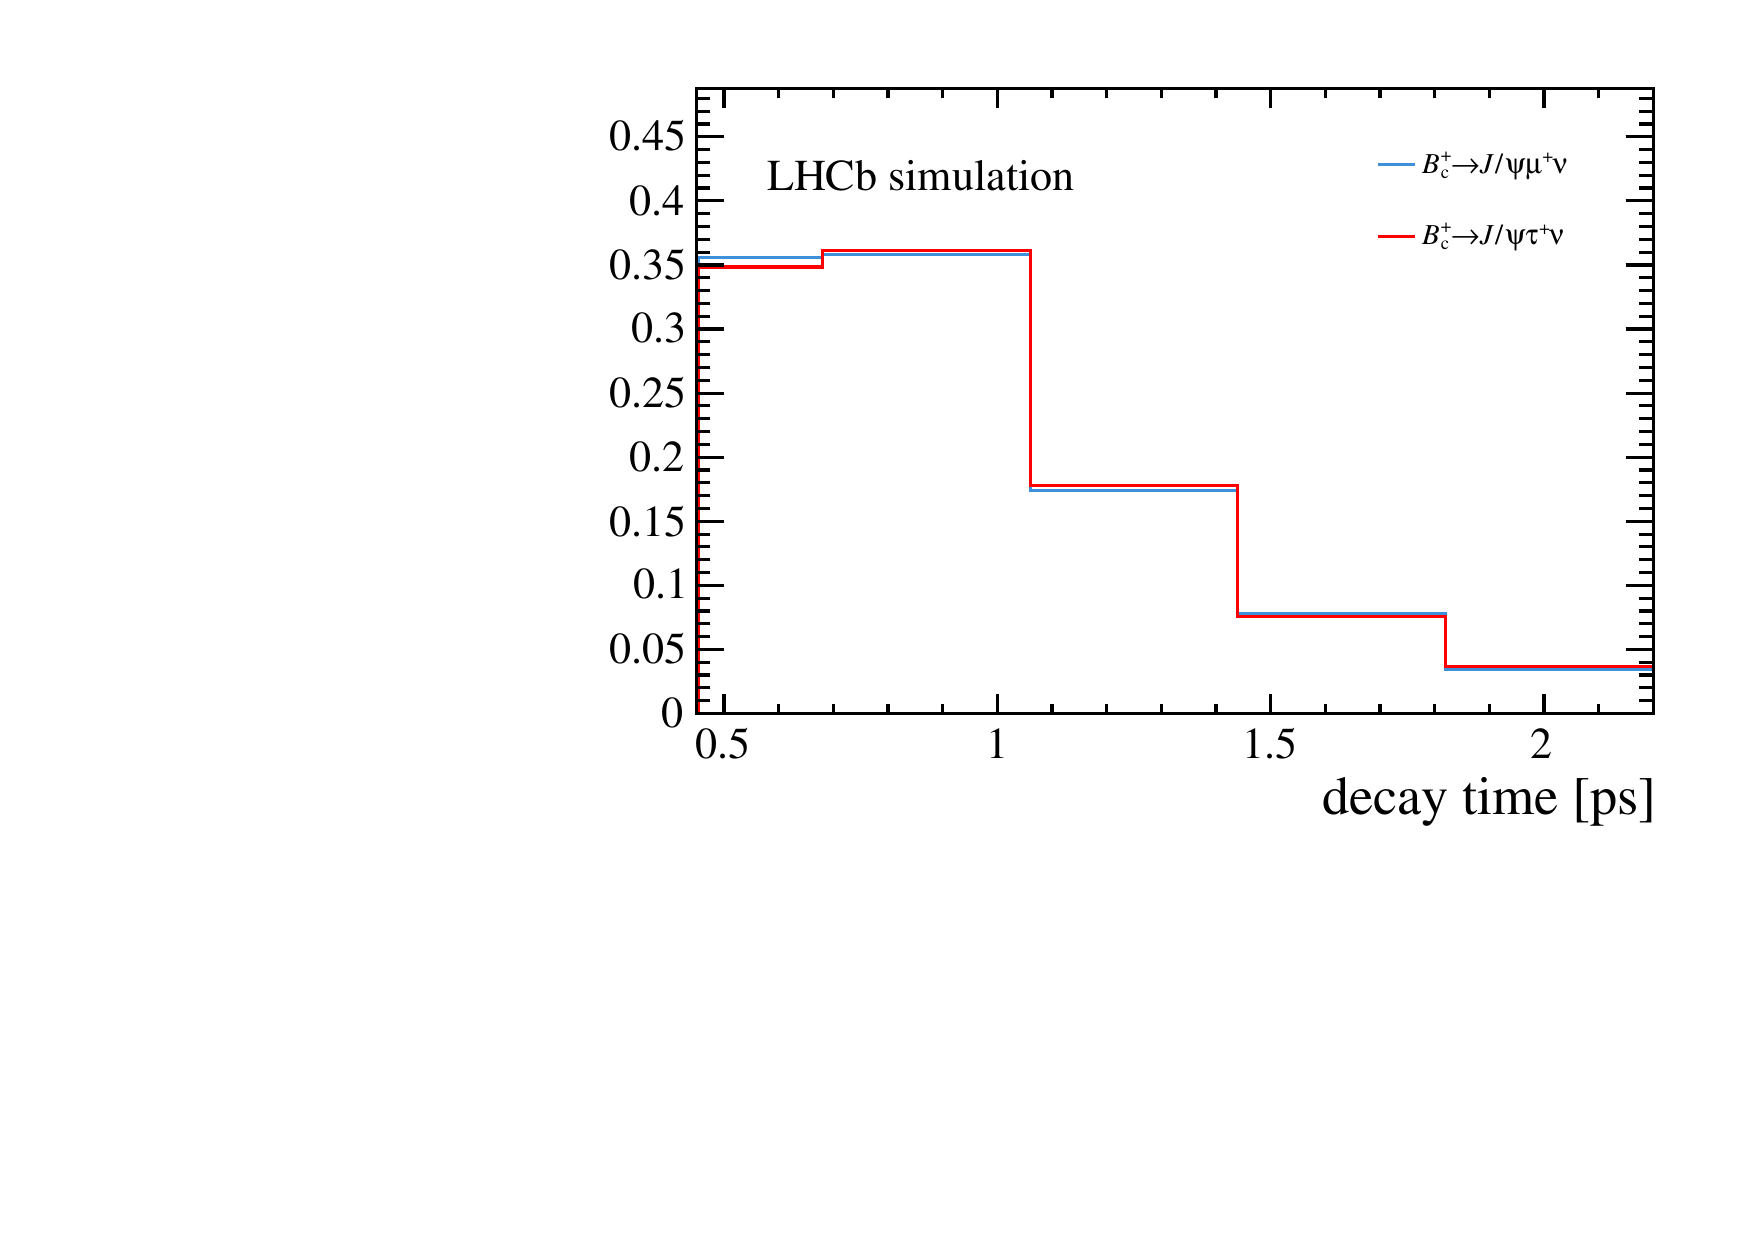}
    \includegraphics[width=0.3\textwidth]{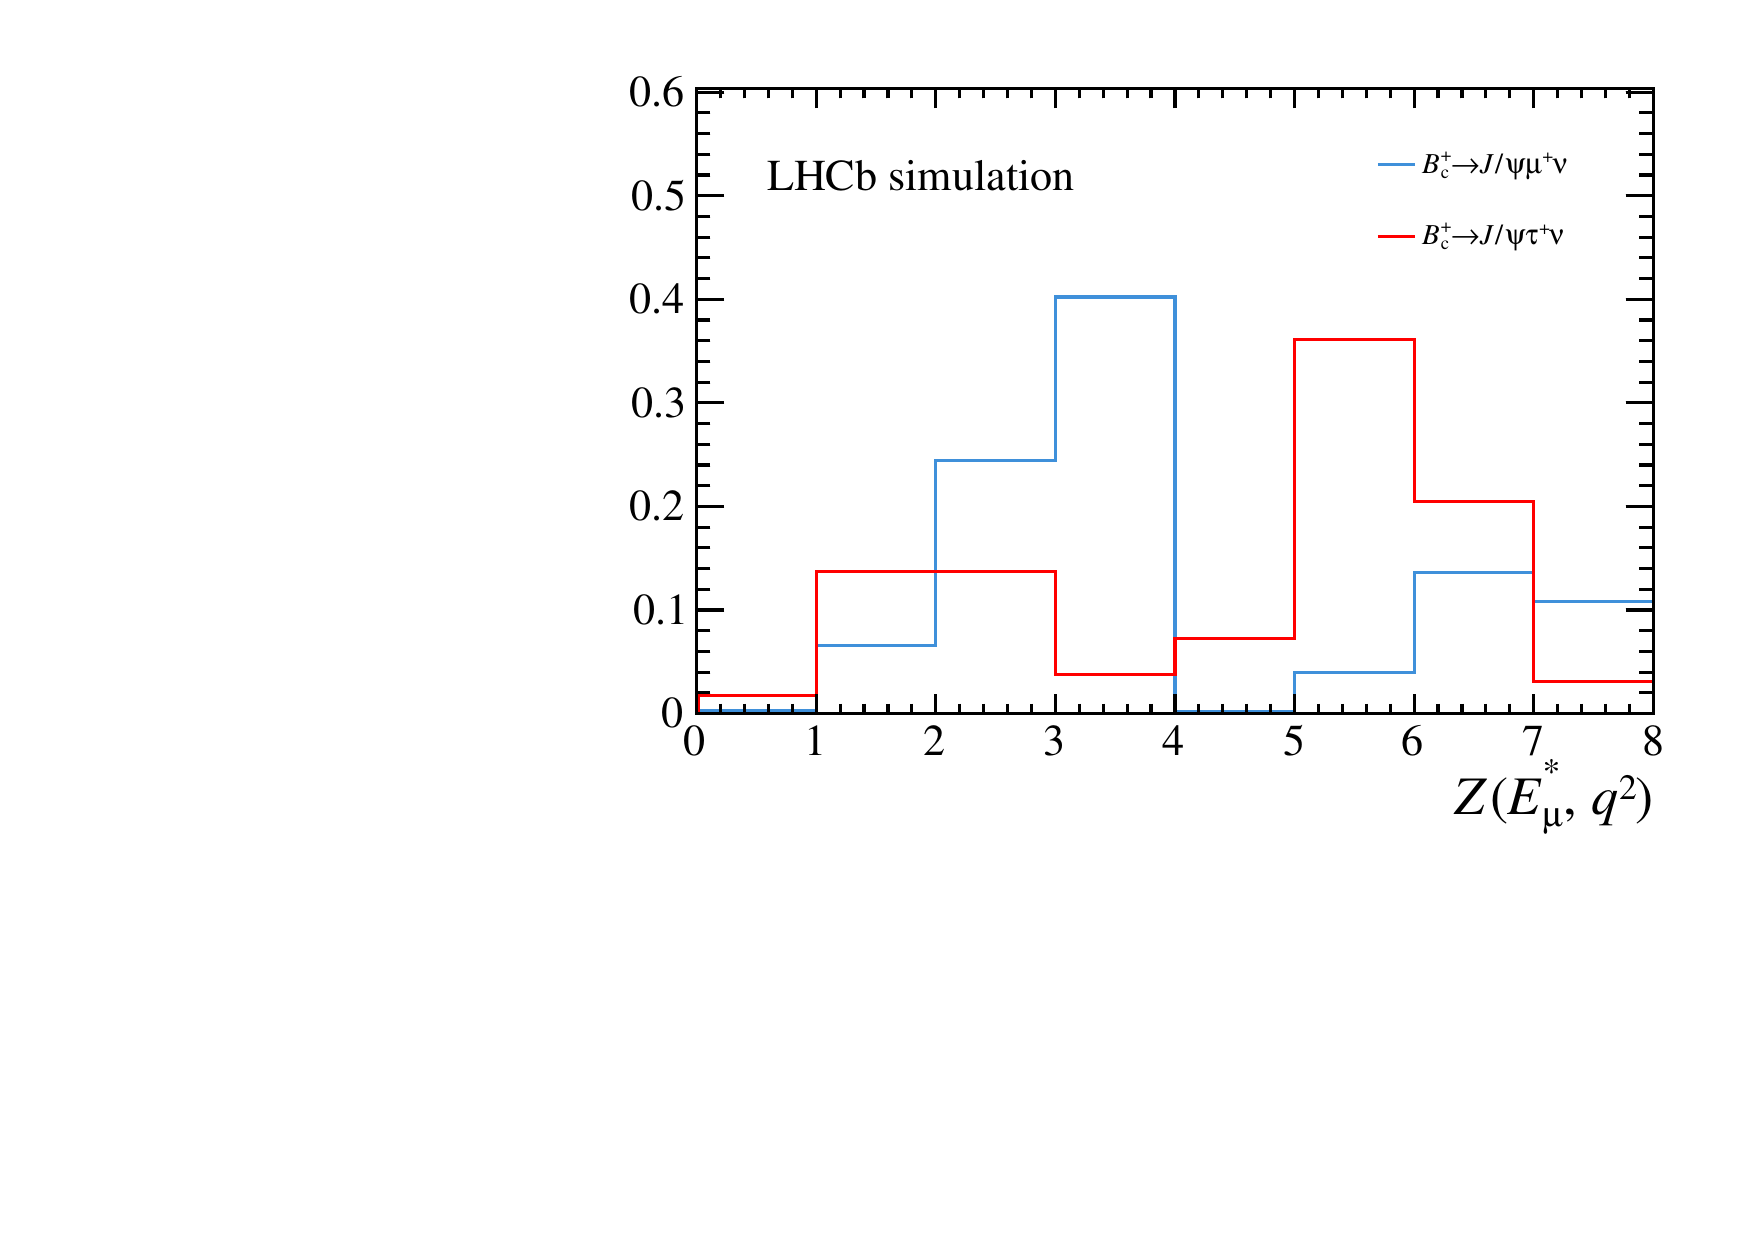}
    \caption{The distributions of rest-frame variables for the normalization (blue) compared with the signal (red) modes.}
    \label{fig:bc2jpsimu_templates}
\end{figure}

\begin{figure}[b]
\centering
    \includegraphics[width=0.3\textwidth]{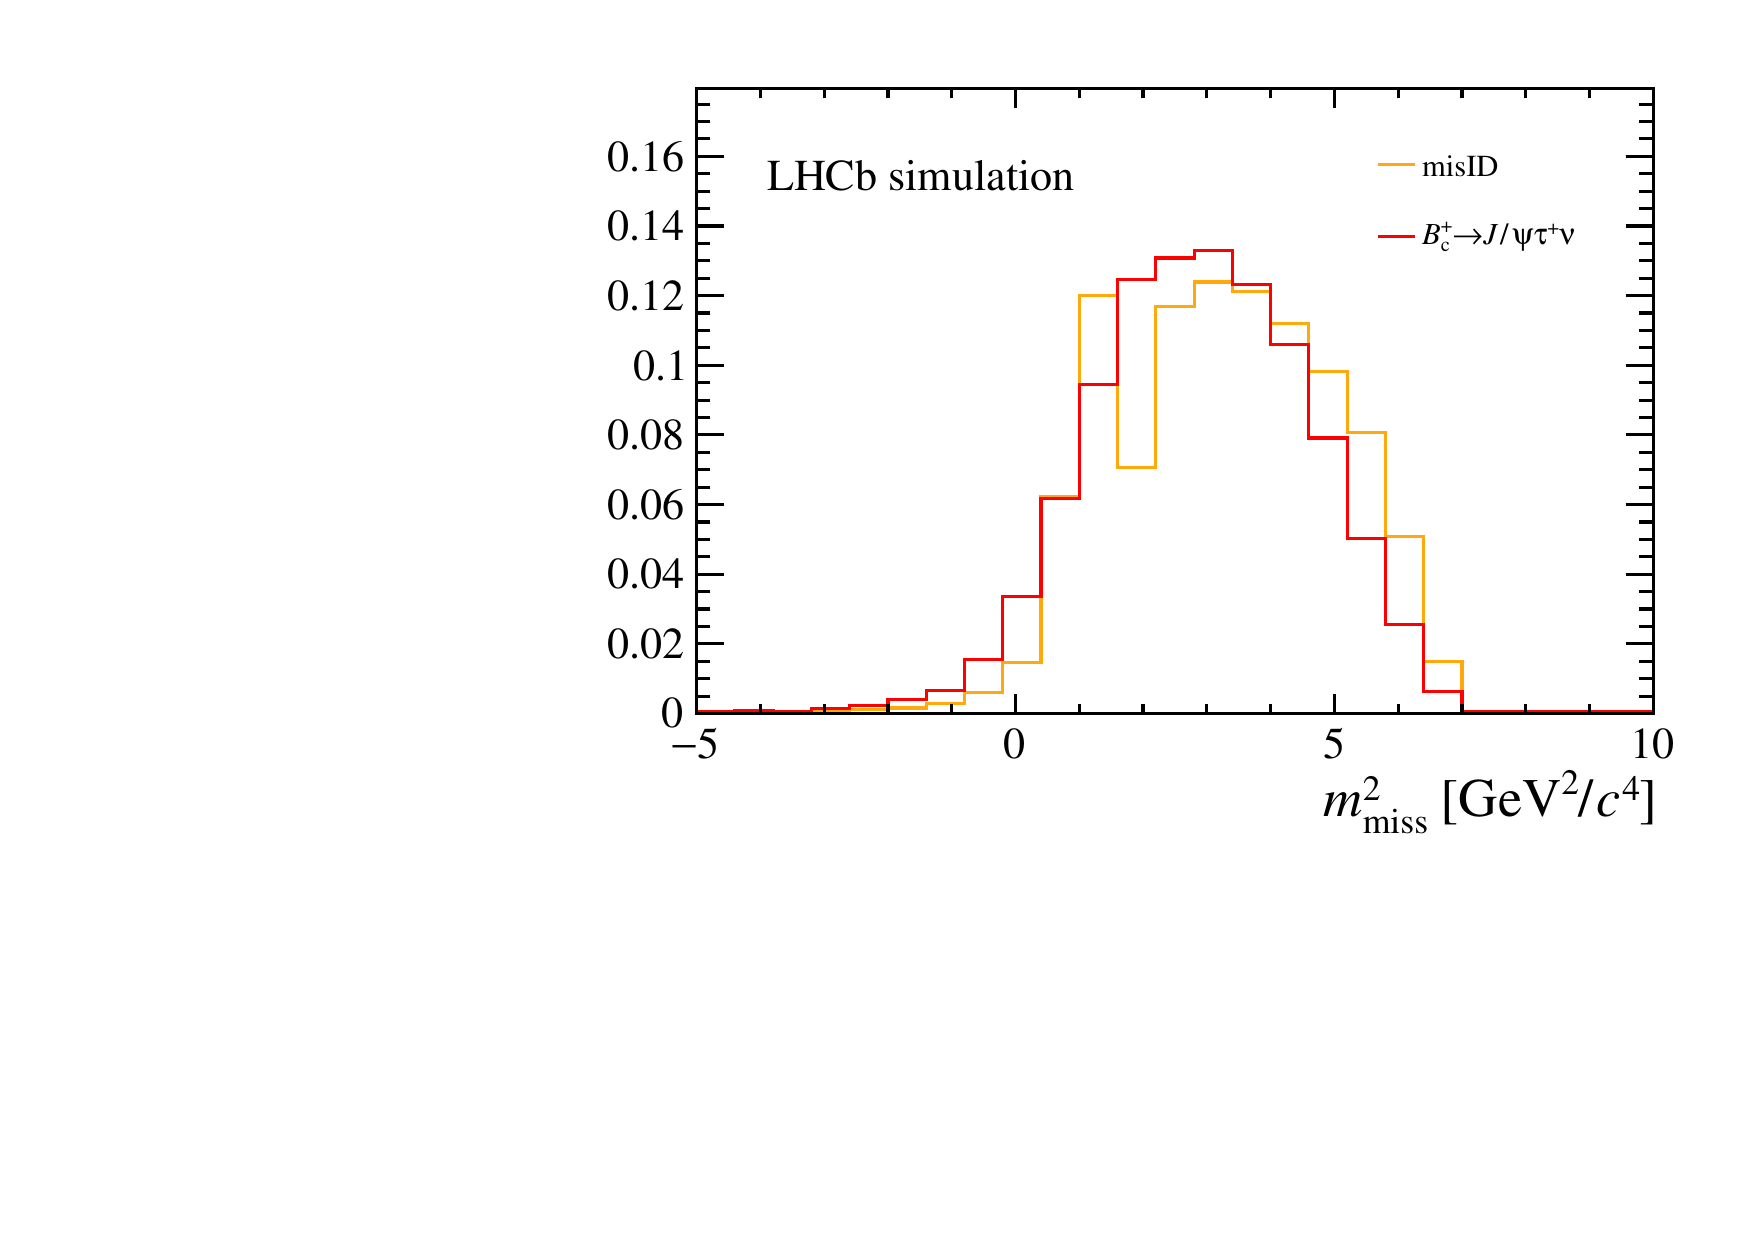}
    \includegraphics[width=0.3\textwidth]{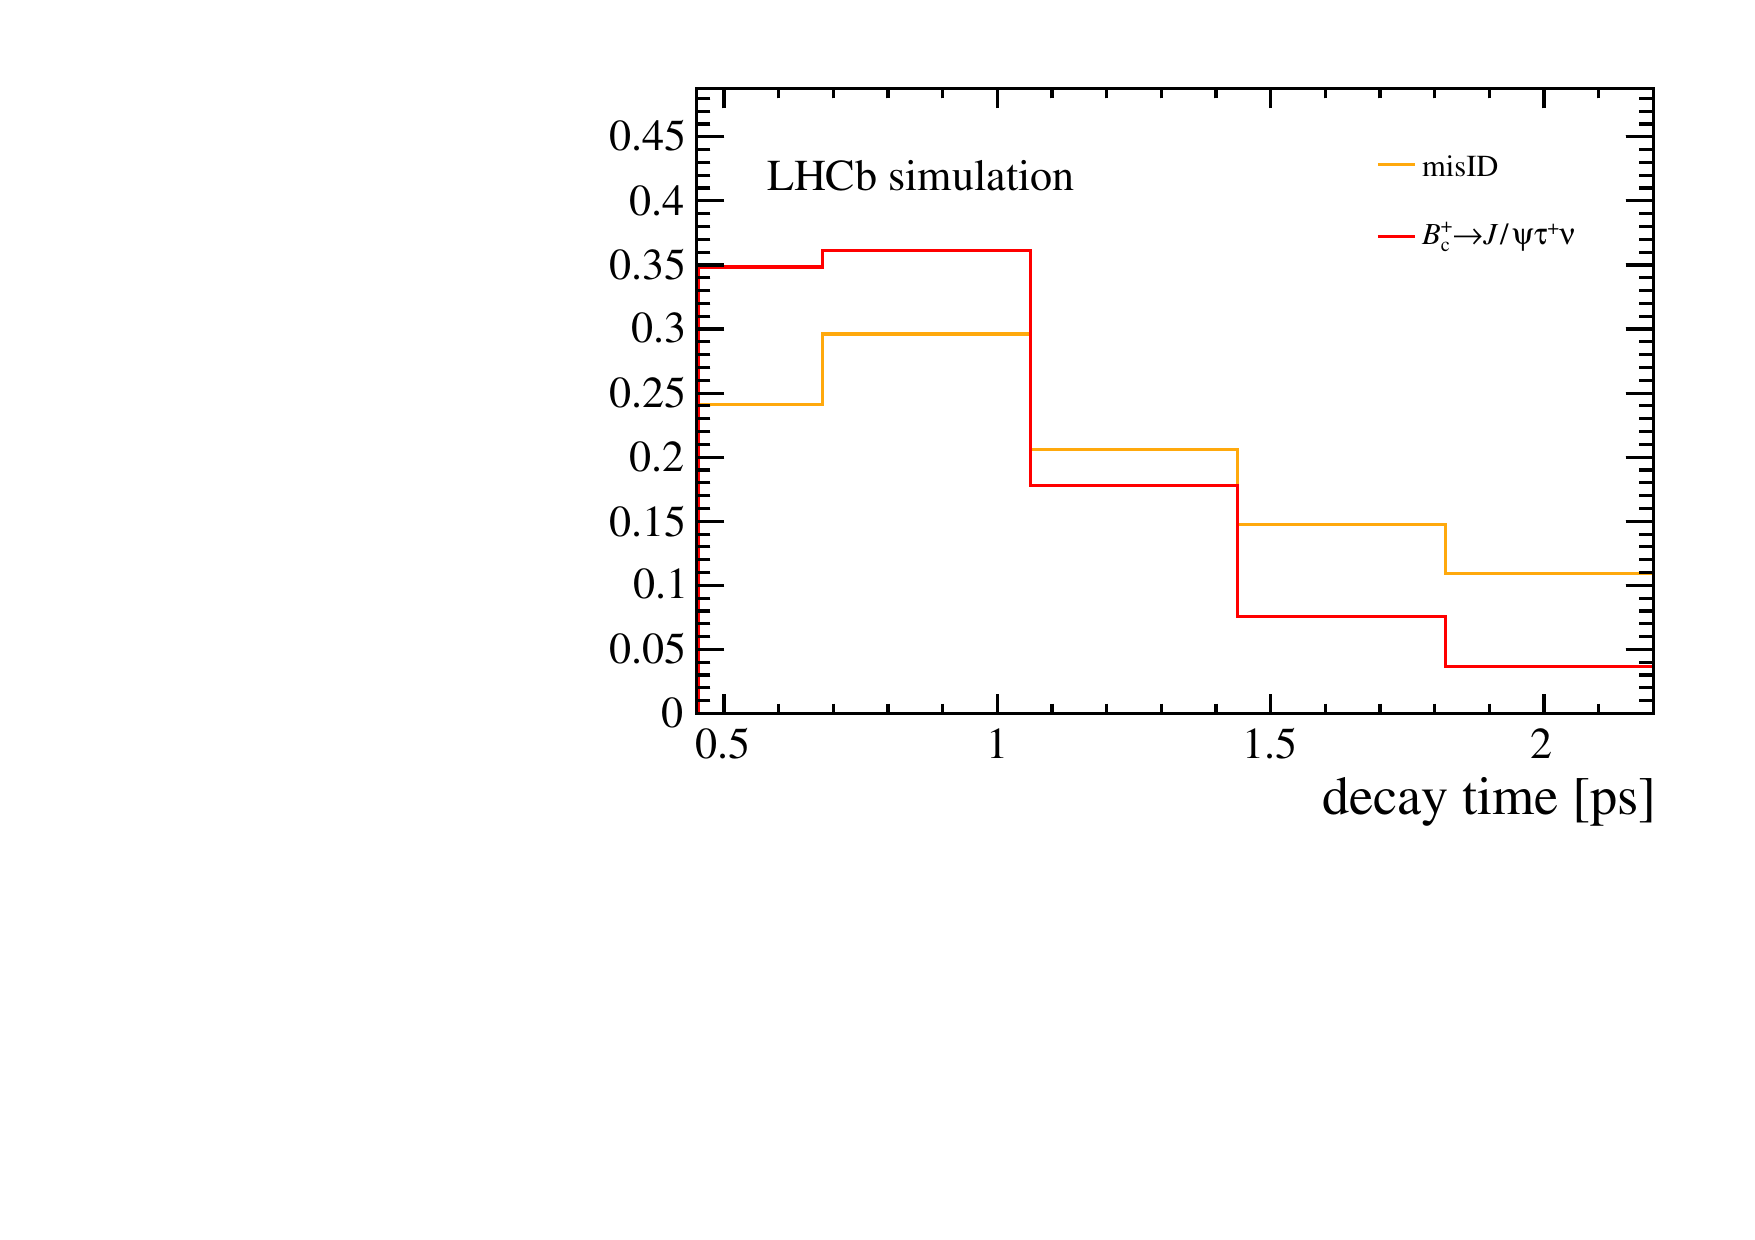}
    \includegraphics[width=0.3\textwidth]{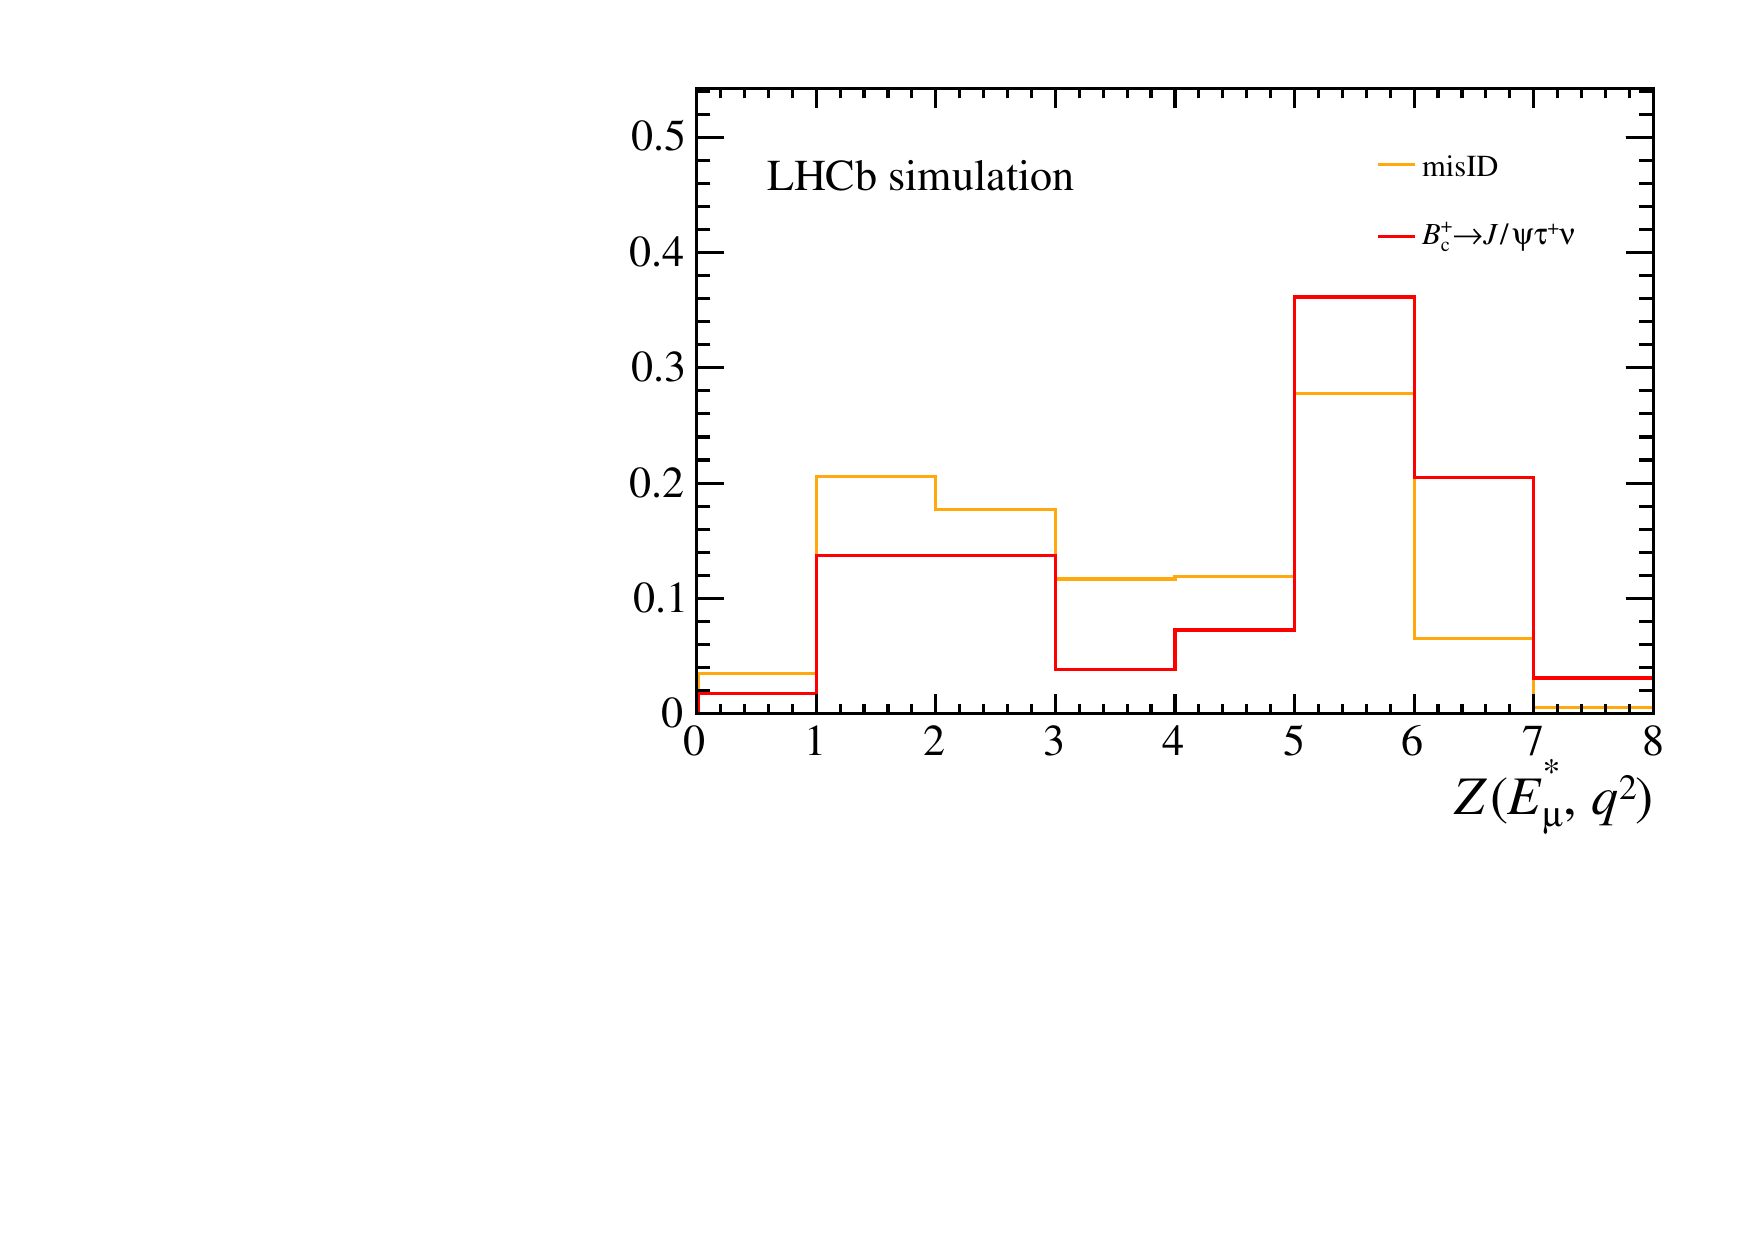}
    \includegraphics[width=0.3\textwidth]{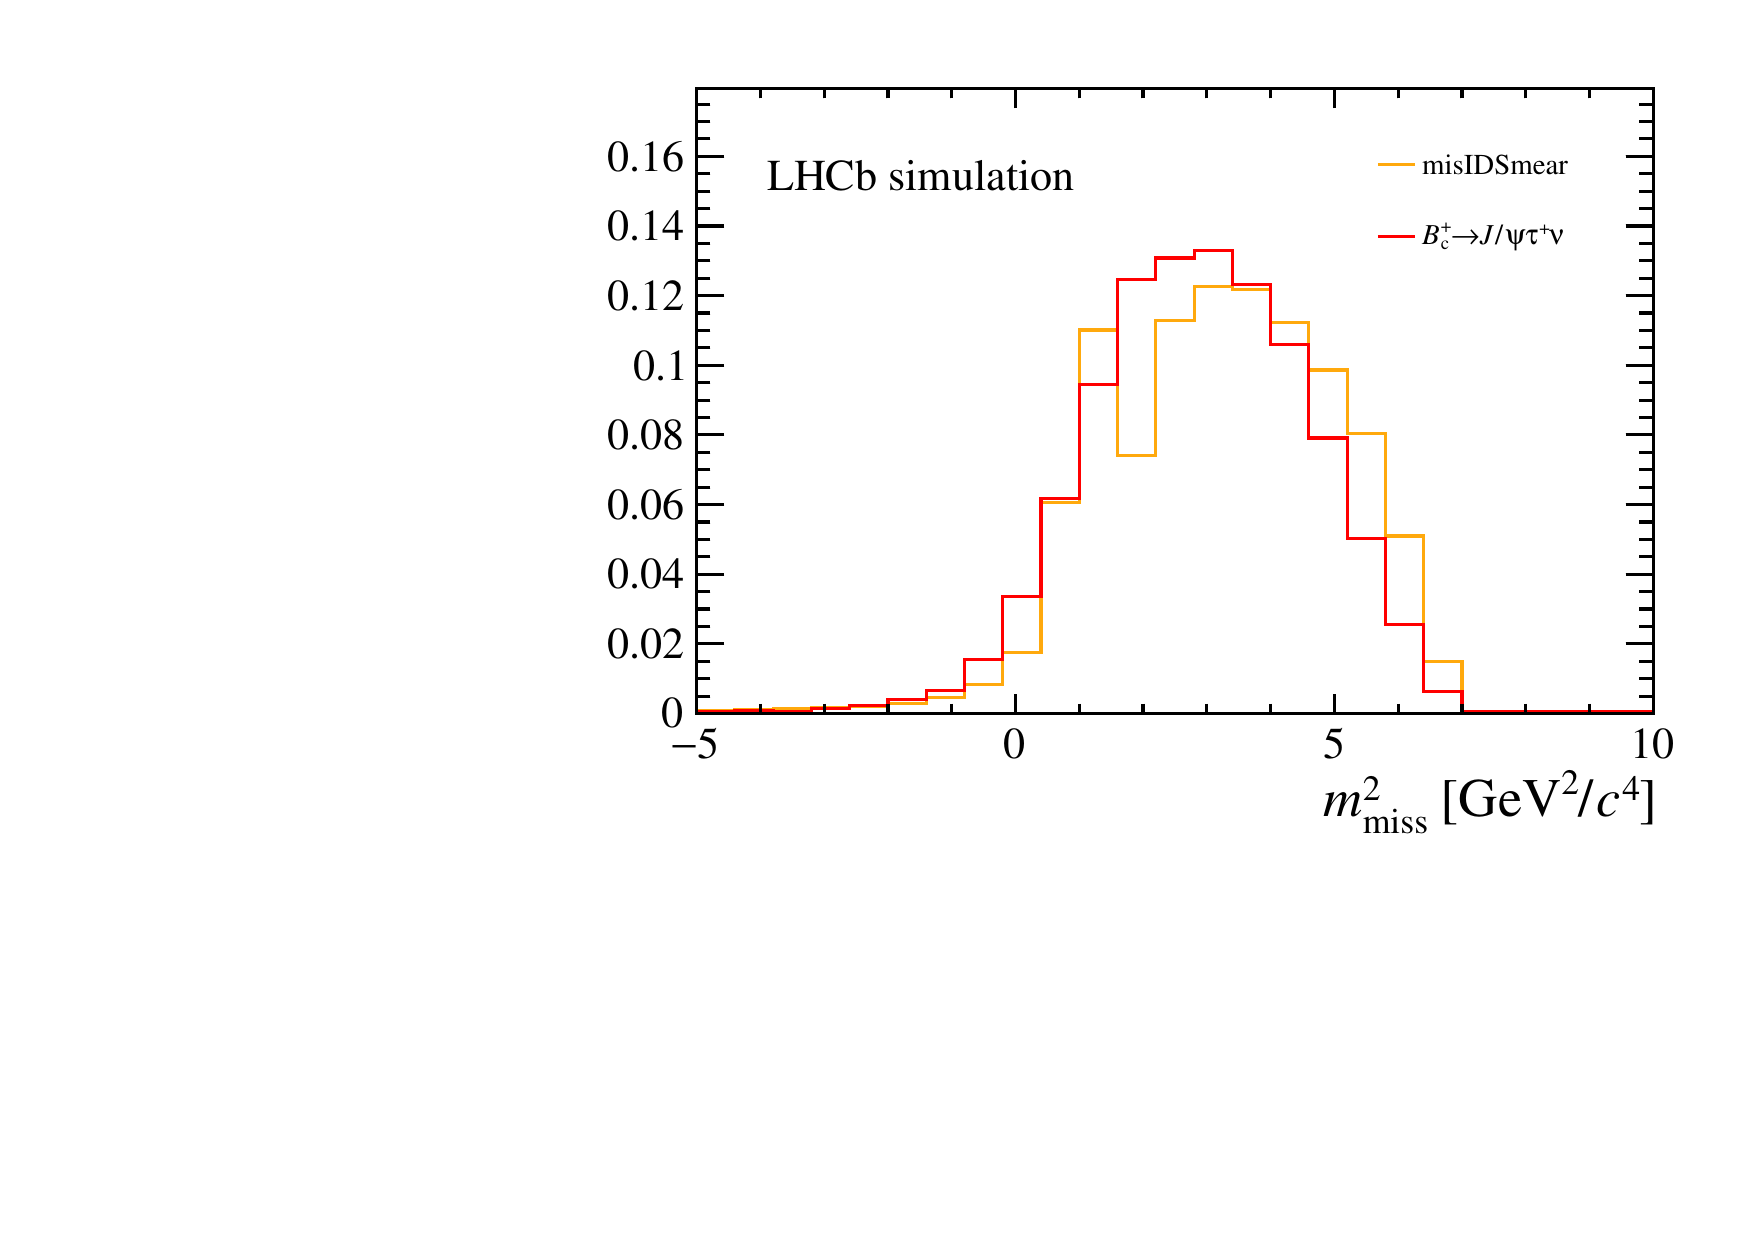}
    \includegraphics[width=0.3\textwidth]{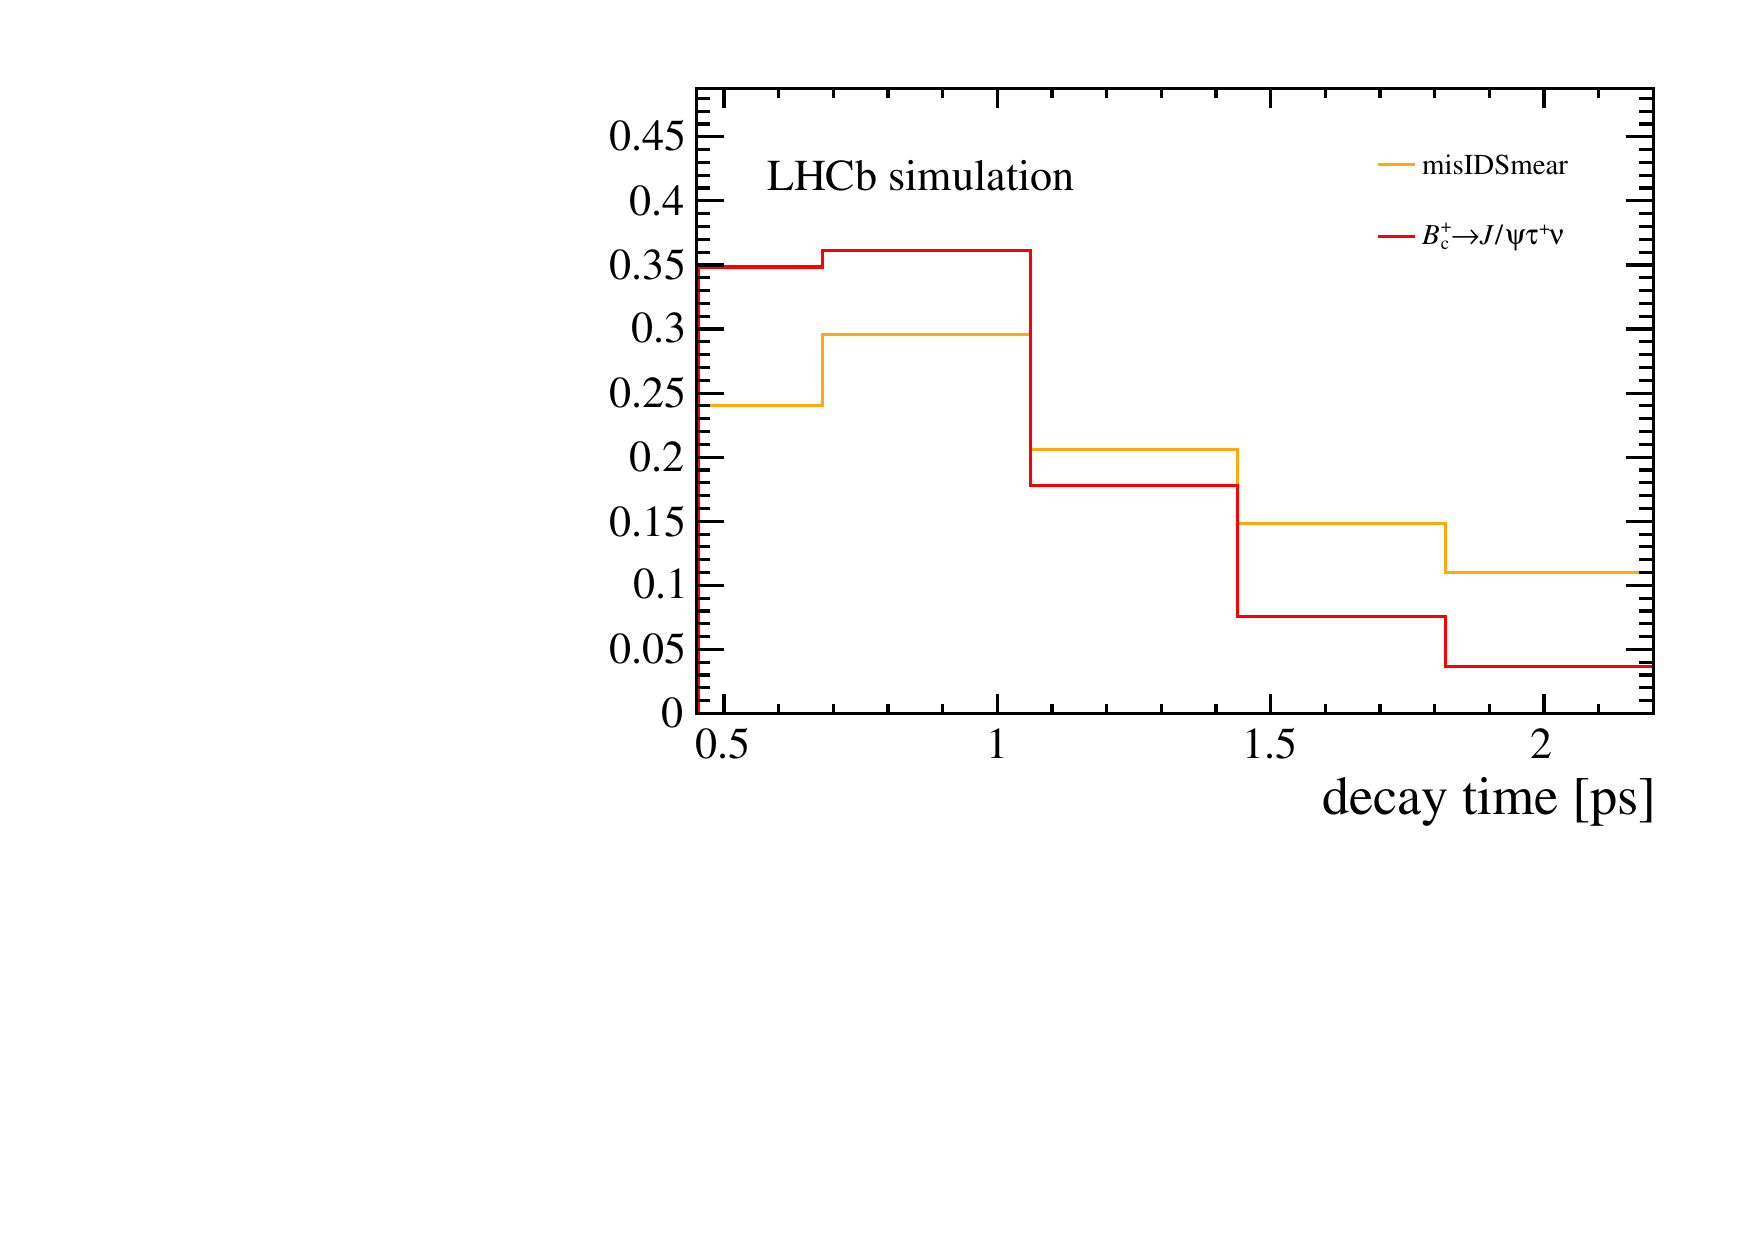}
    \includegraphics[width=0.3\textwidth]{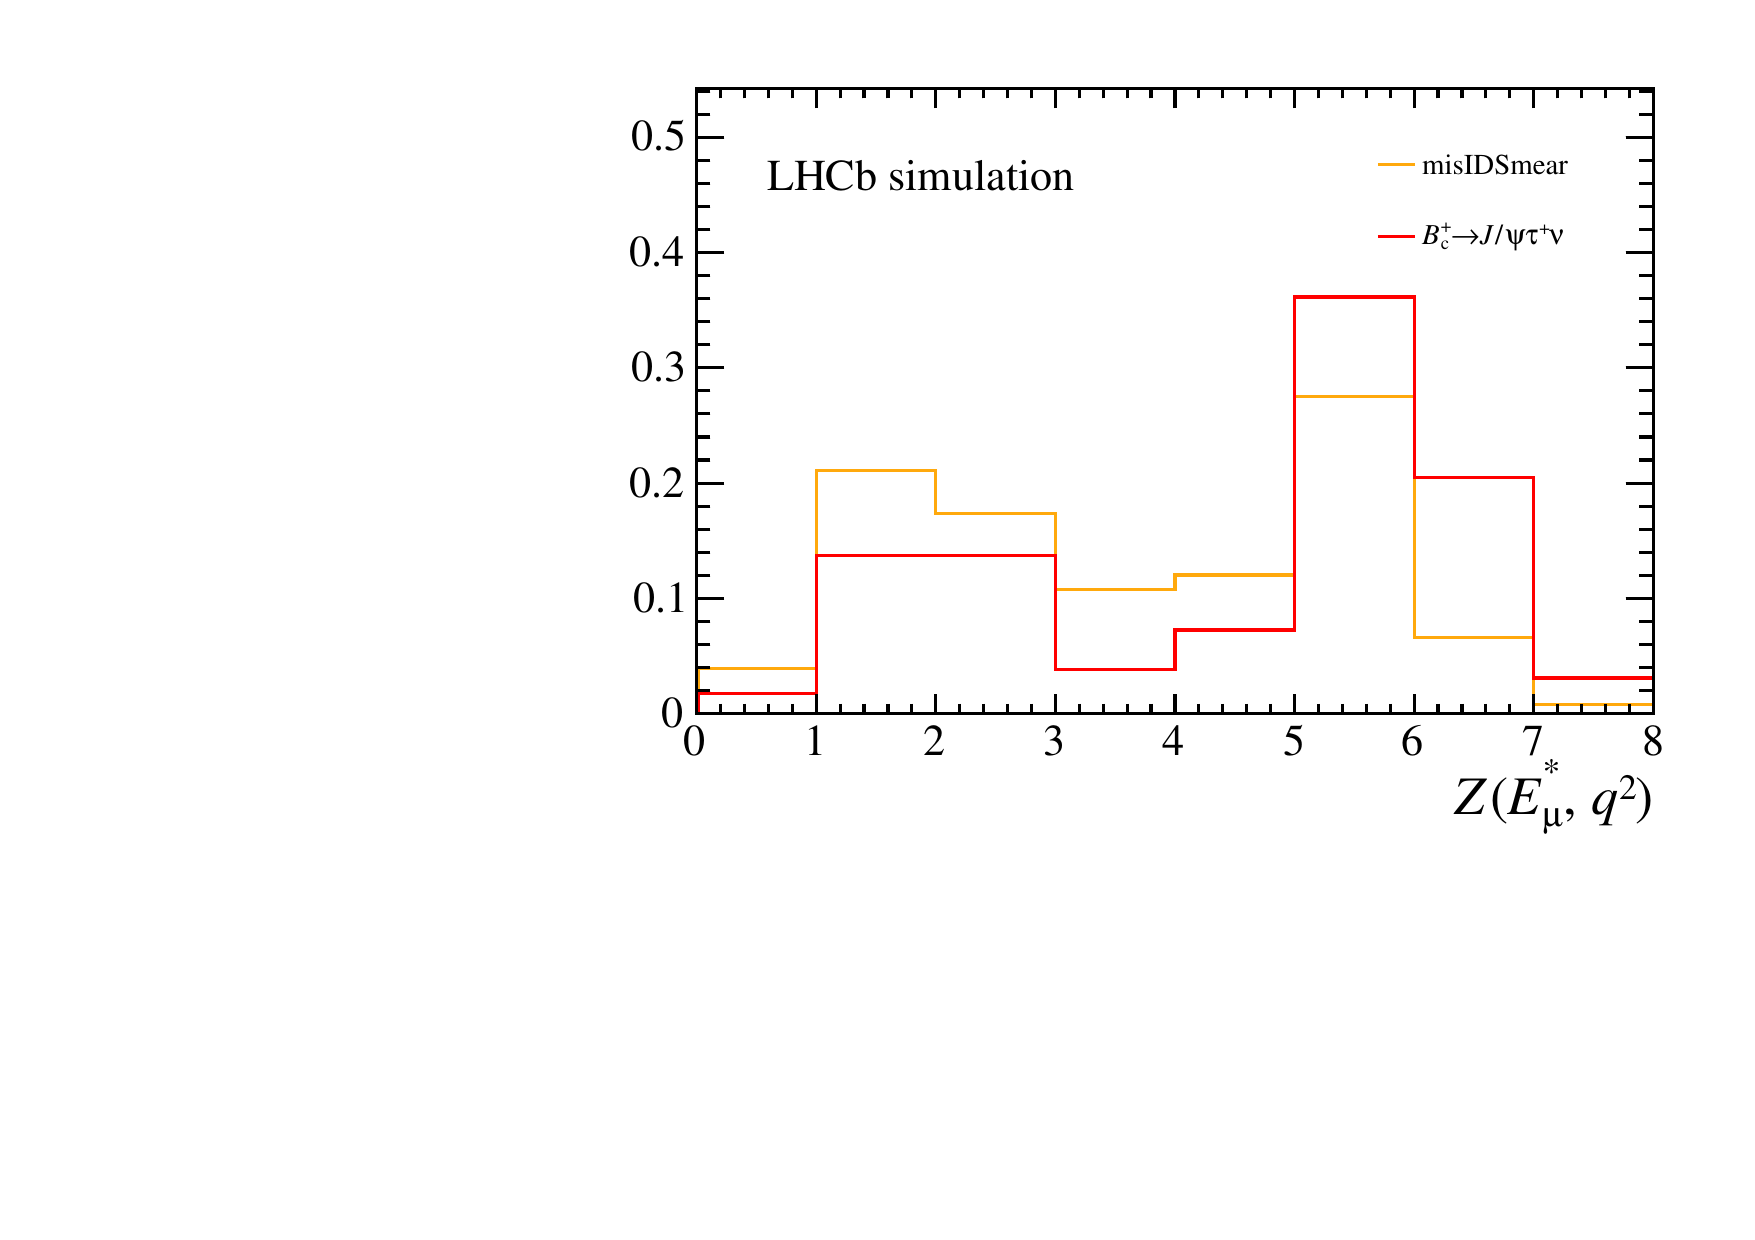}   

    \caption{The distributions of rest-frame variables for the misID background (yellow) compared with the signal mode (red), with unsmeared data on the top row and smeared data on the bottom row.}
    \label{fig:bc2jpsimu_templates}
\end{figure}

\begin{figure}
\centering
    \includegraphics[width=0.3\textwidth]{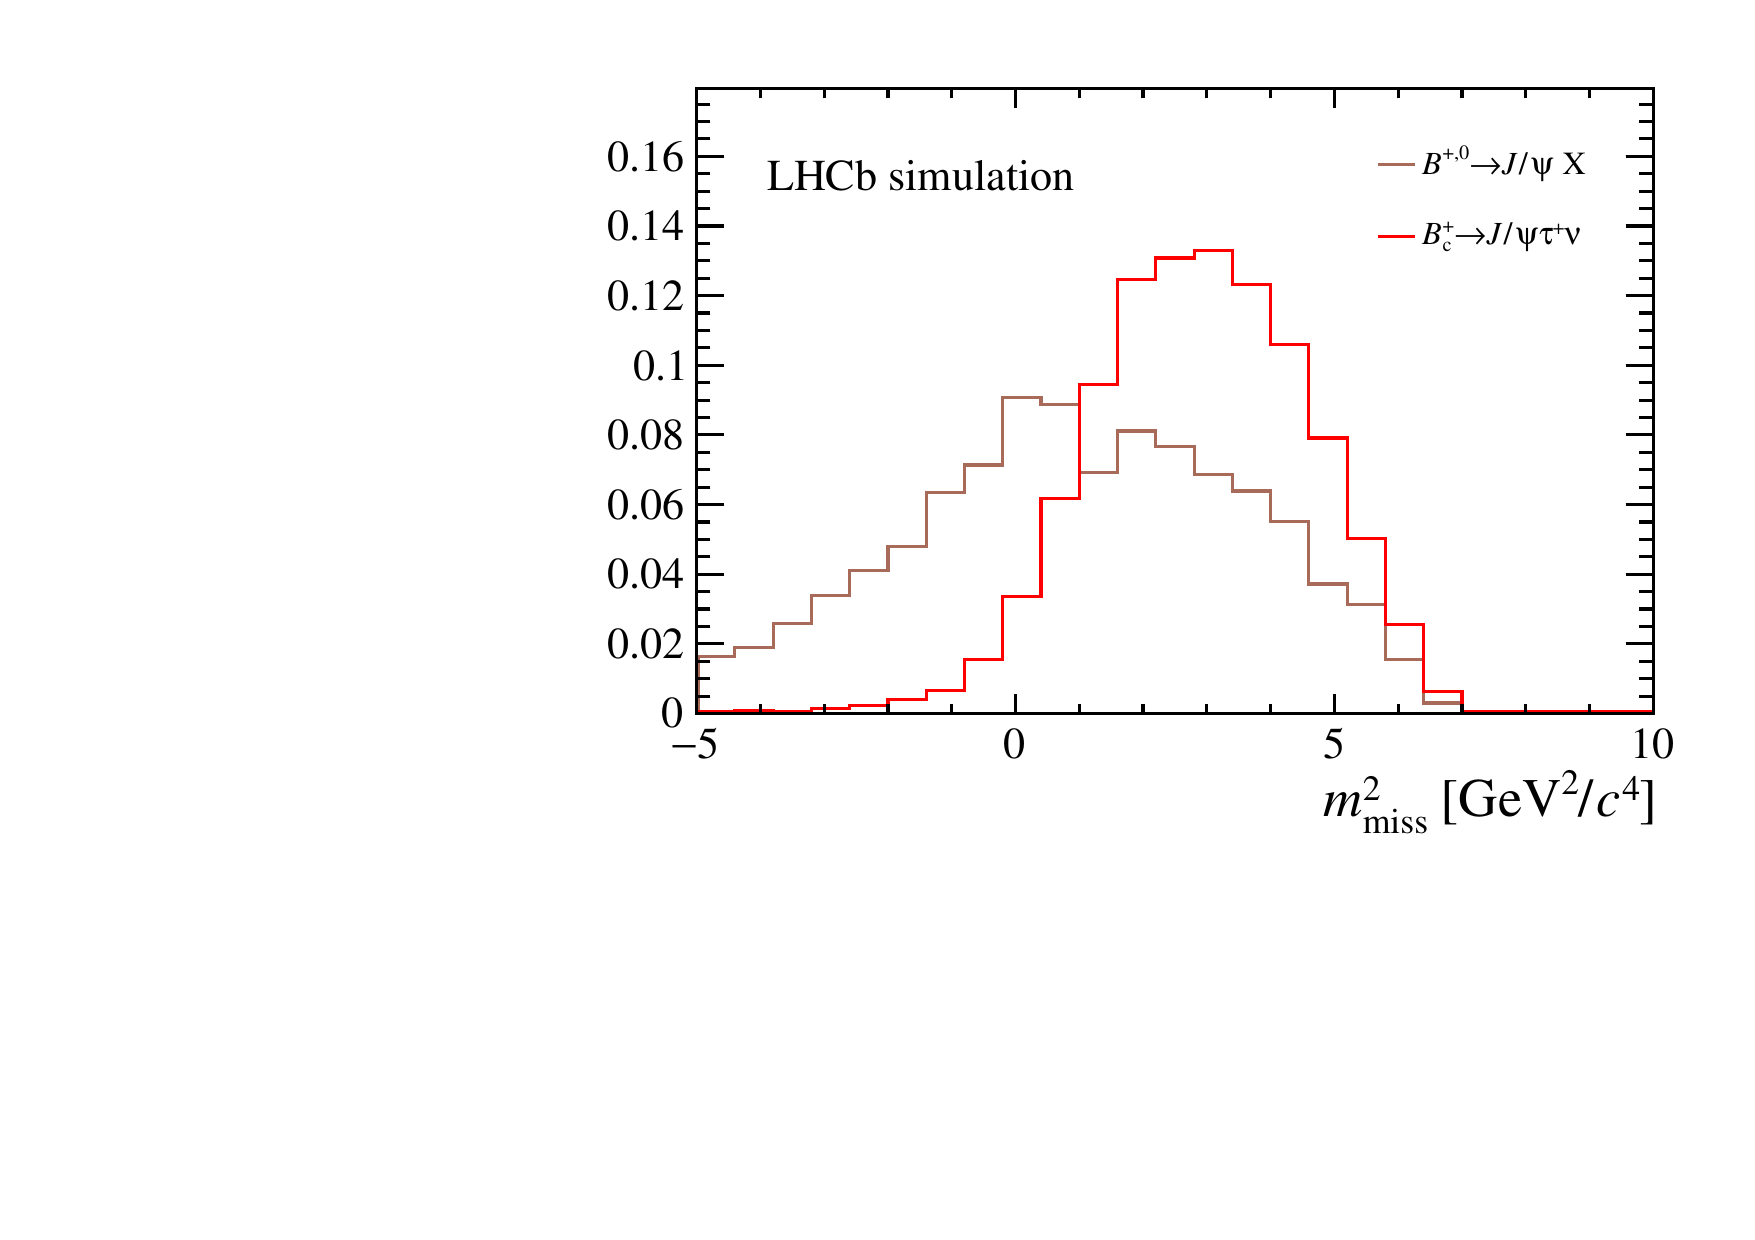}
    \includegraphics[width=0.3\textwidth]{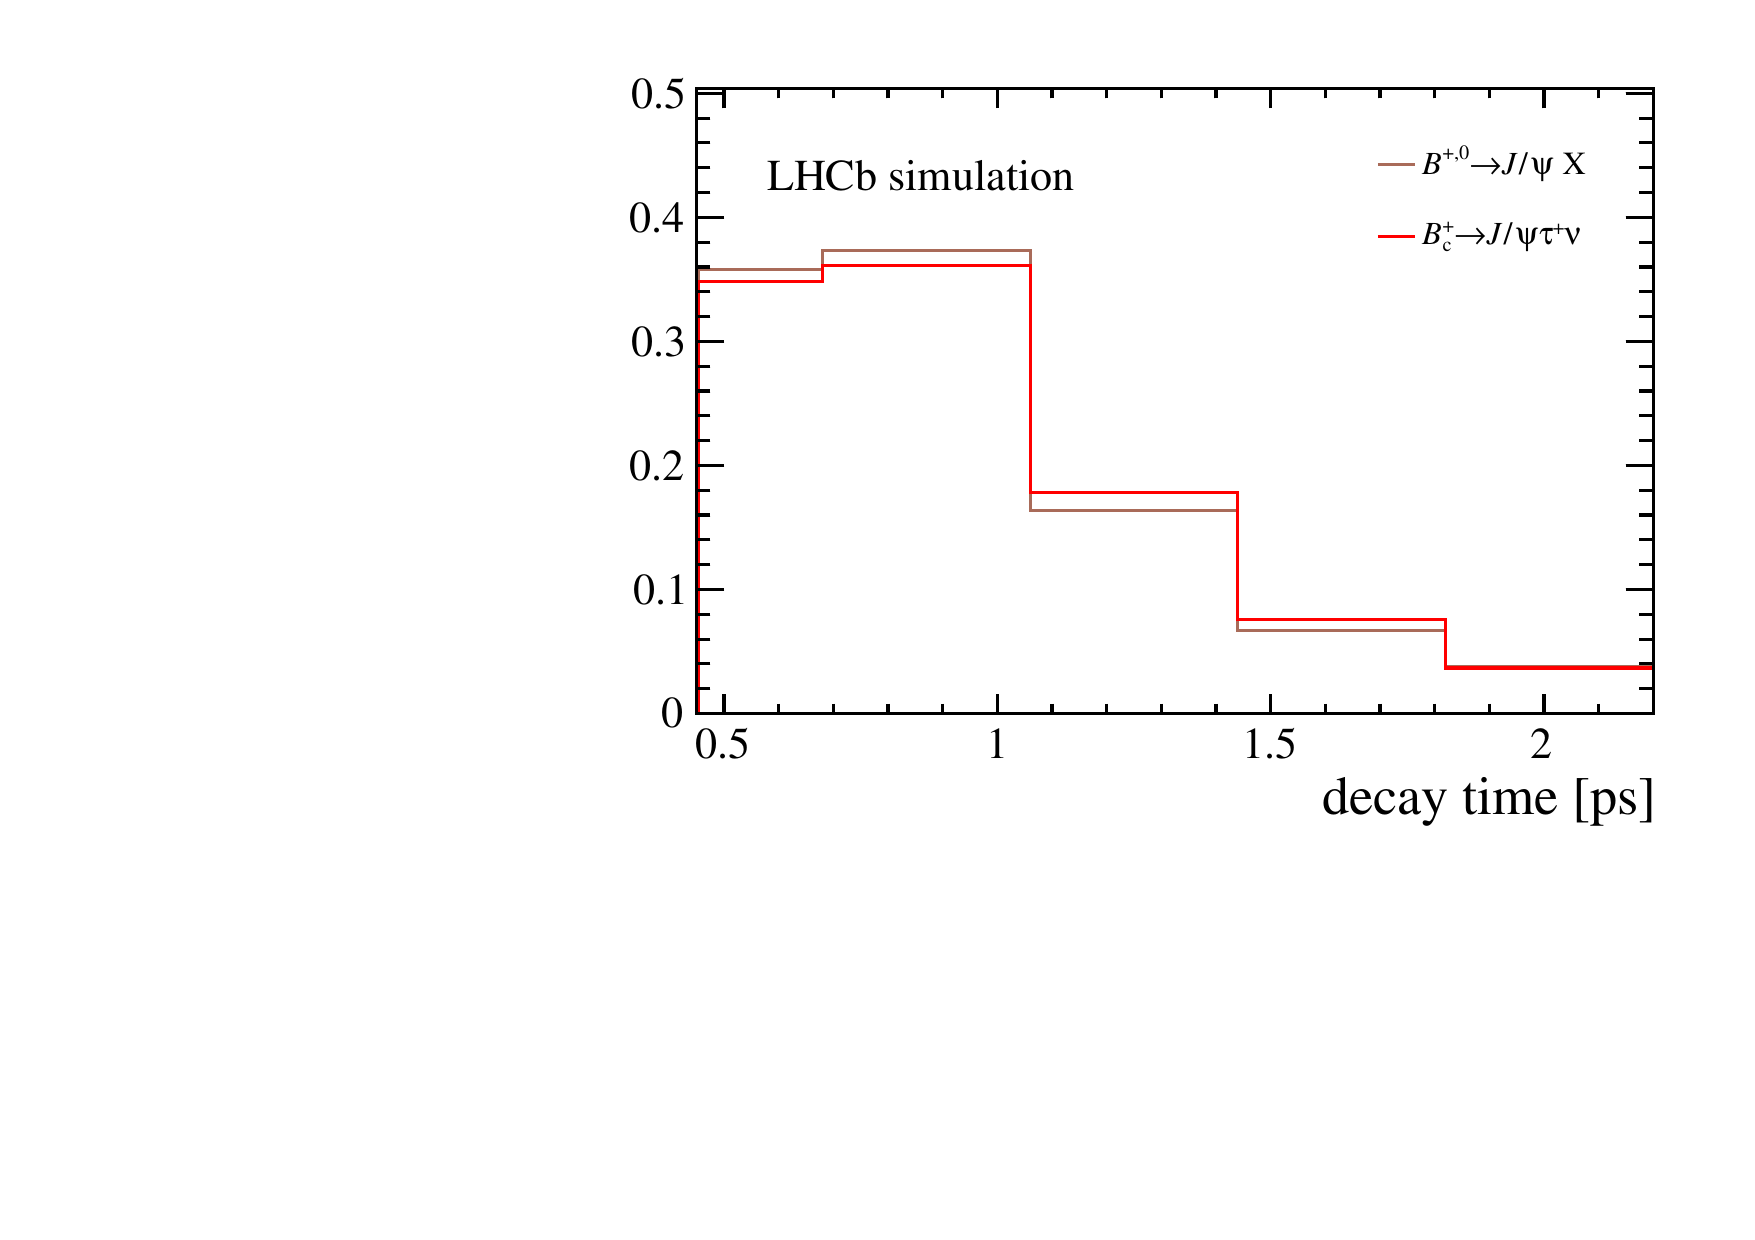}
    \includegraphics[width=0.3\textwidth]{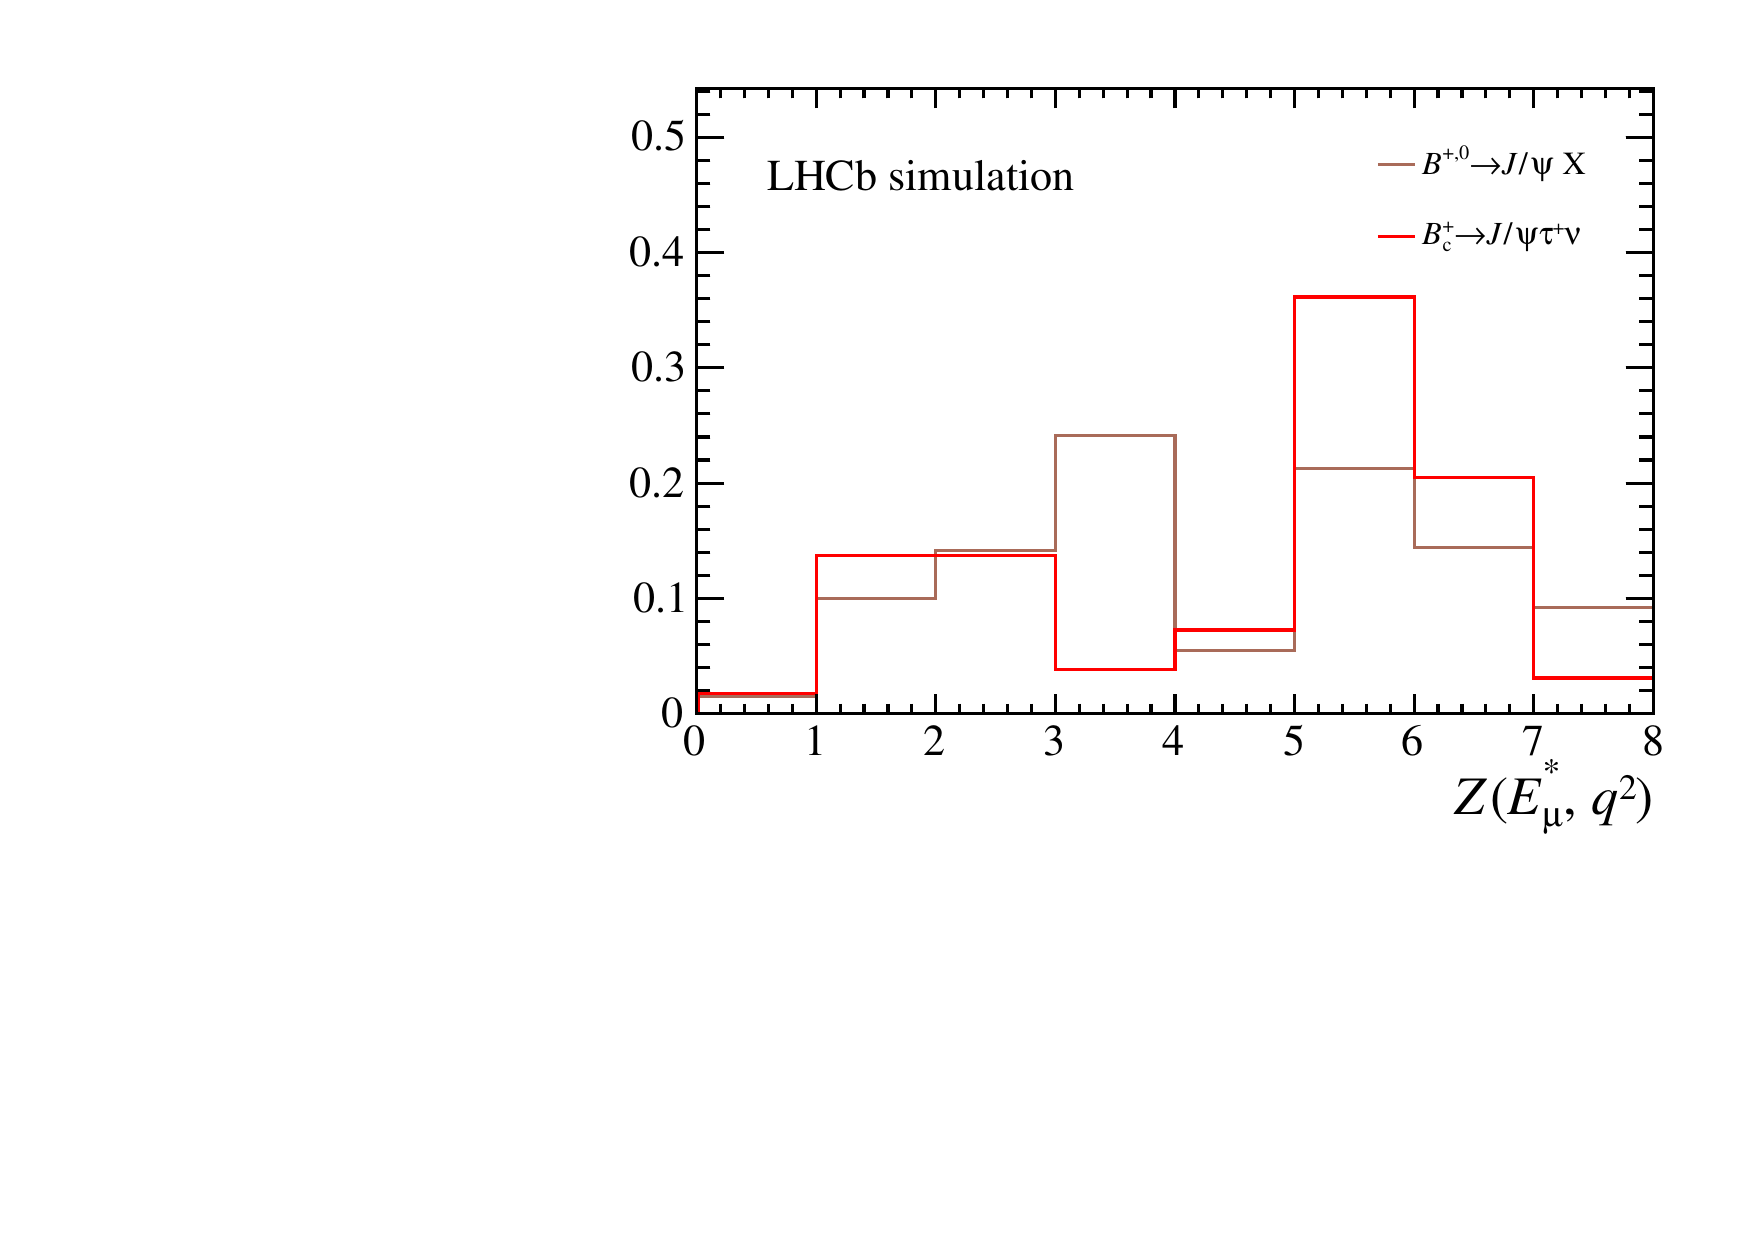}
    \includegraphics[width=0.3\textwidth]{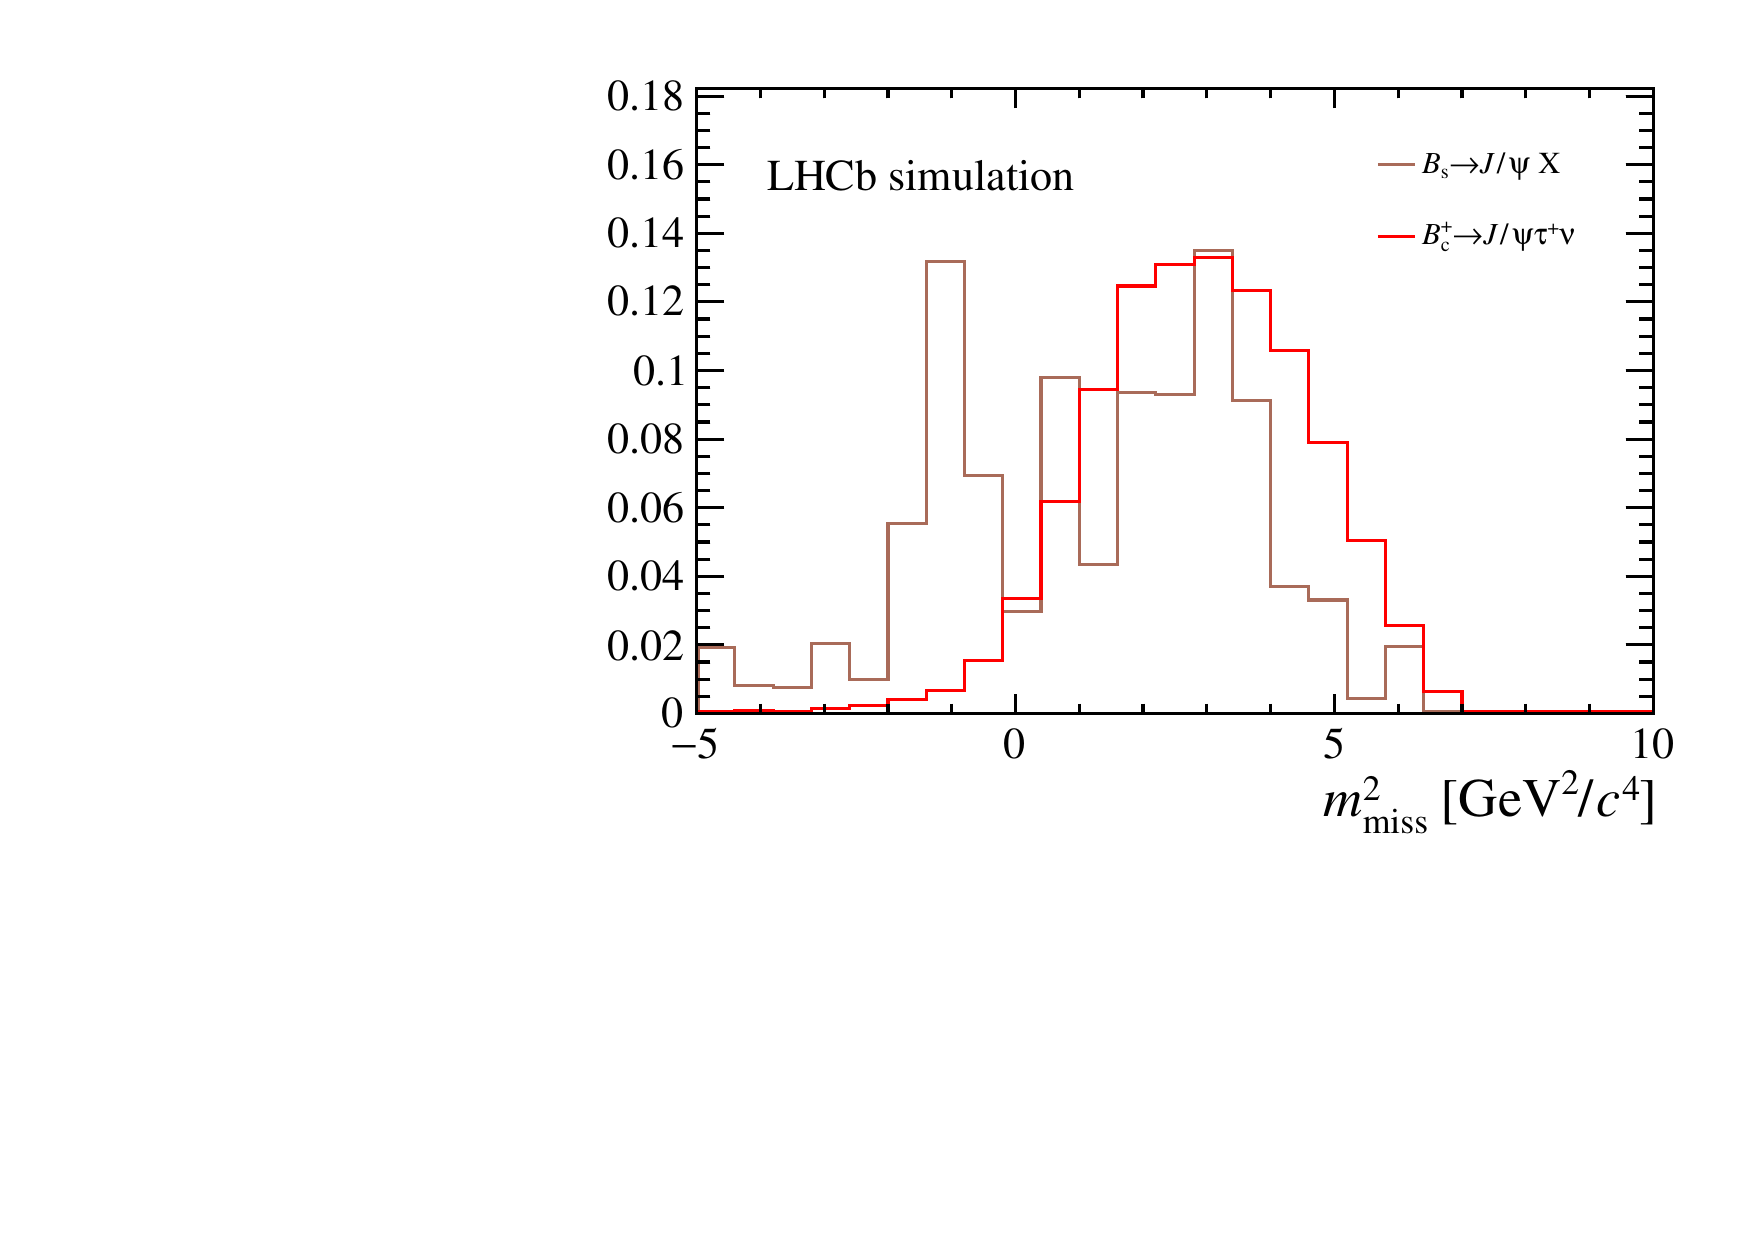}
    \includegraphics[width=0.3\textwidth]{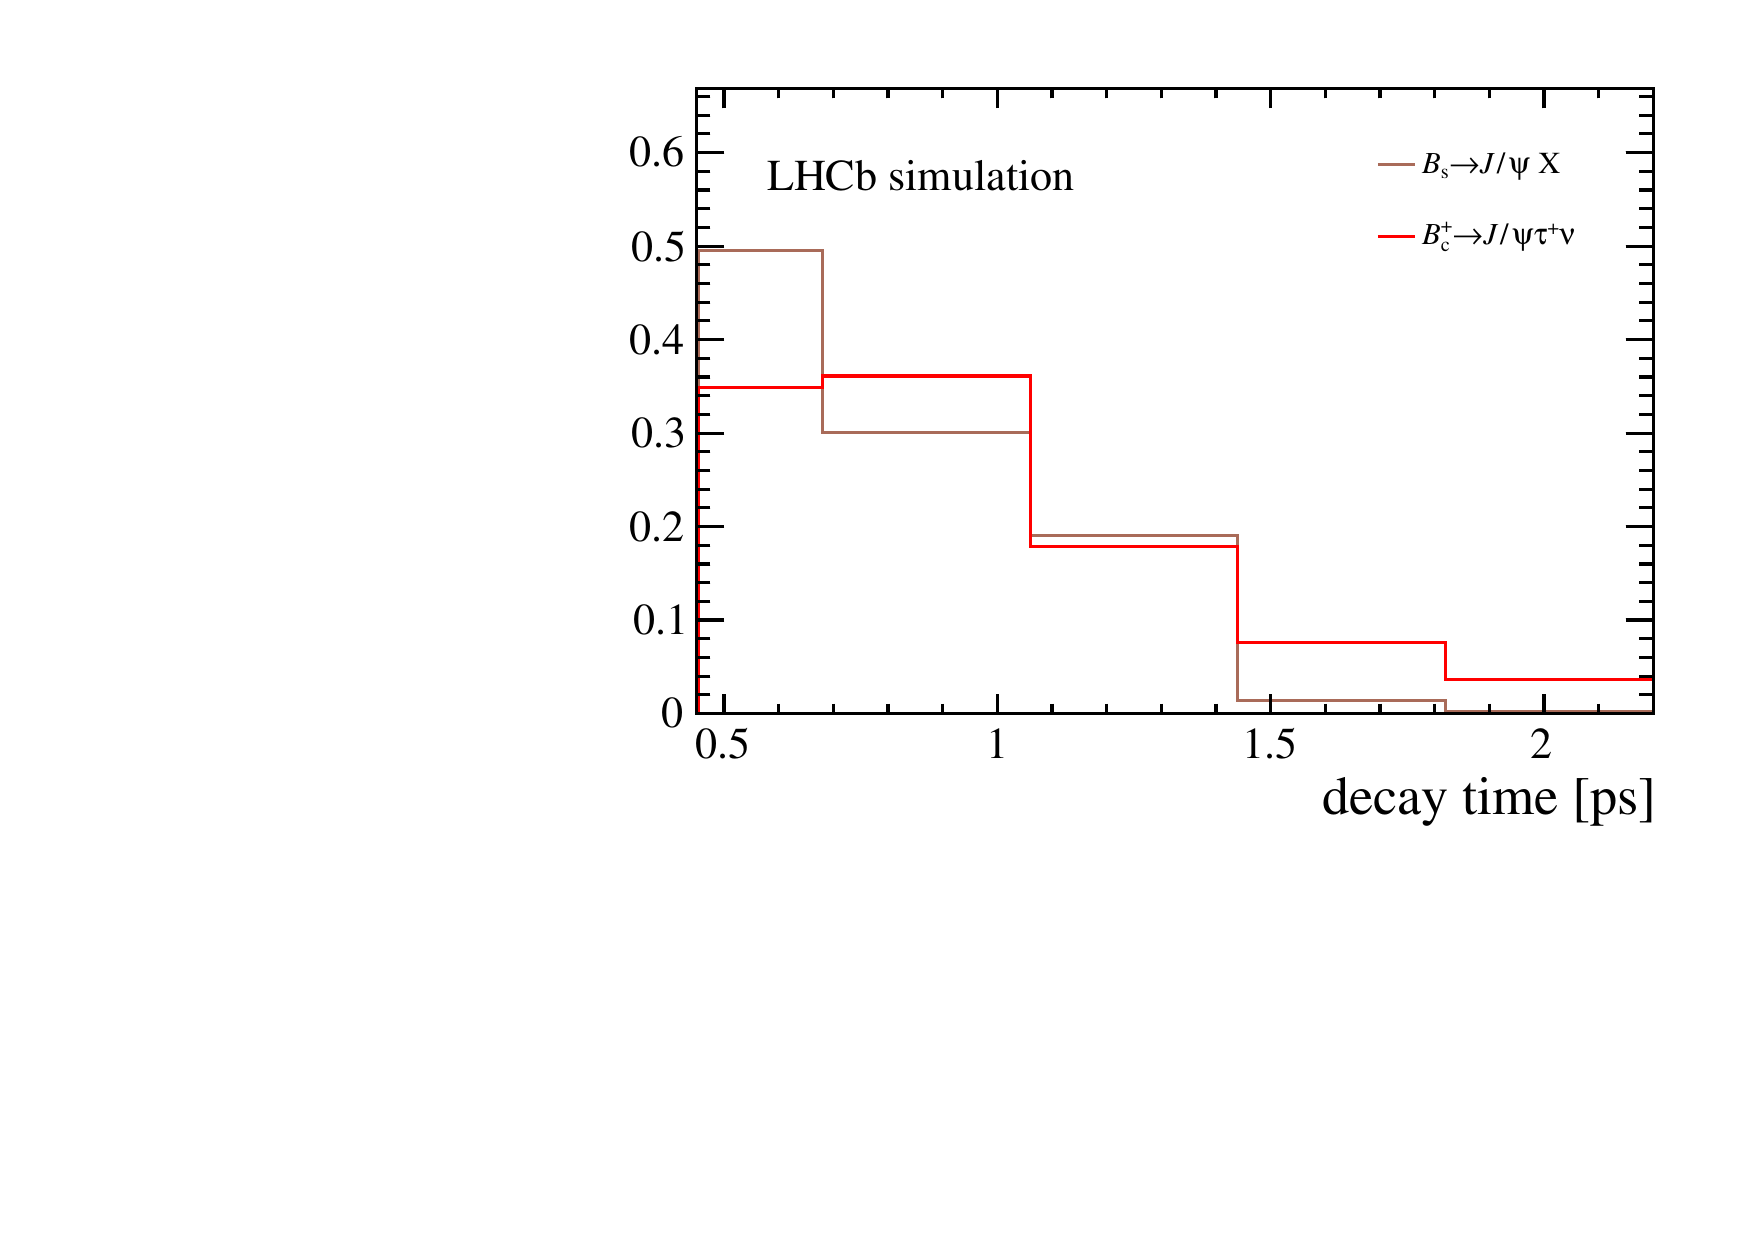}
    \includegraphics[width=0.3\textwidth]{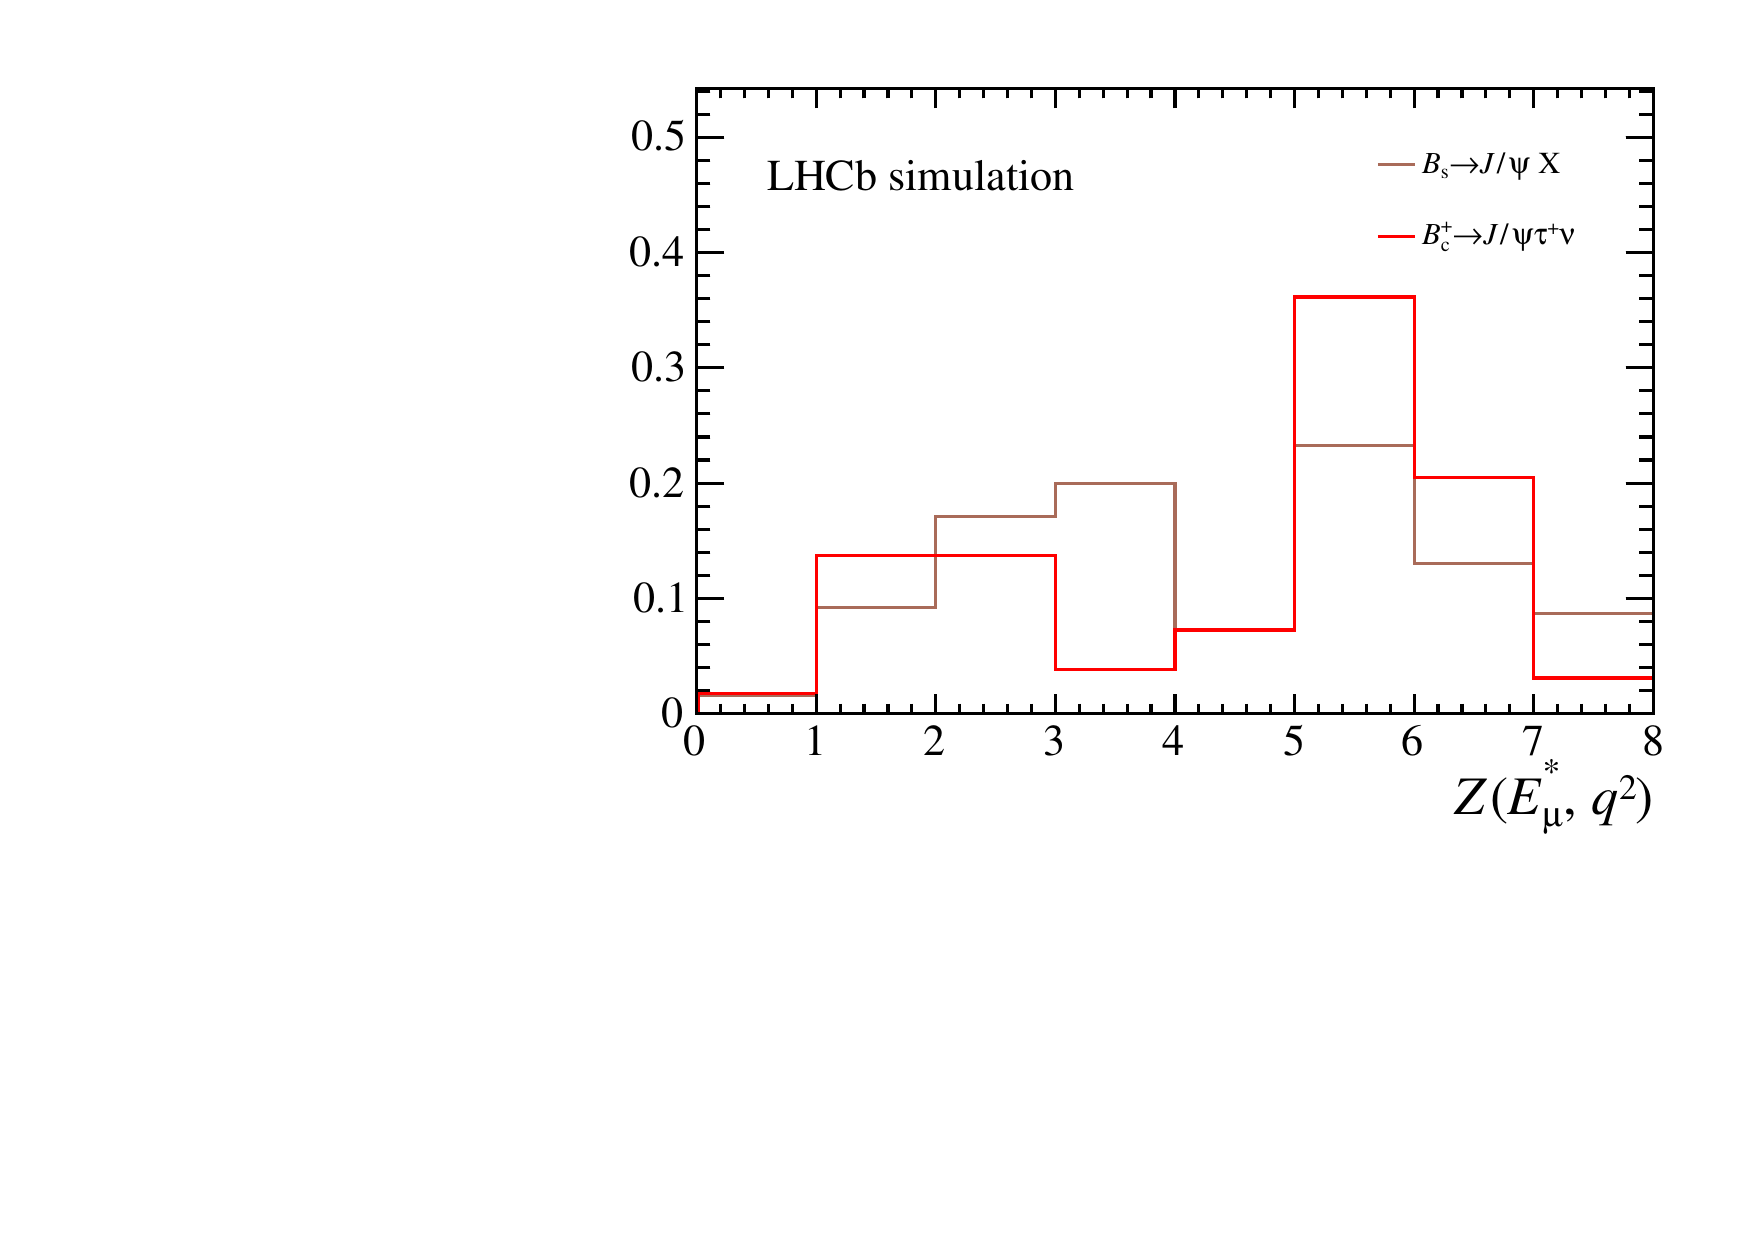}
    
    \caption{The distributions of rest-frame variables for the $B_{d,s} \to J/\psi X$ decays (brown) compared with the signal mode (red).}
    \label{fig:bds2jpsix_templates}
\end{figure}

\begin{figure}
\centering
    \includegraphics[width=0.3\textwidth]{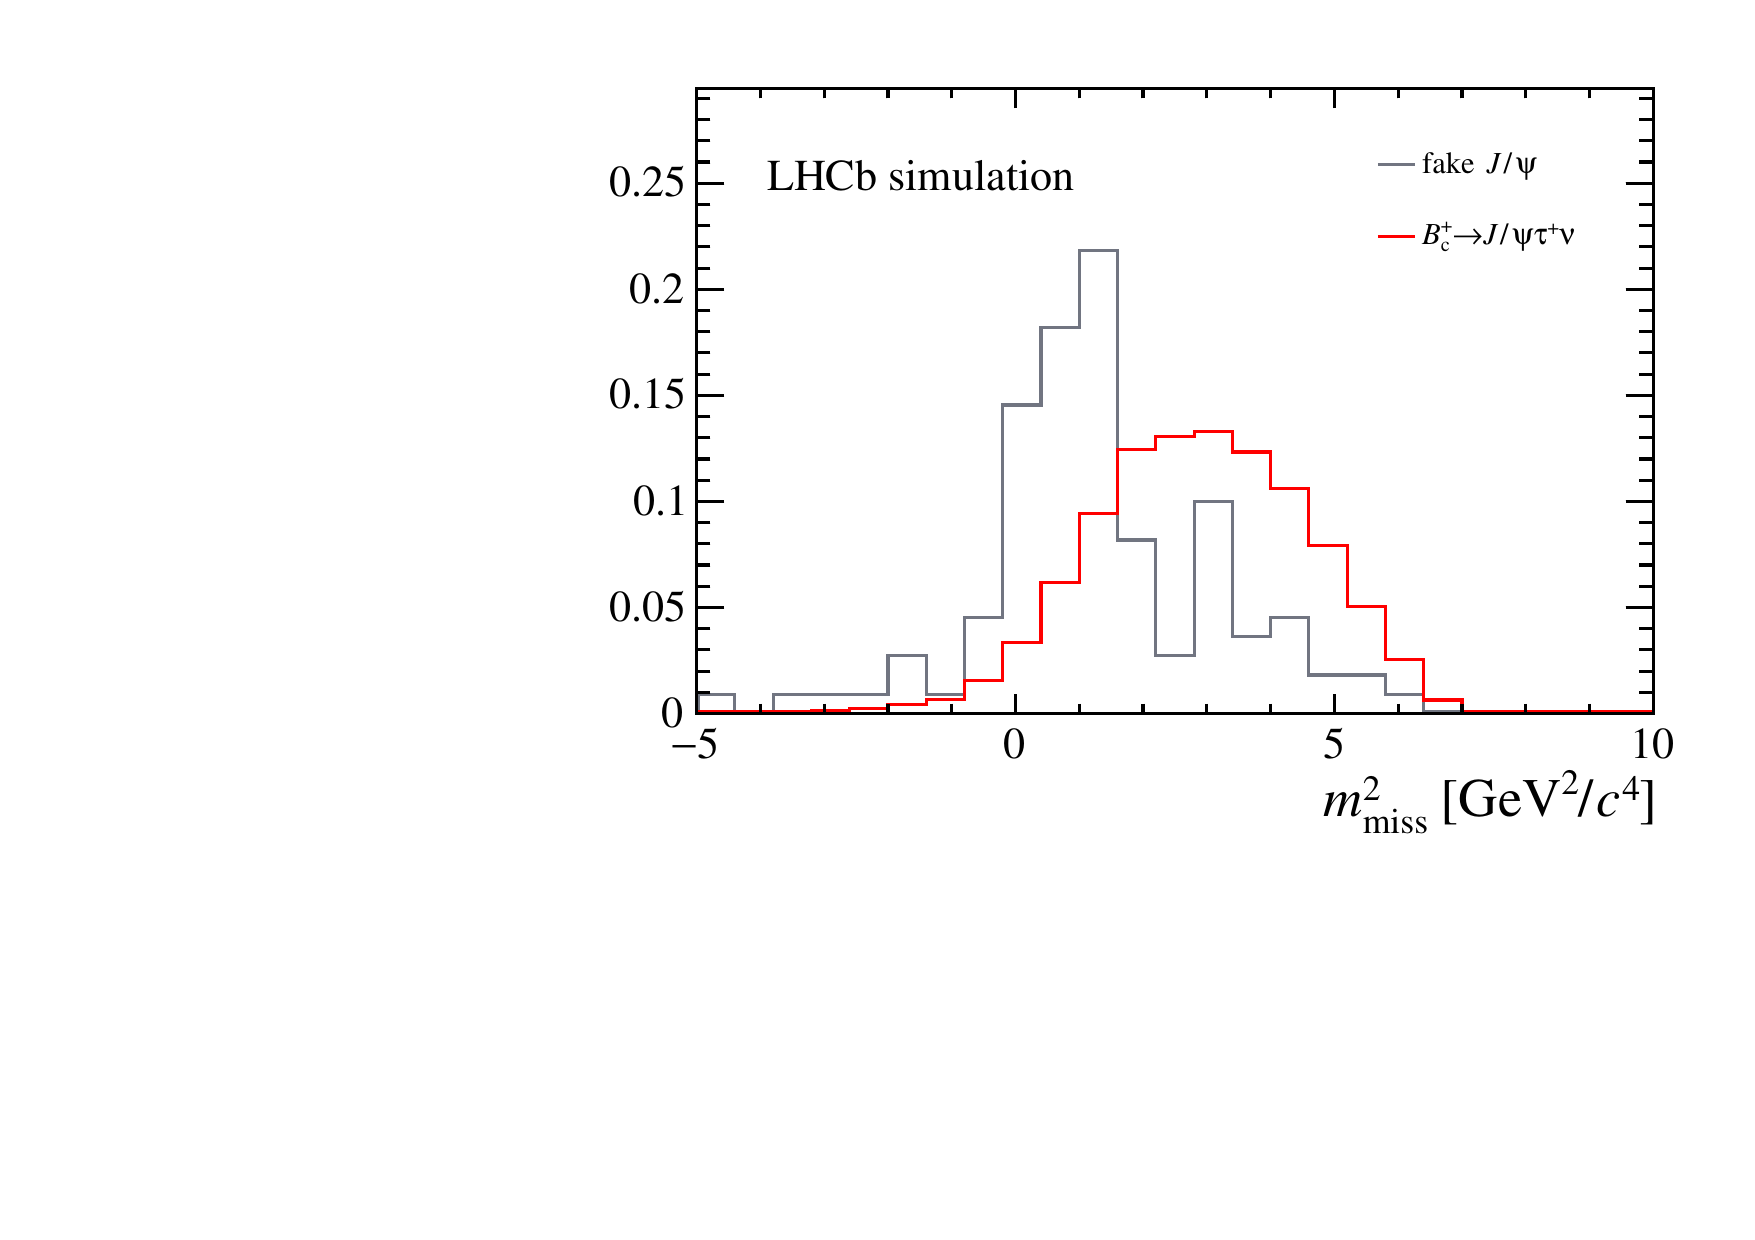}
    \includegraphics[width=0.3\textwidth]{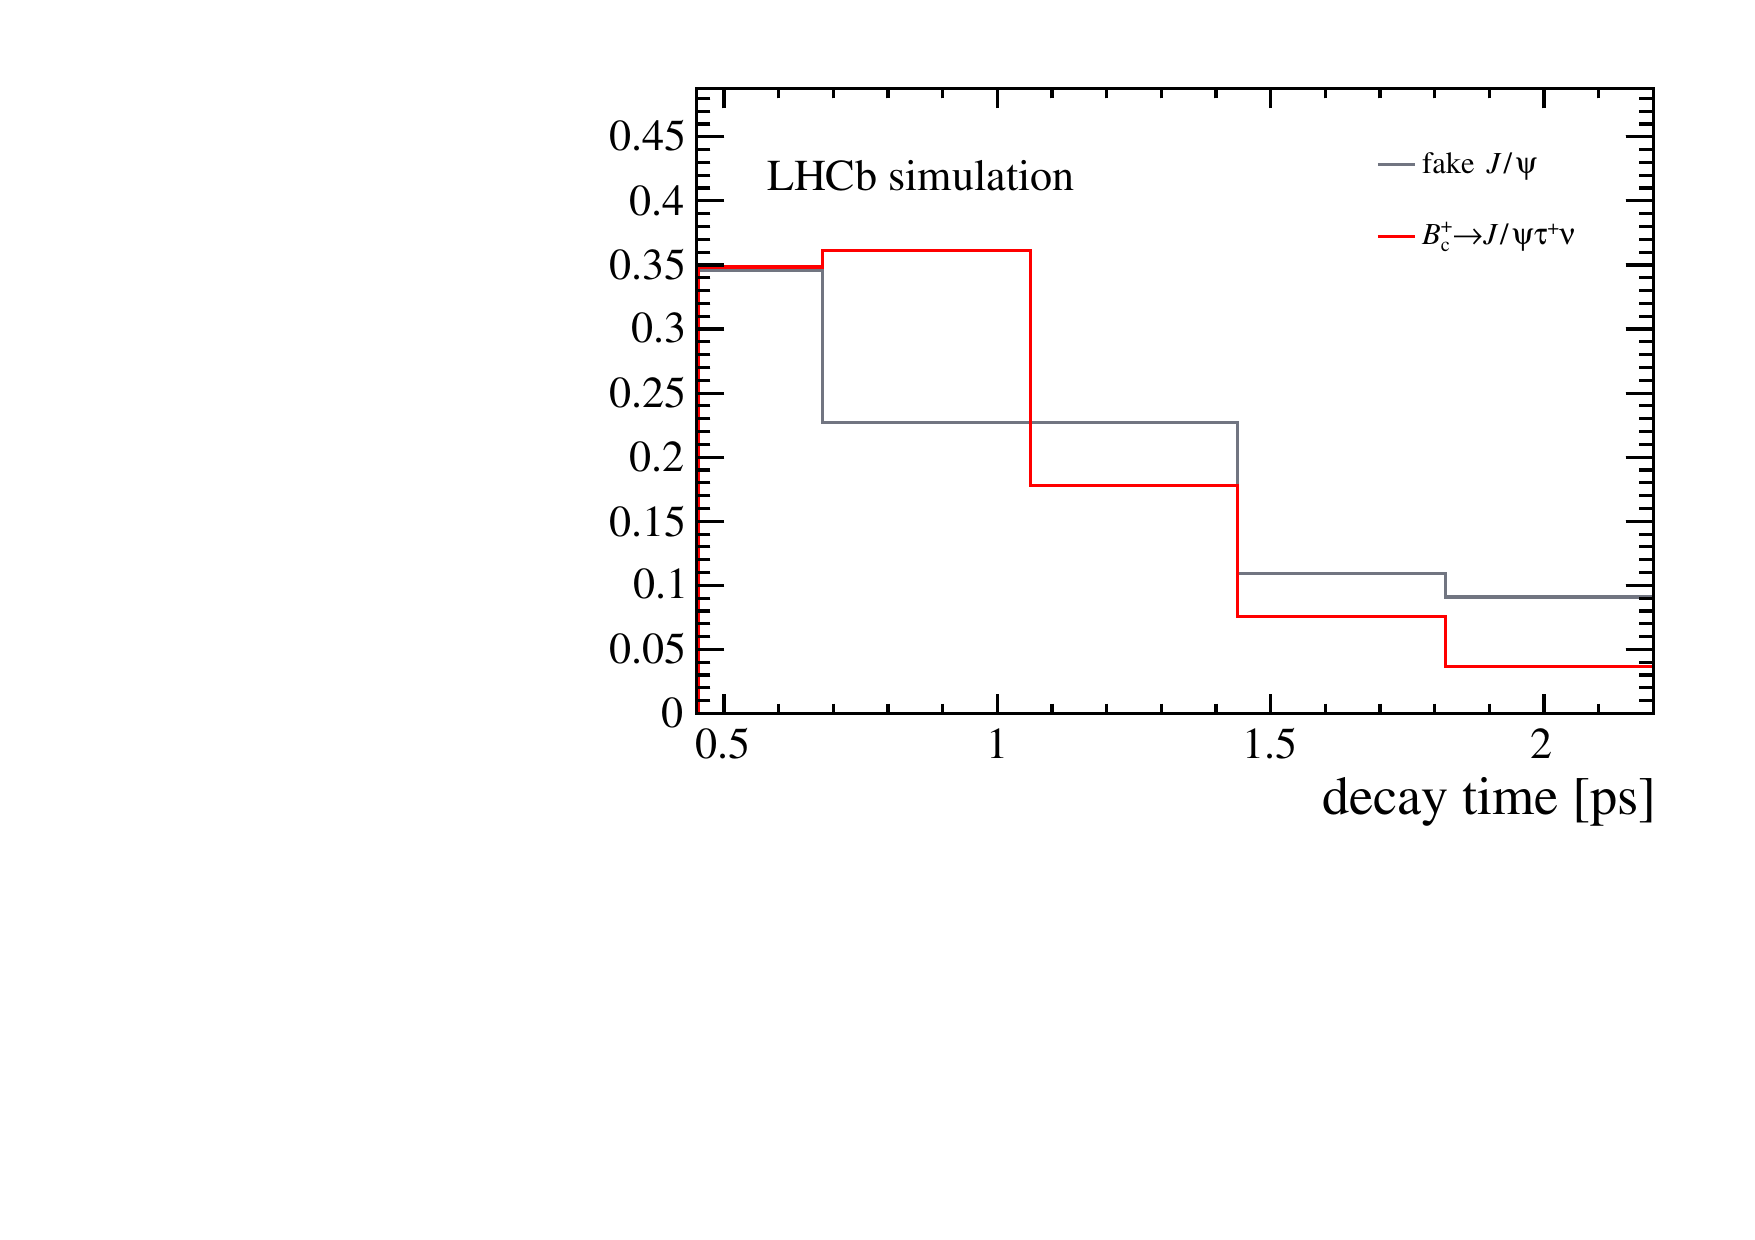}
    \includegraphics[width=0.3\textwidth]{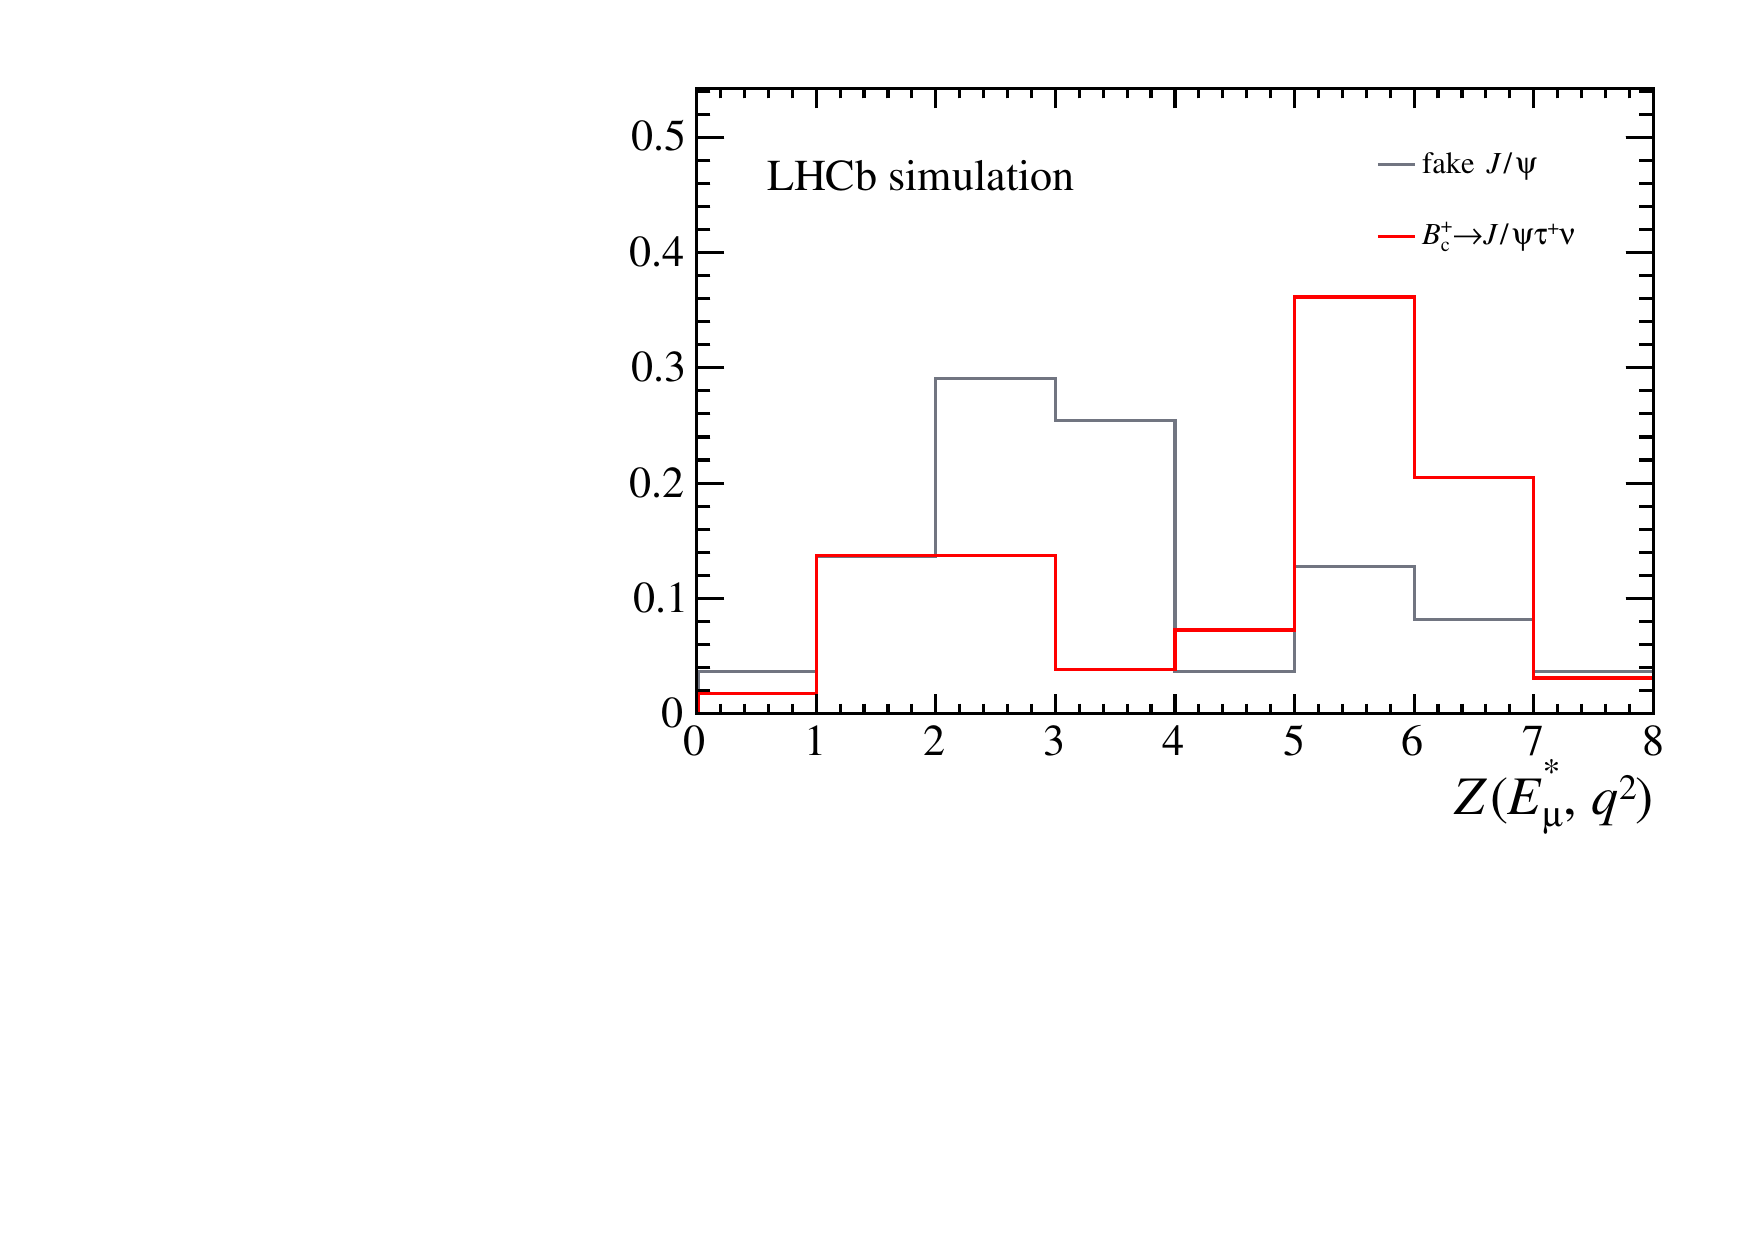}
    \caption{The distributions of rest-frame variables for the $(\mup \mun)\mup$ background (gray) compared with the signal mode (red).}
    \label{fig:fakejpsi_templates}
\end{figure}

\begin{figure}
\centering
    \includegraphics[width=0.3\textwidth]{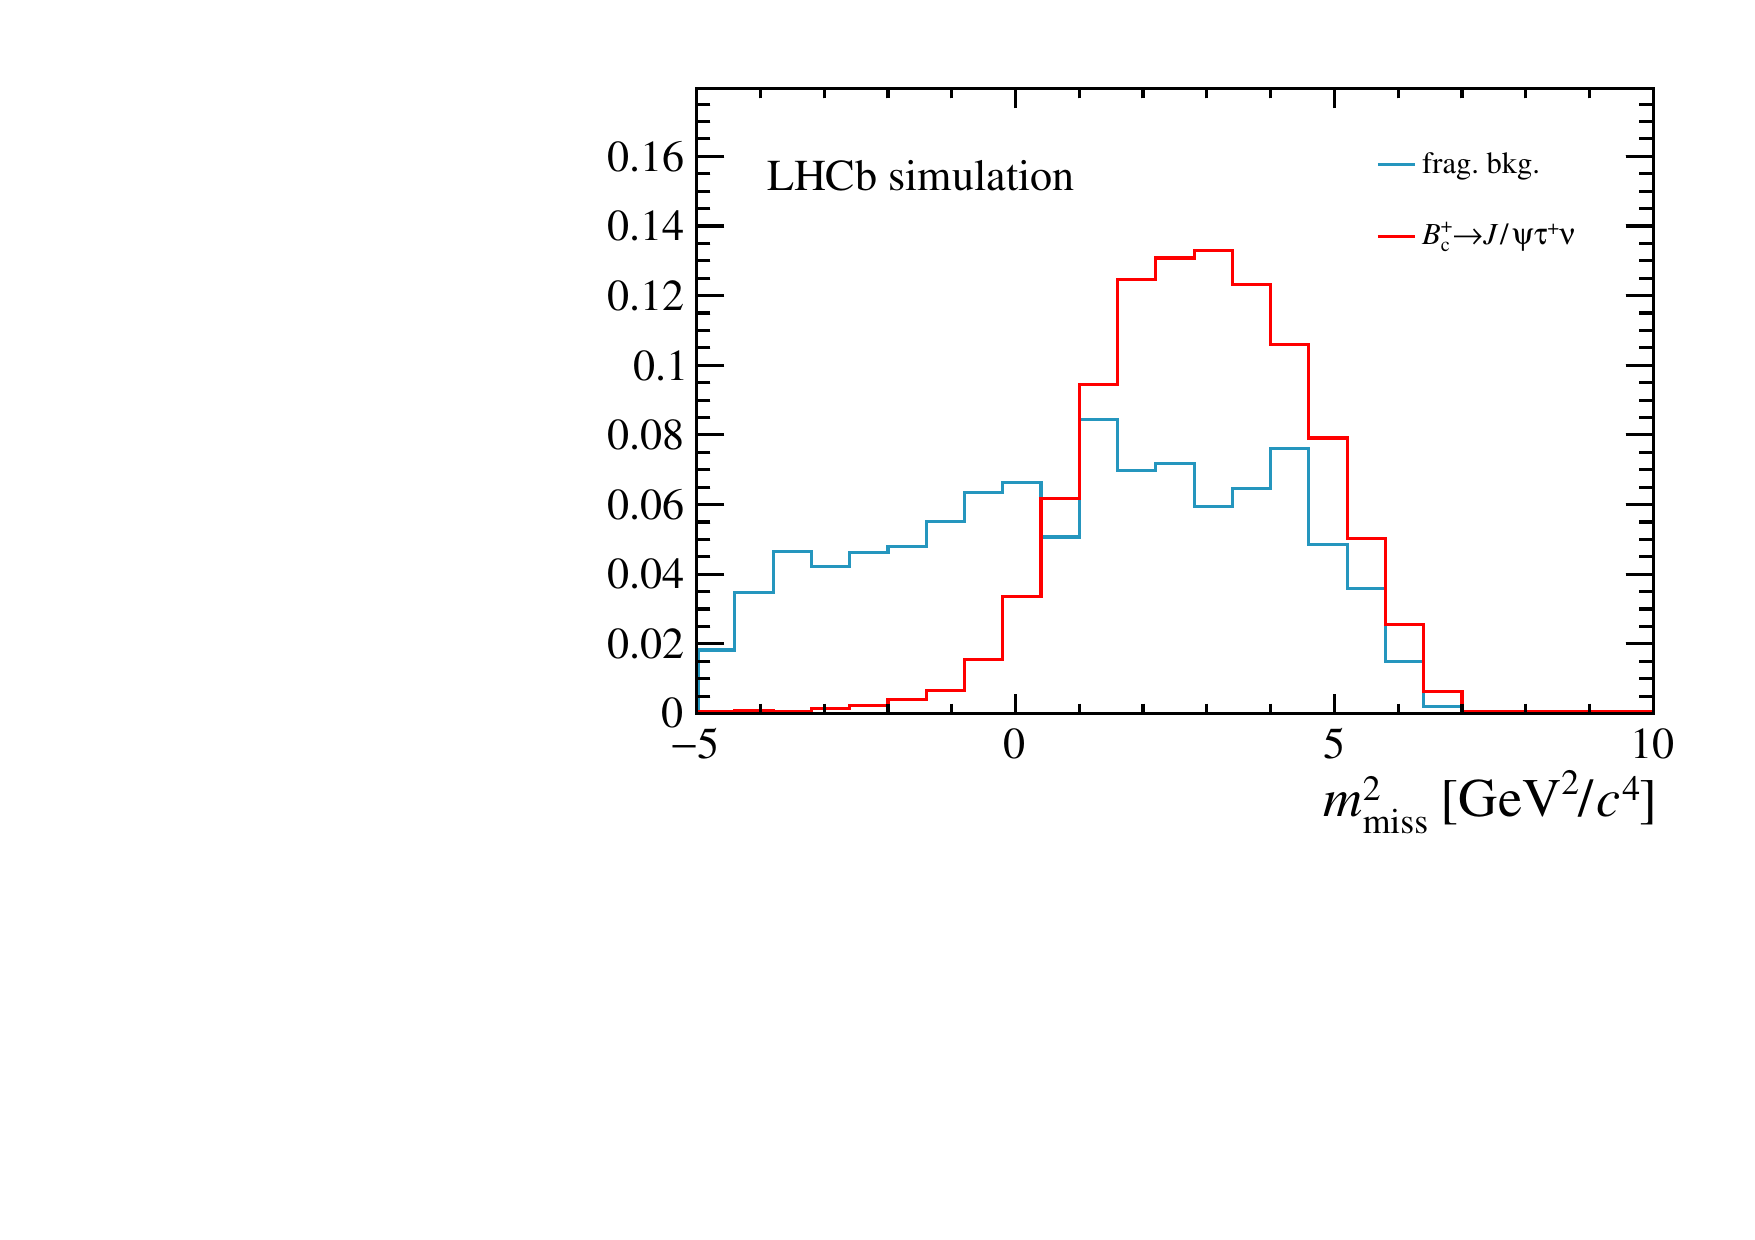}
    \includegraphics[width=0.3\textwidth]{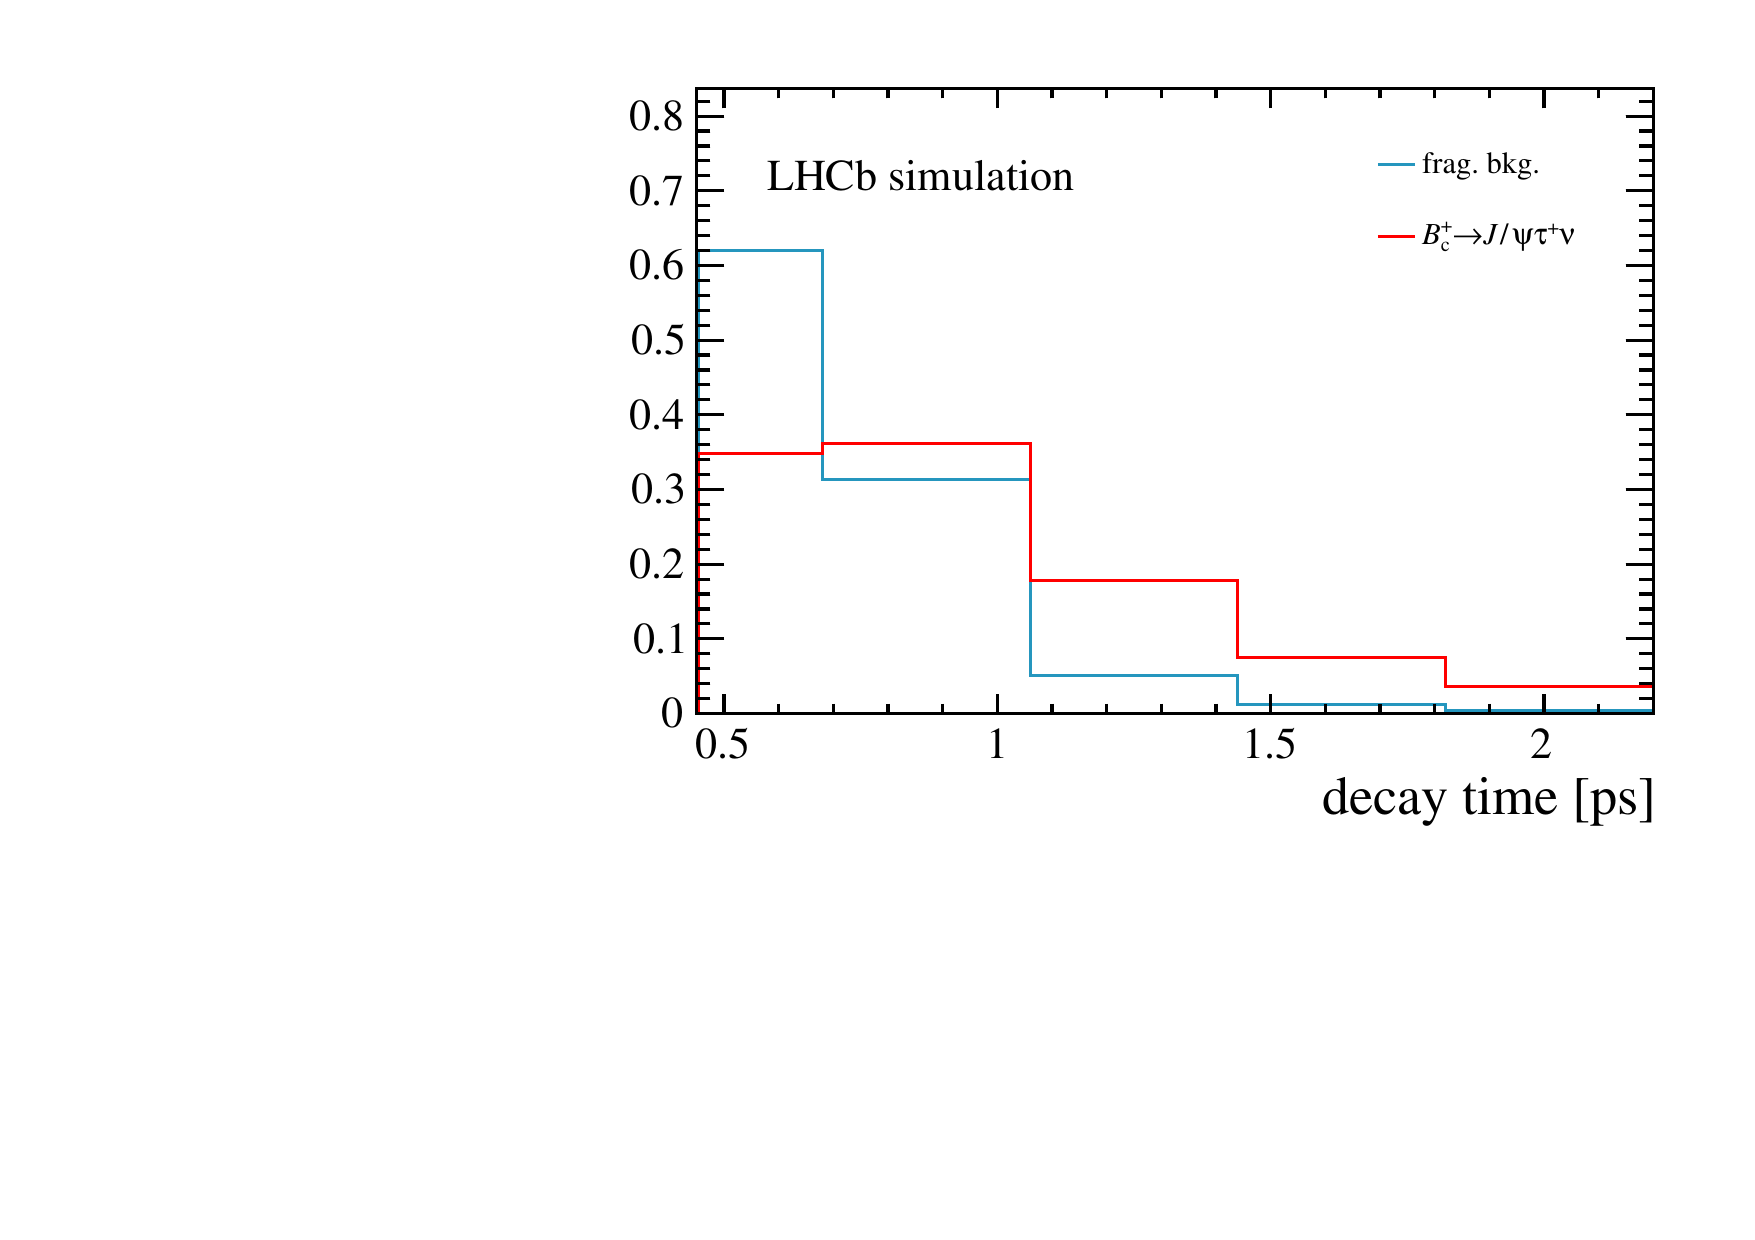}
    \includegraphics[width=0.3\textwidth]{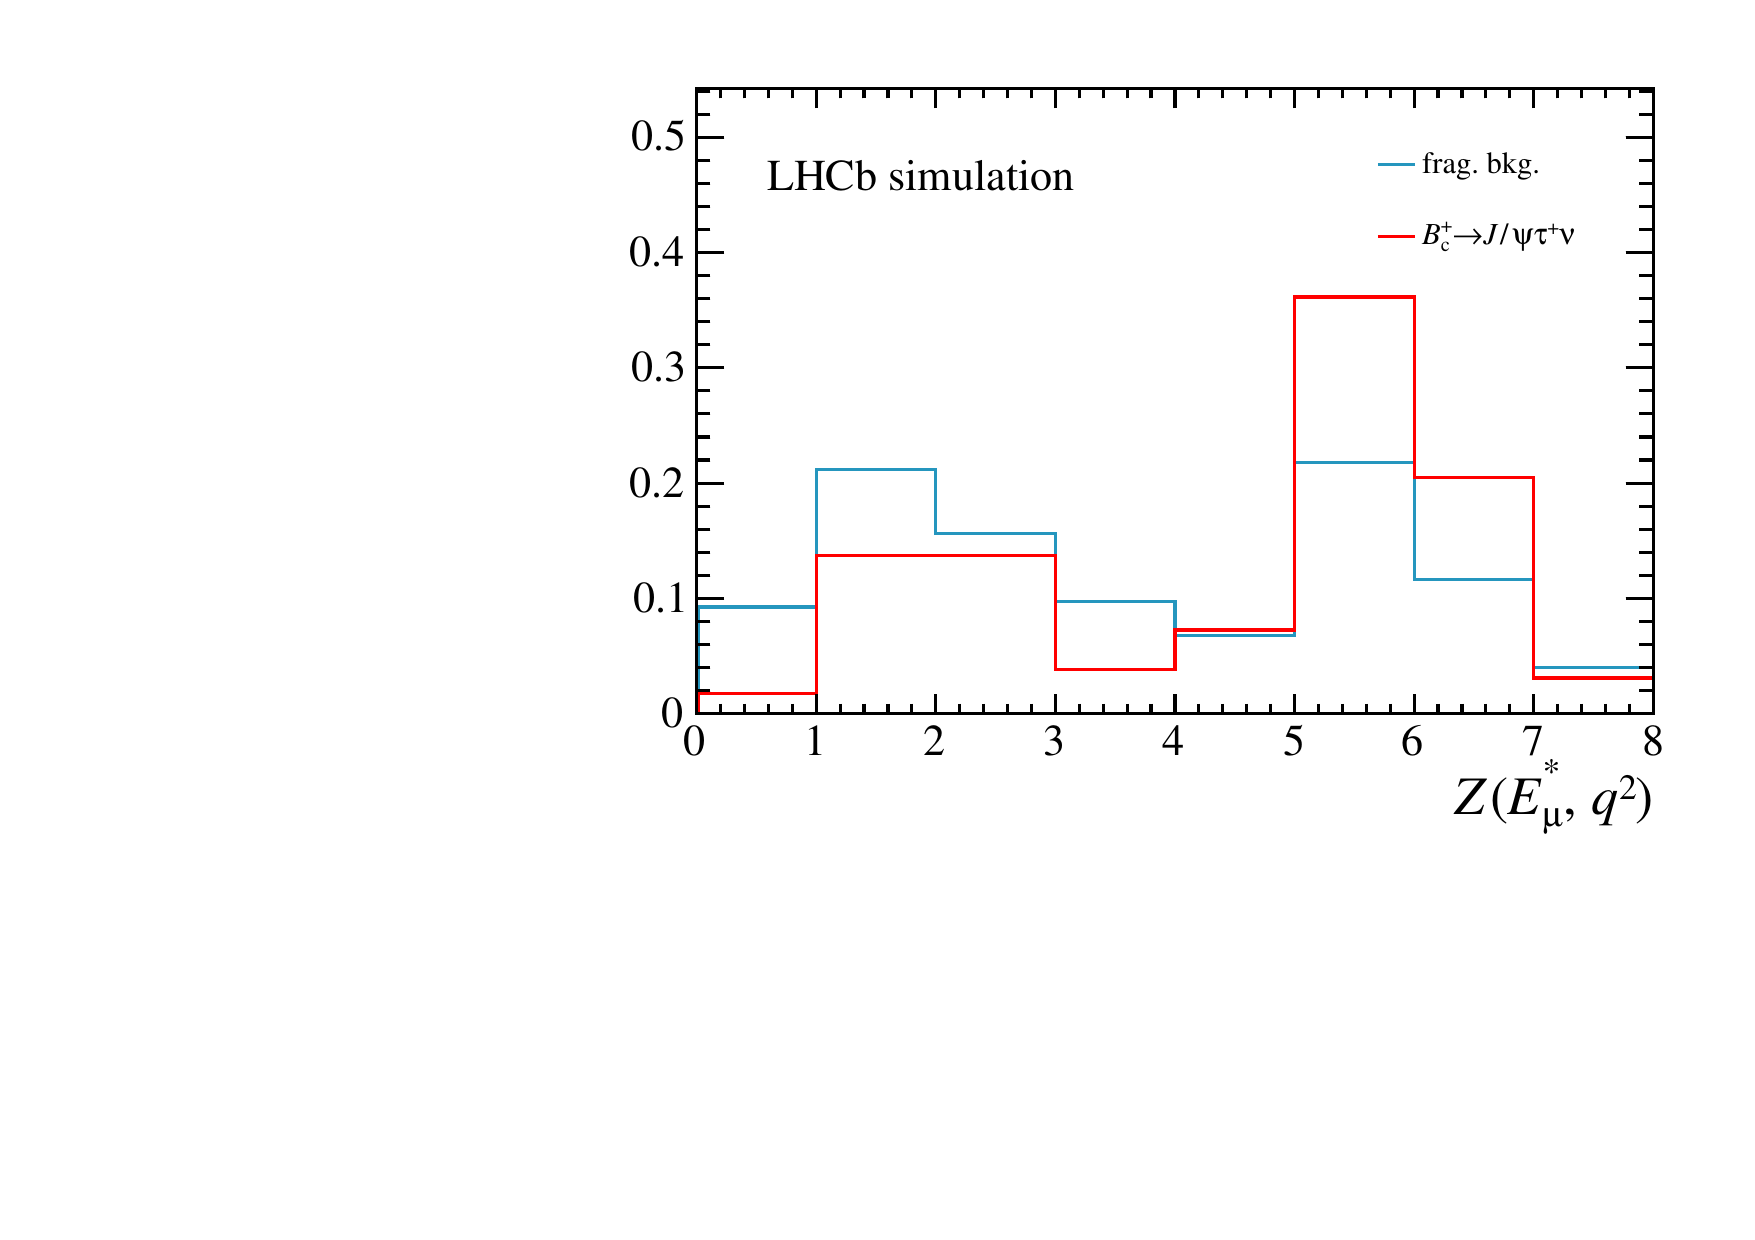}
    \caption{The distributions of rest-frame variables for the fragmentation background (cyan) compared with the signal mode (red).}
    \label{fig:ccomb_templates}
\end{figure}

\begin{figure}
\centering
    \includegraphics[width=0.3\textwidth]{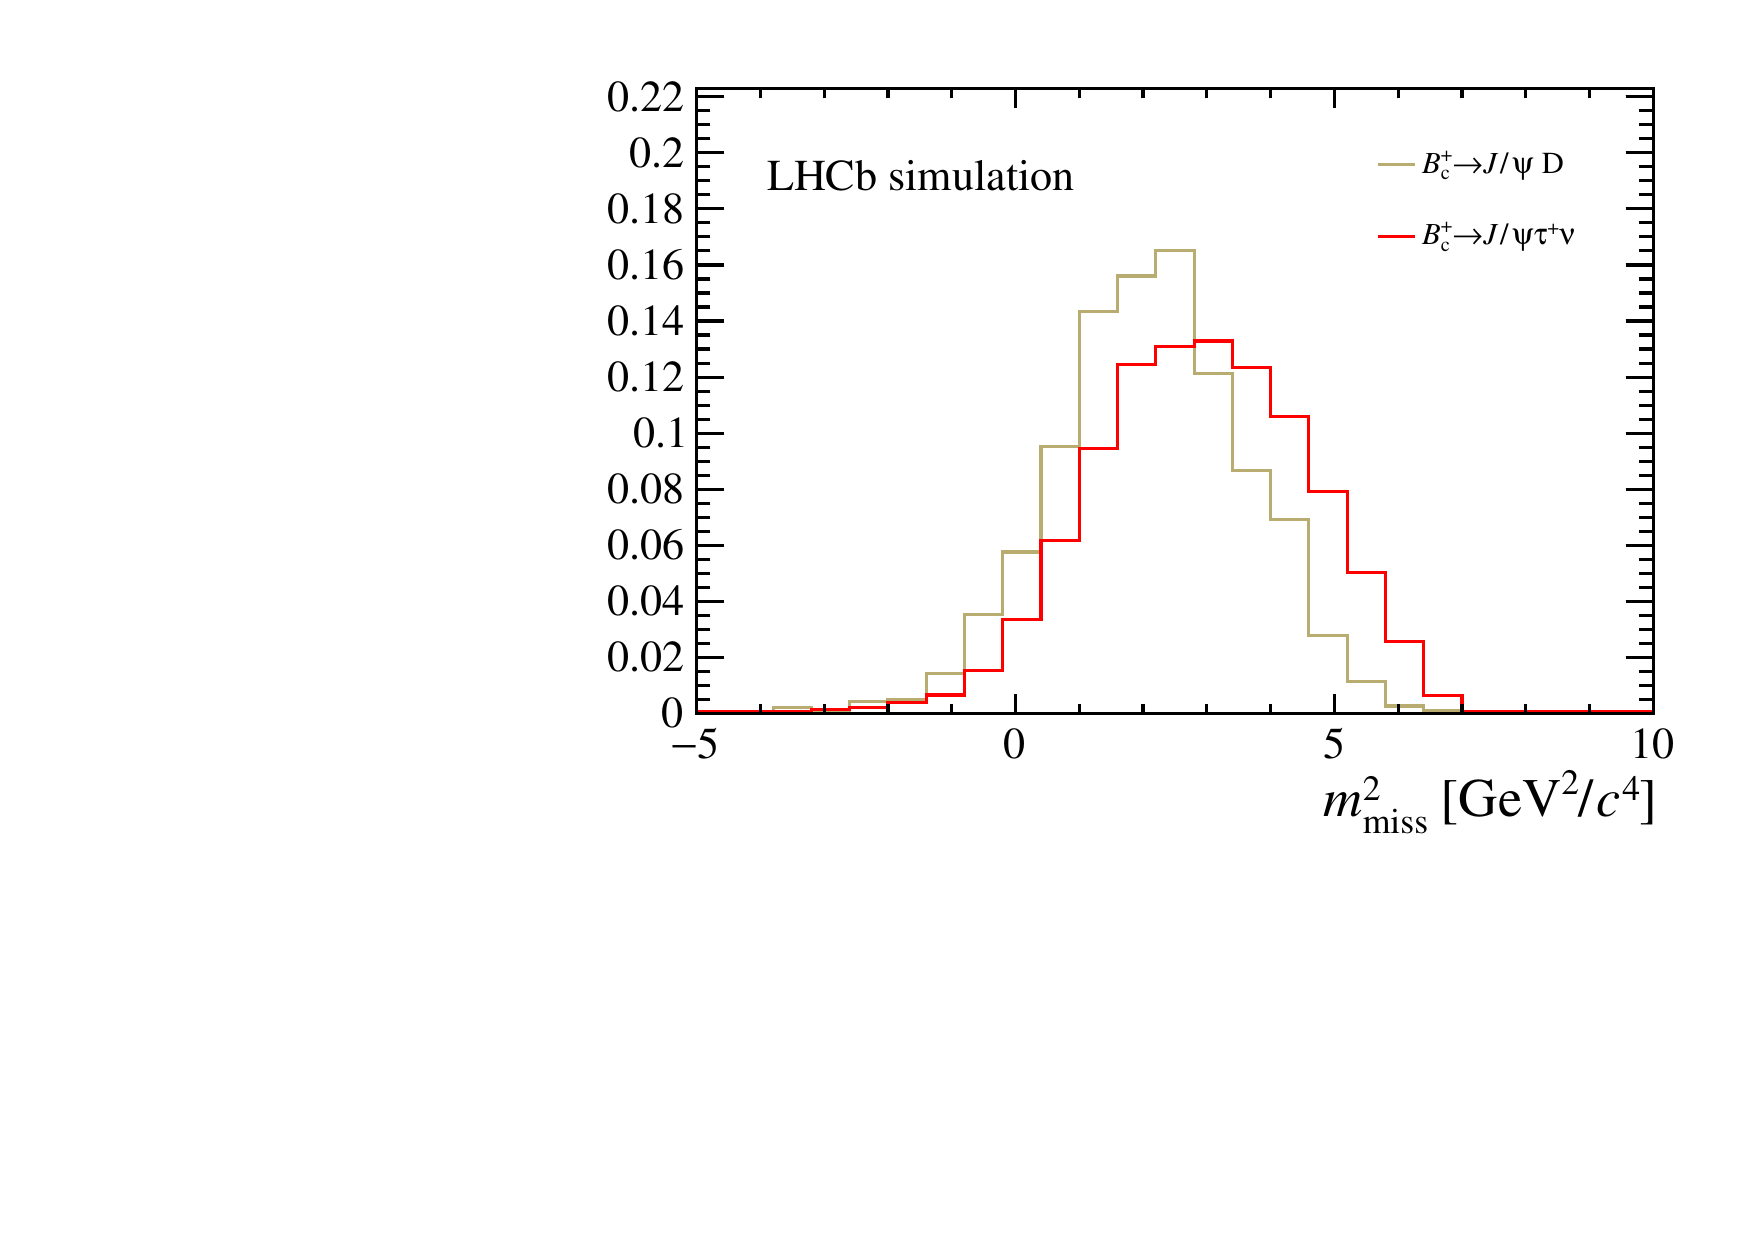}
    \includegraphics[width=0.3\textwidth]{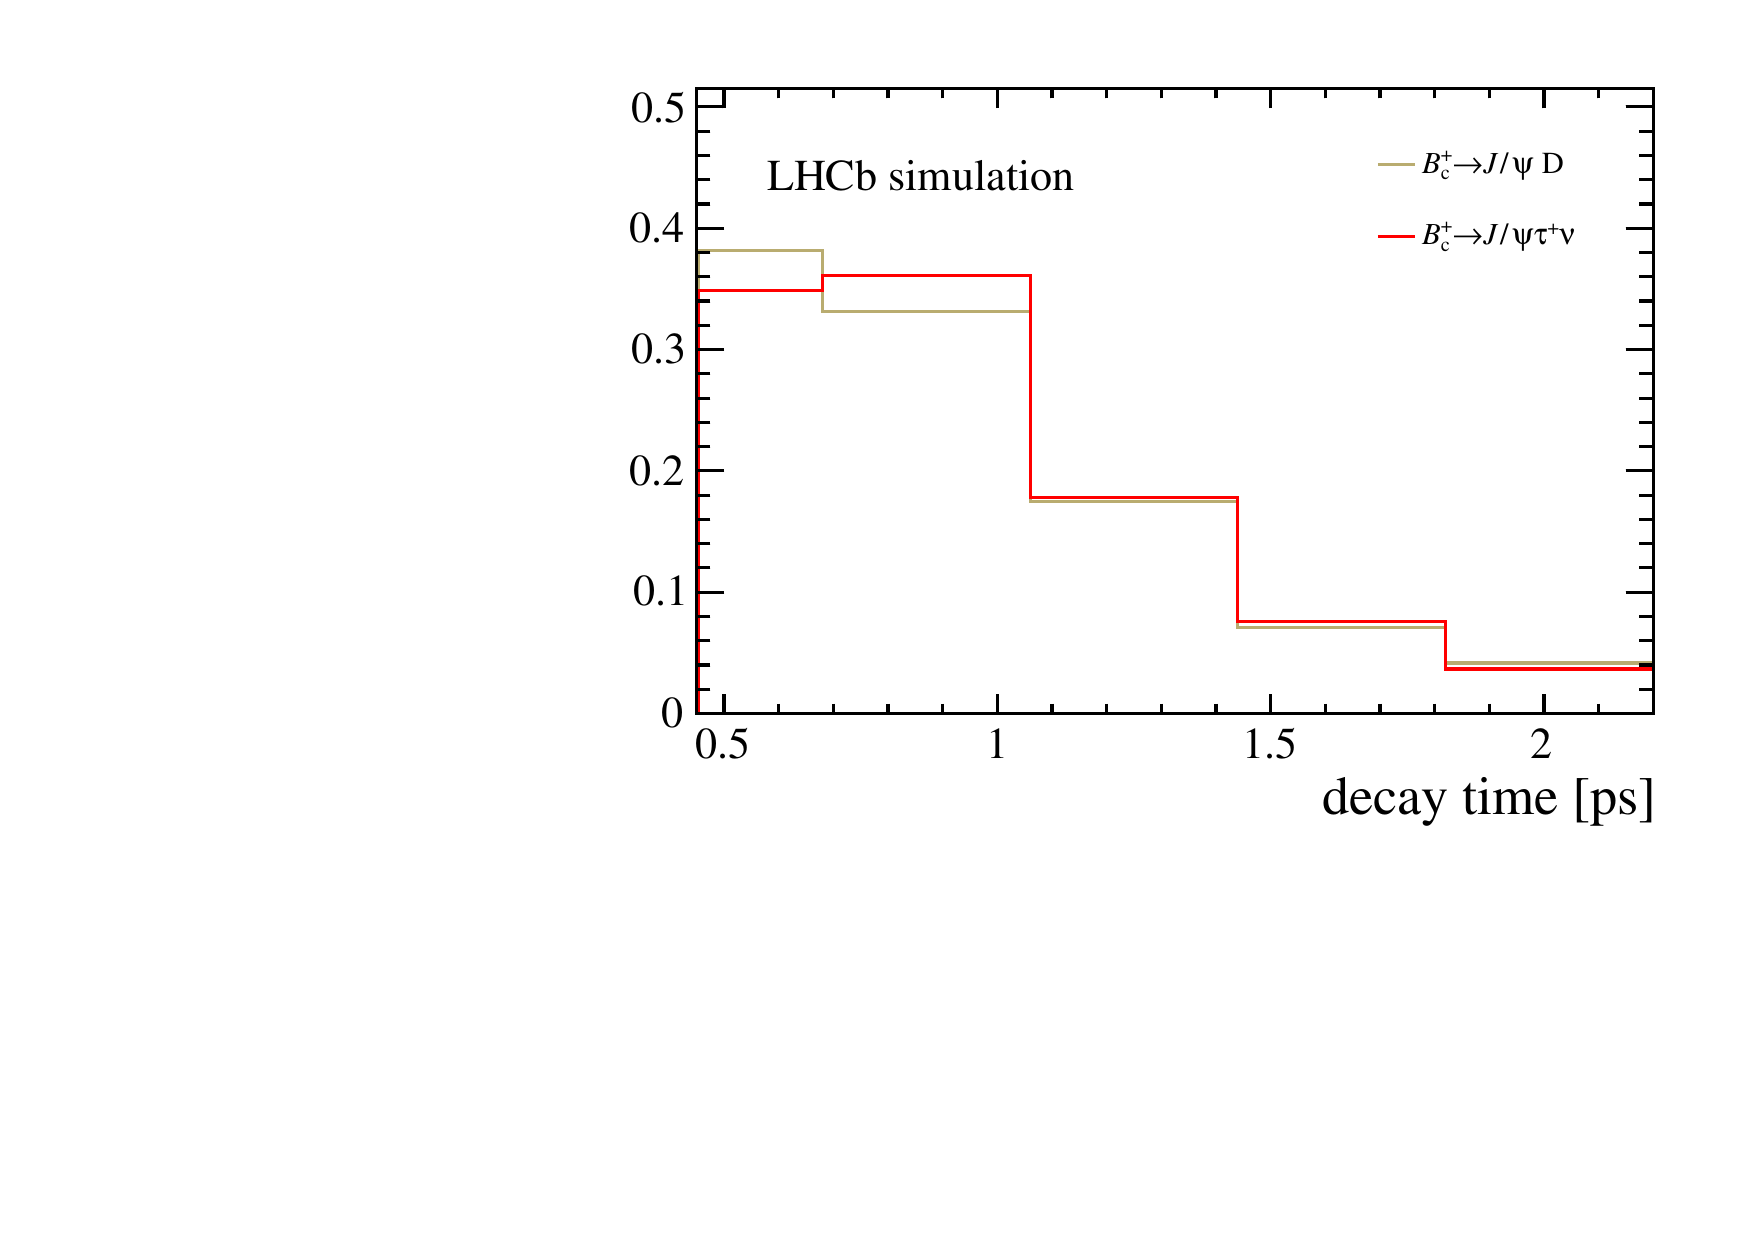}
    \includegraphics[width=0.3\textwidth]{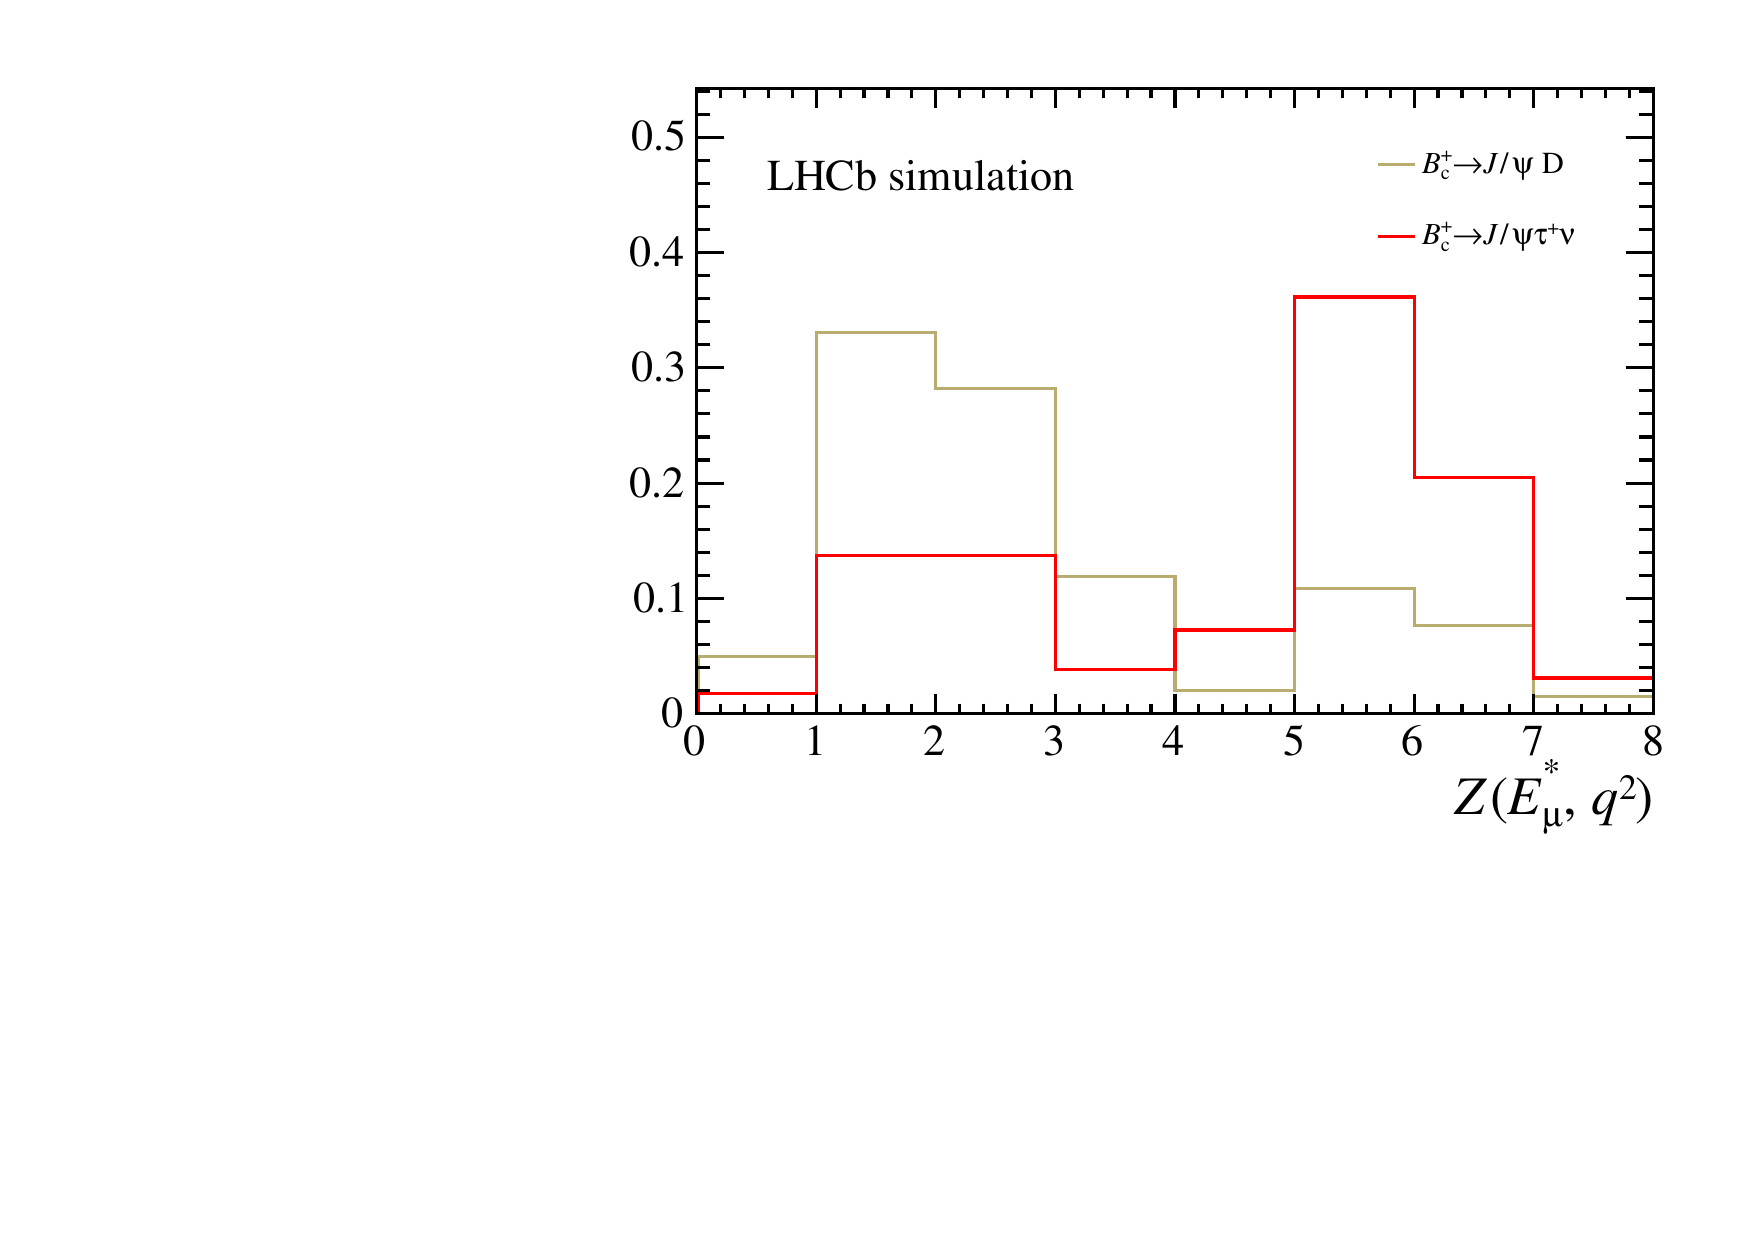}
    \includegraphics[width=0.3\textwidth]{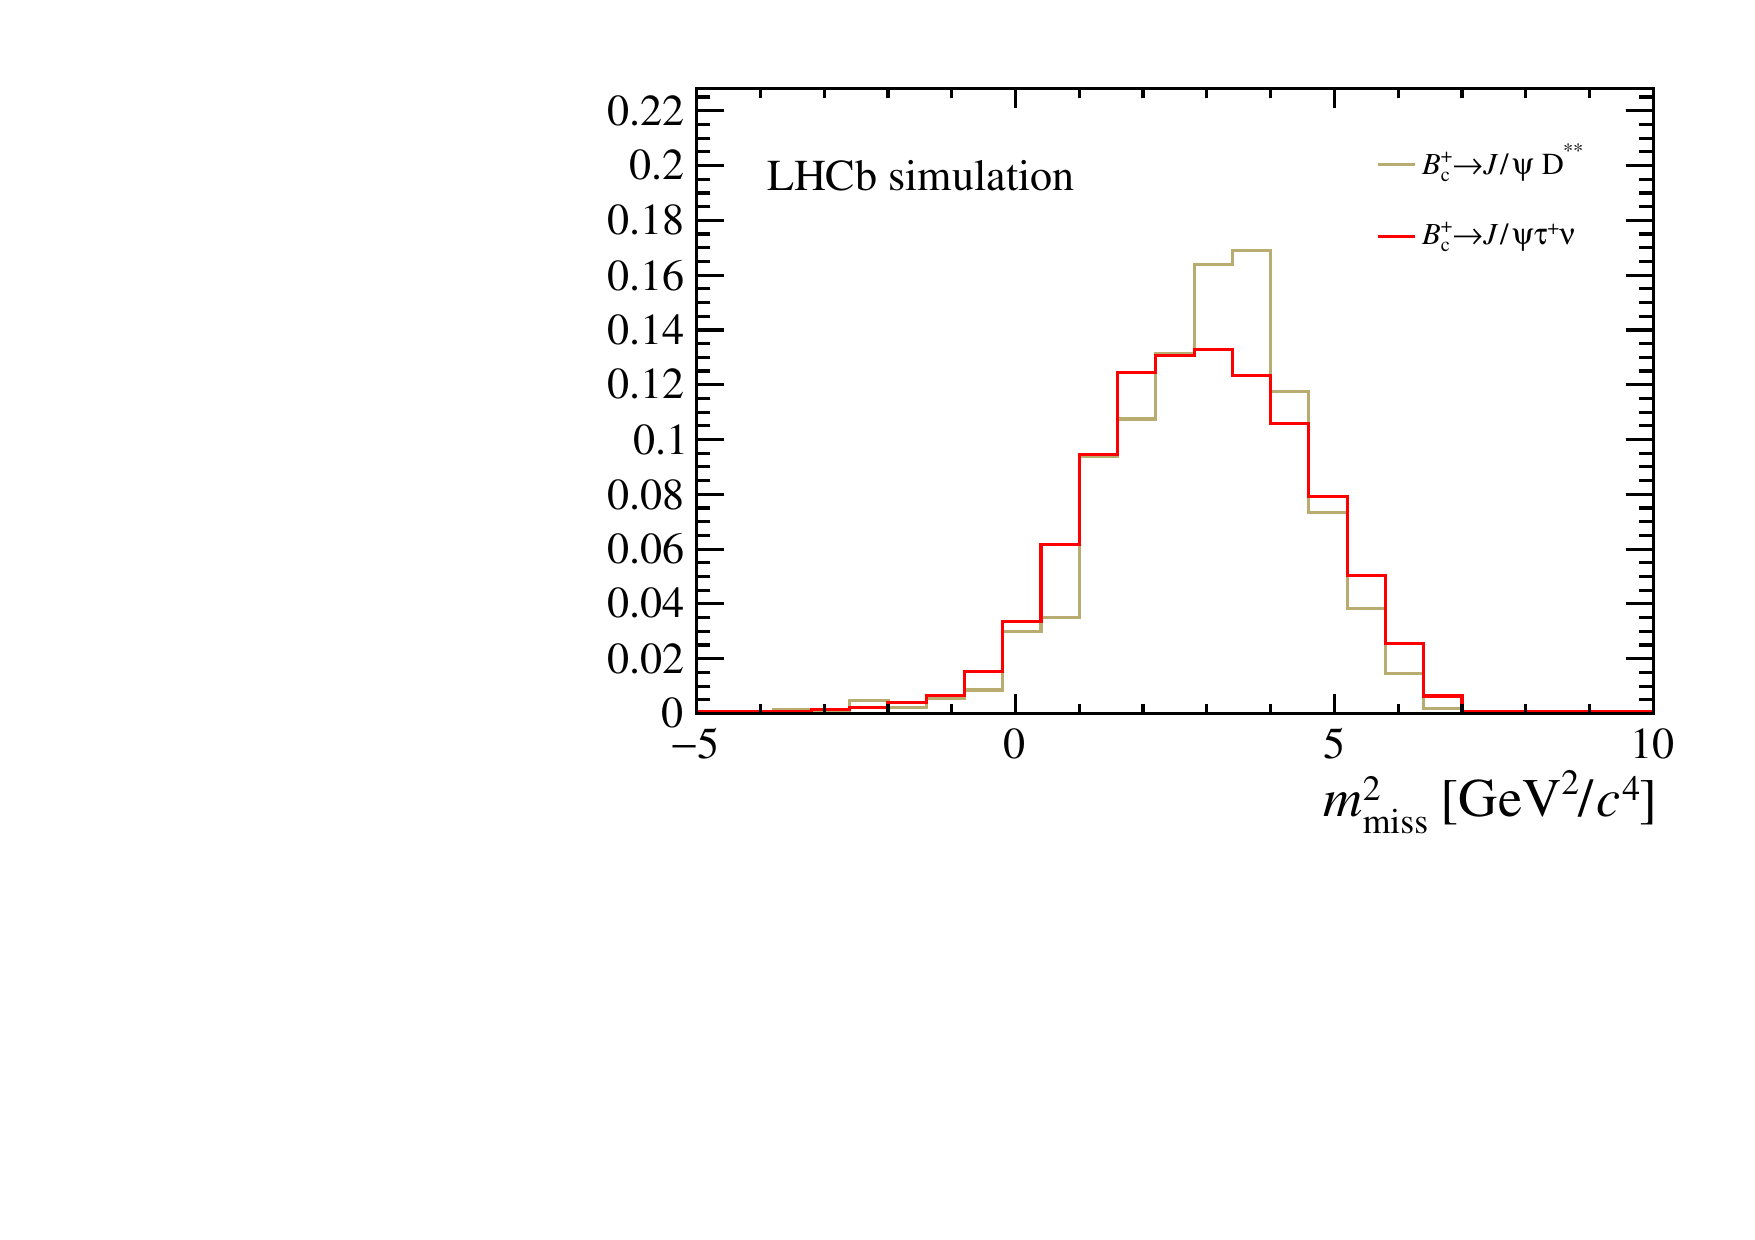}
    \includegraphics[width=0.3\textwidth]{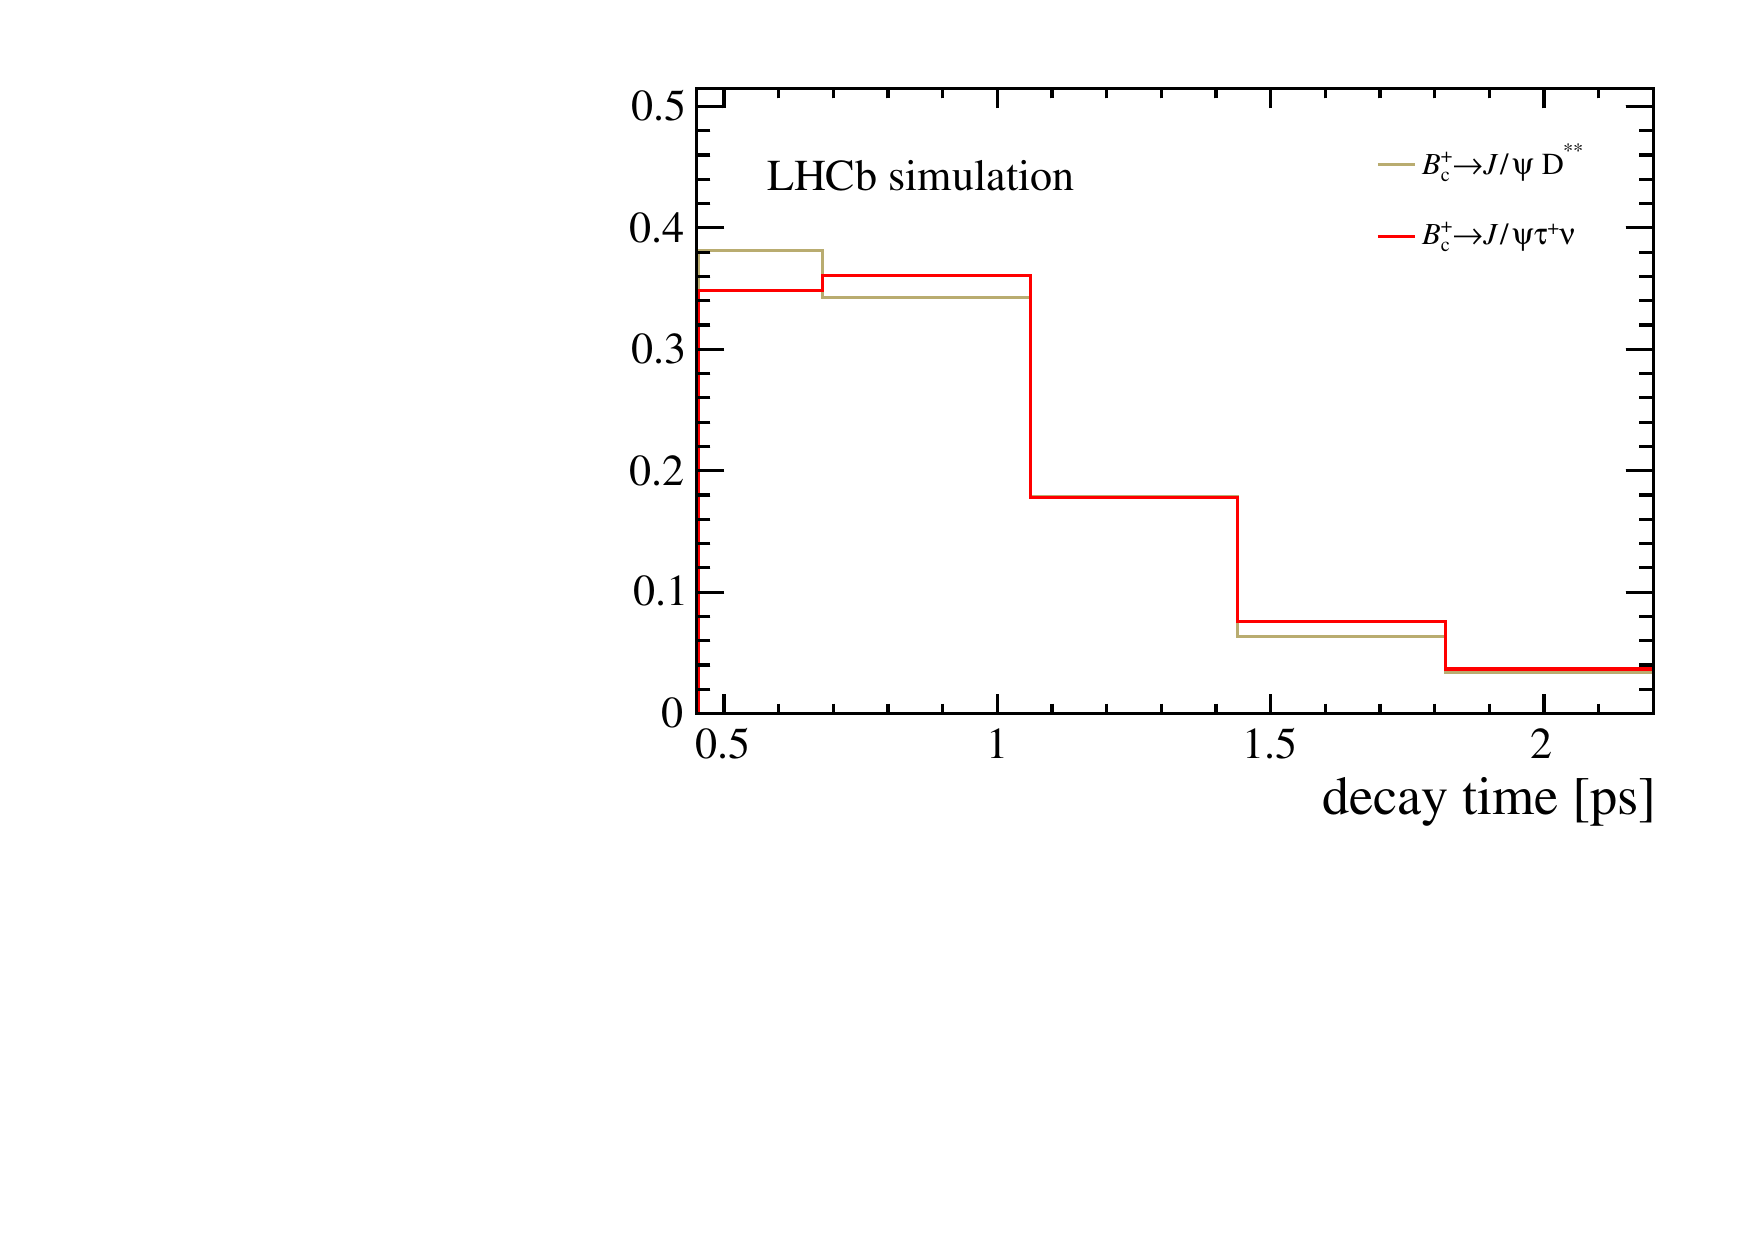}
    \includegraphics[width=0.3\textwidth]{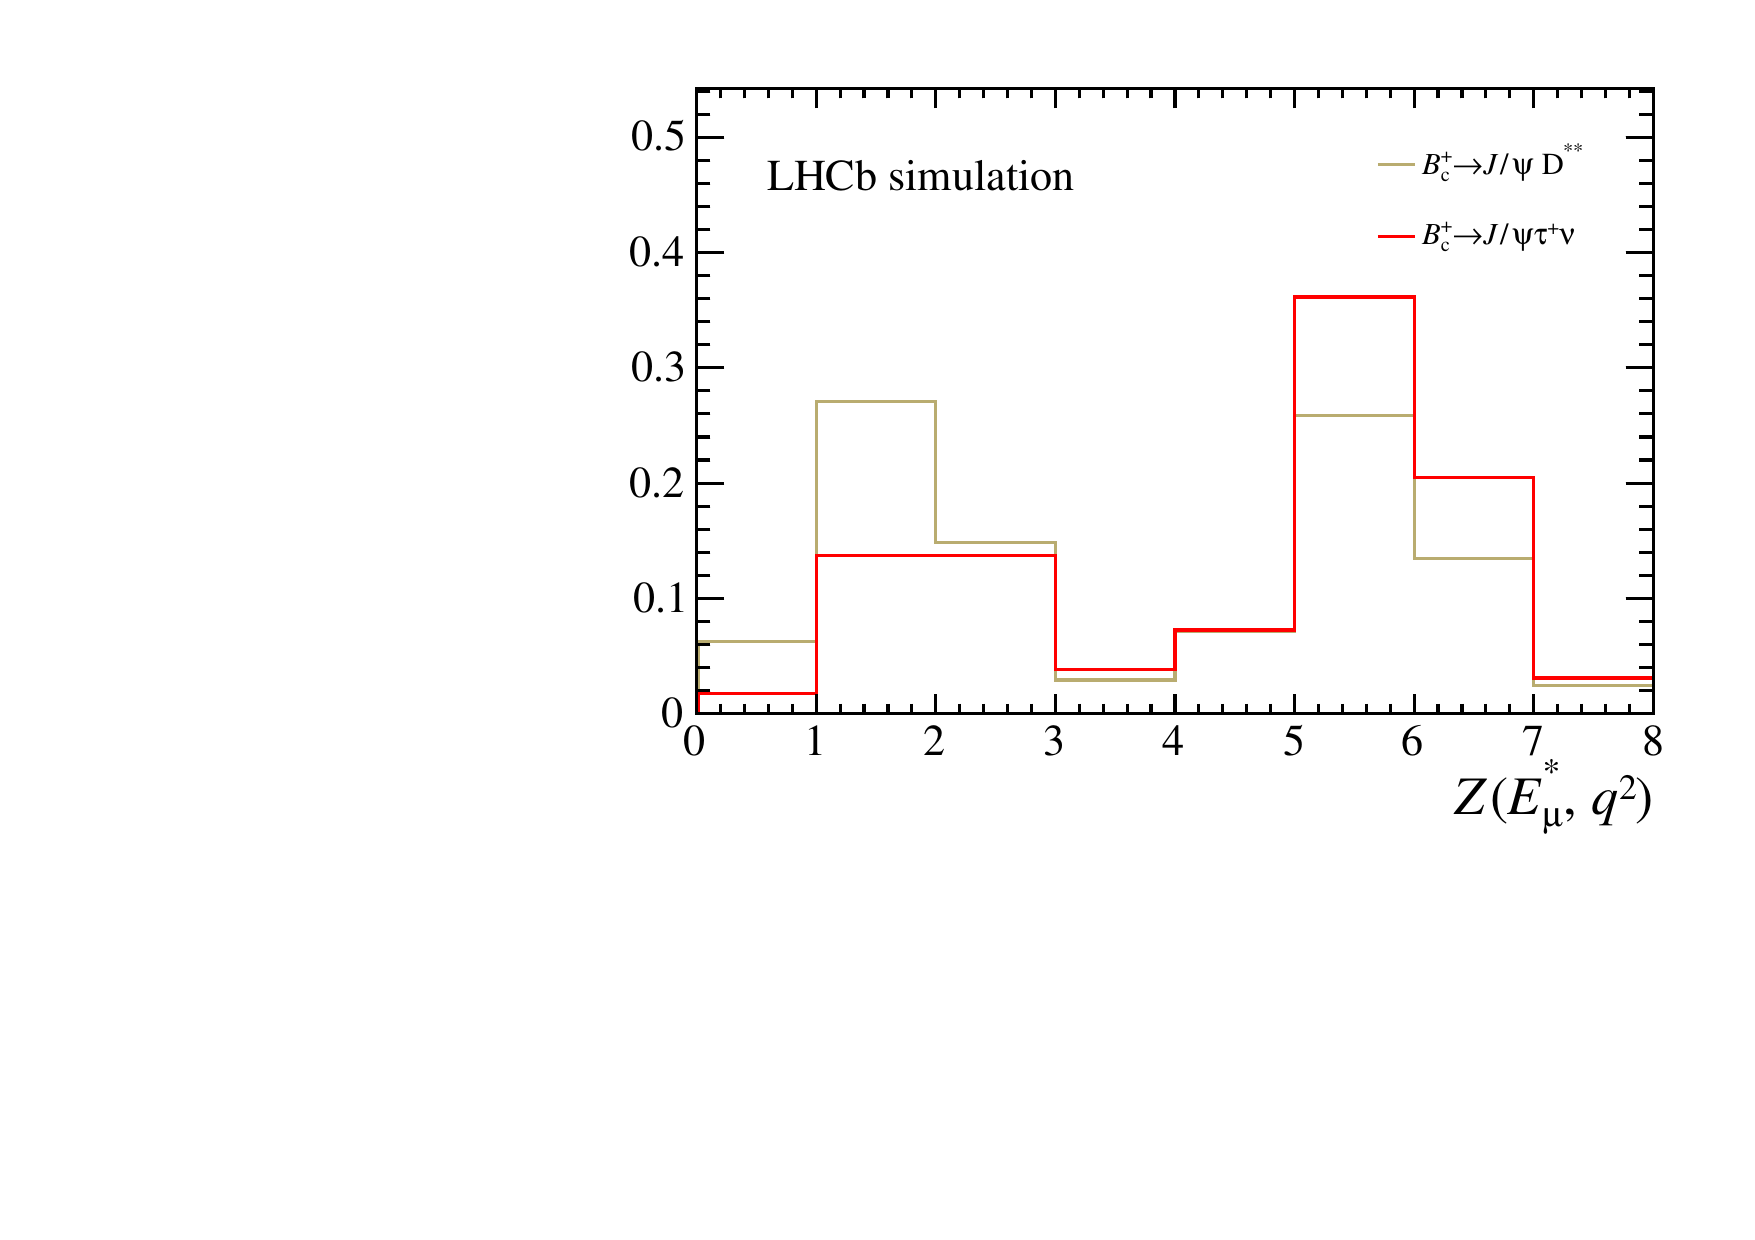}
    \includegraphics[width=0.3\textwidth]{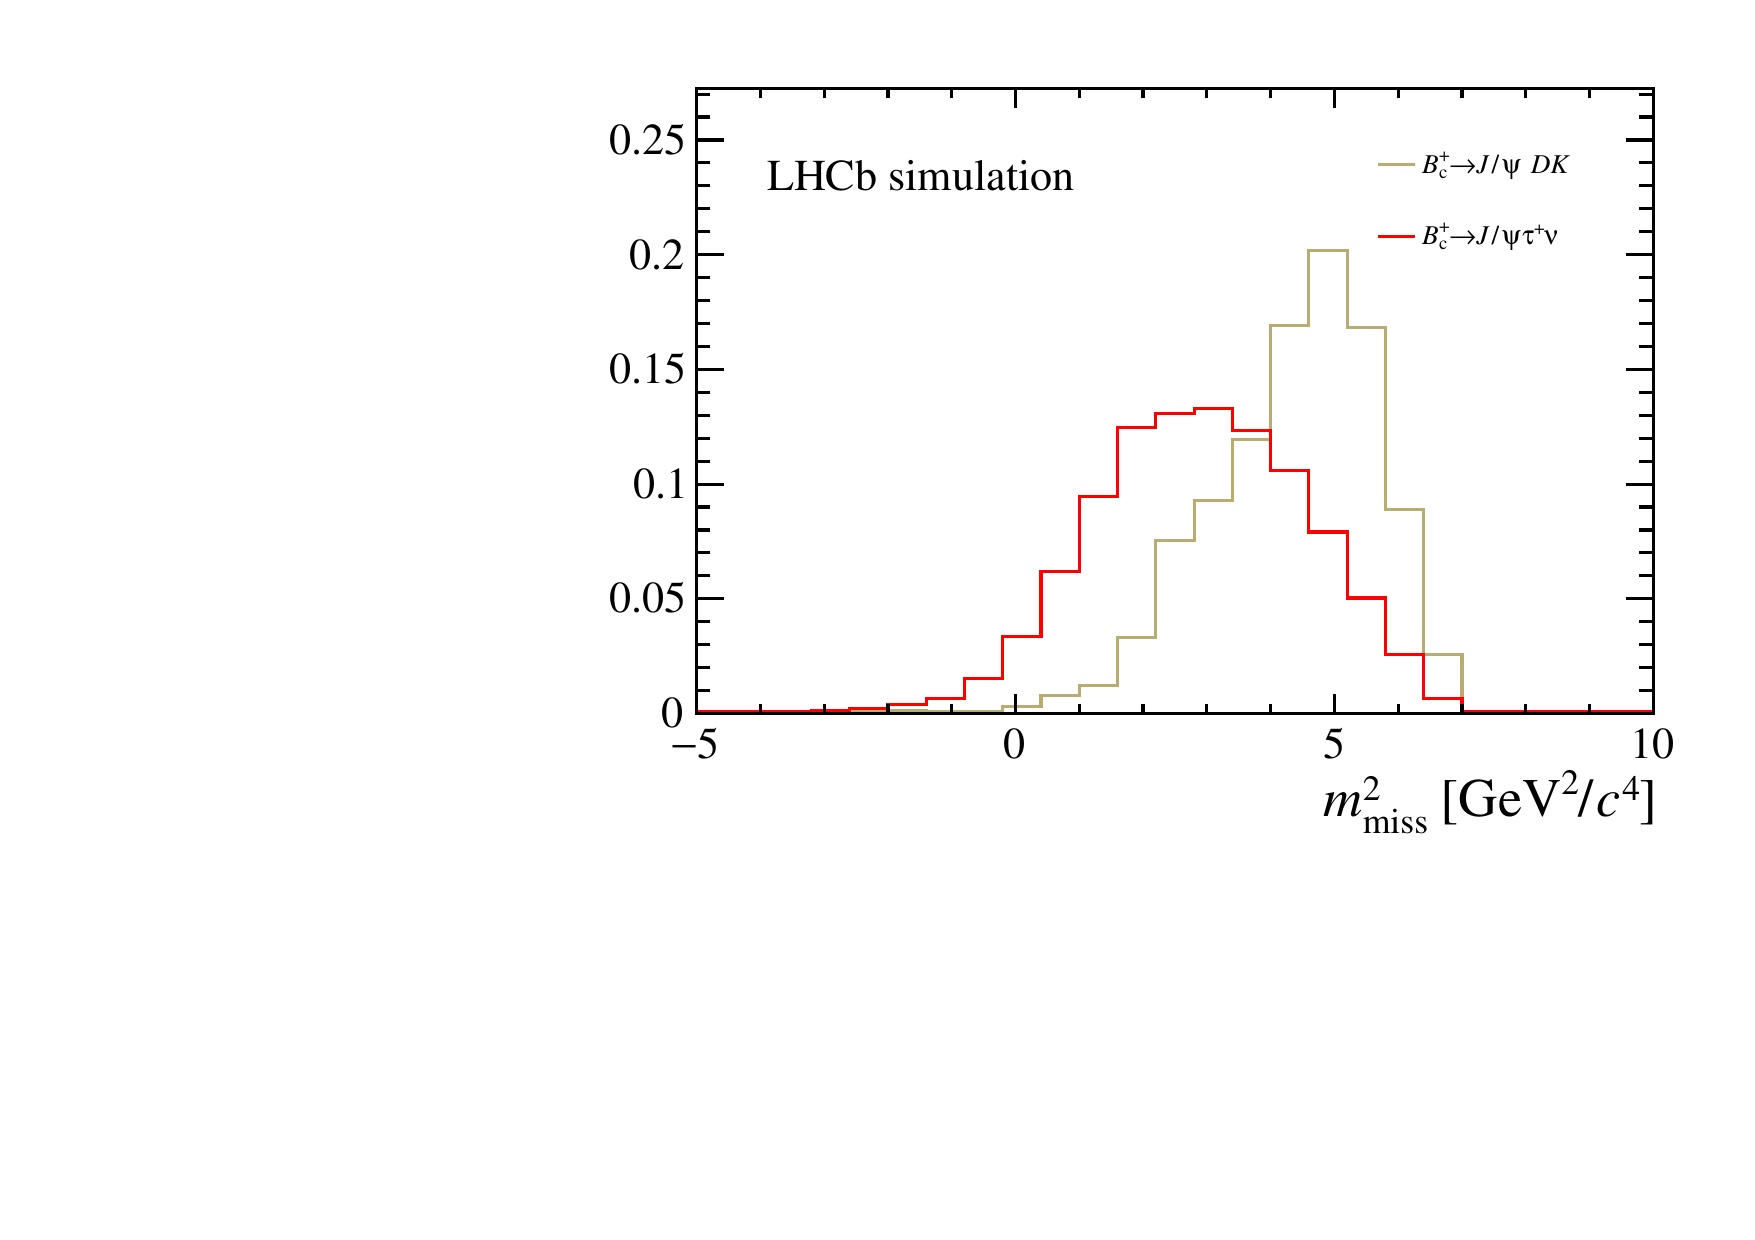}
    \includegraphics[width=0.3\textwidth]{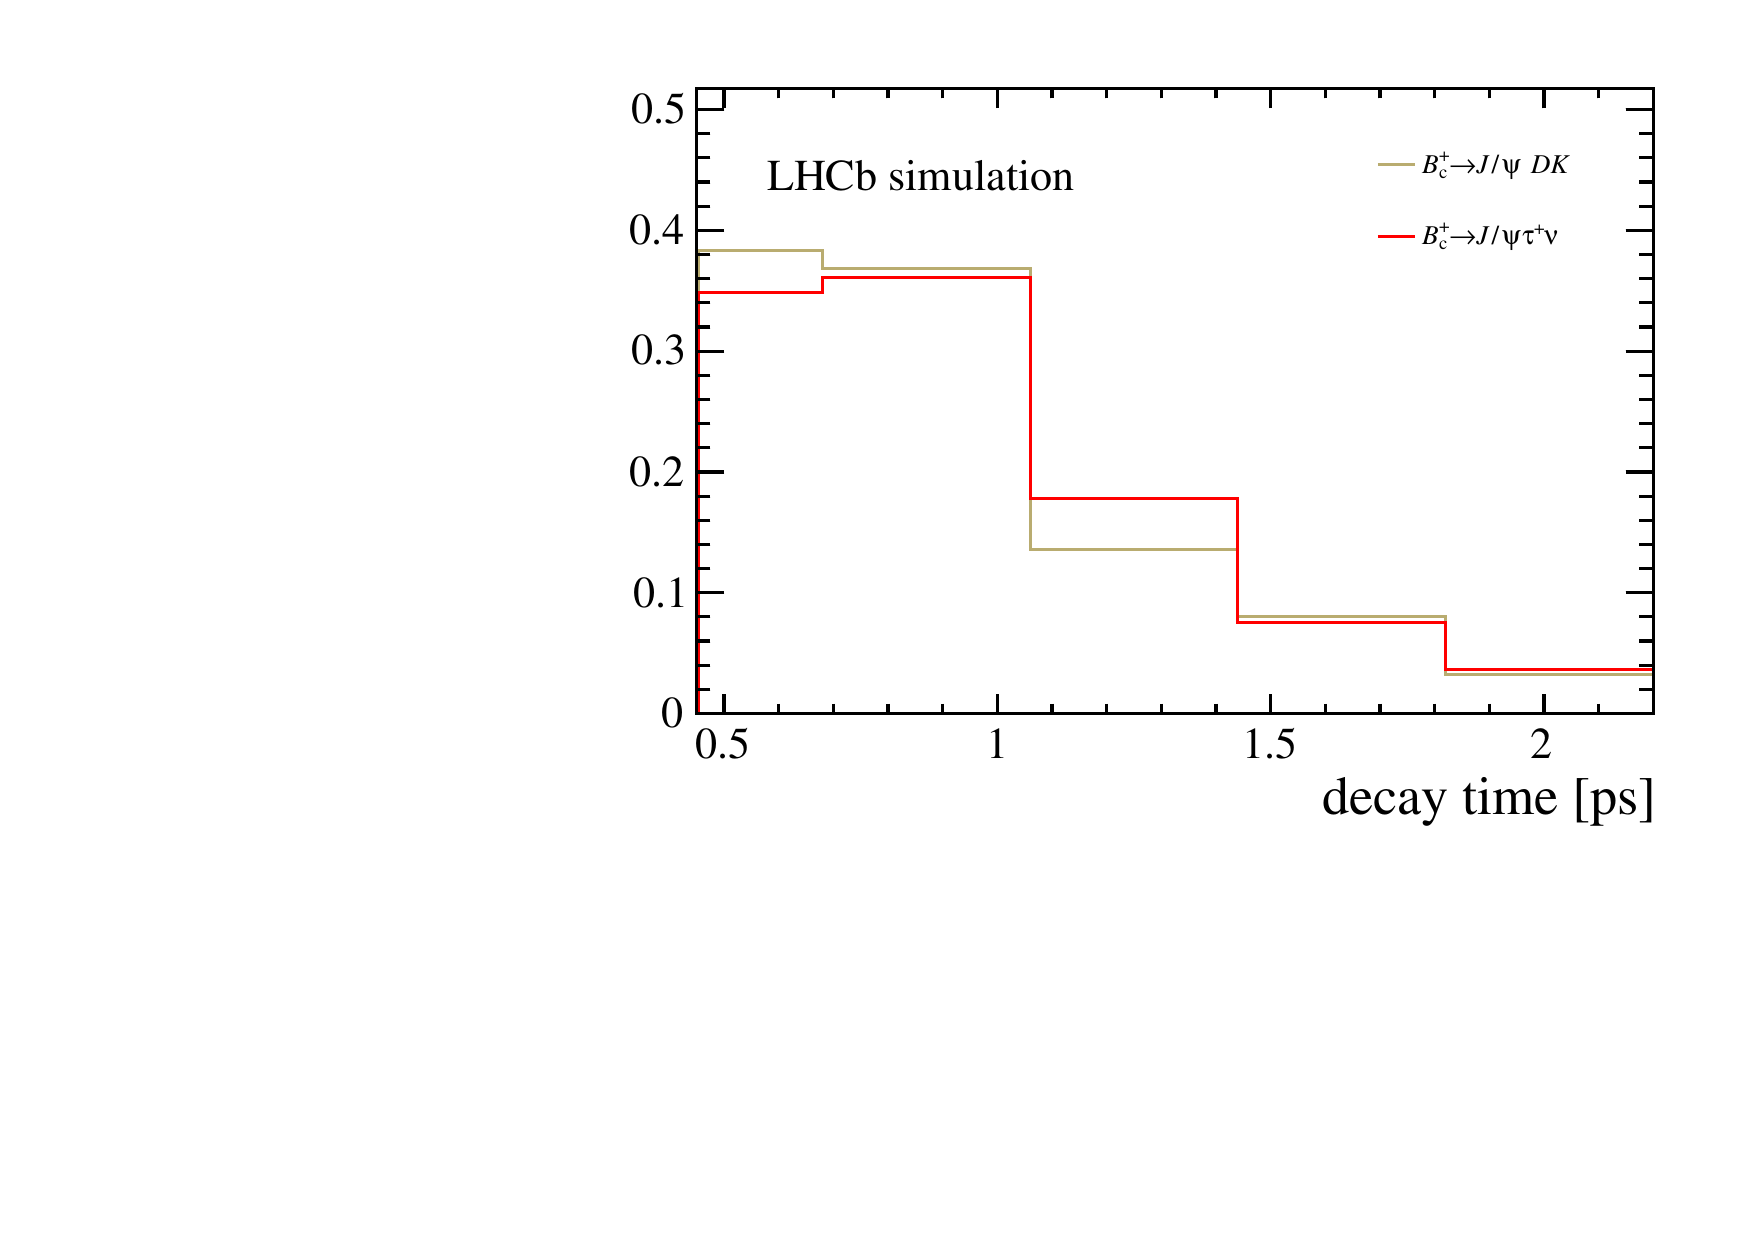}
    \includegraphics[width=0.3\textwidth]{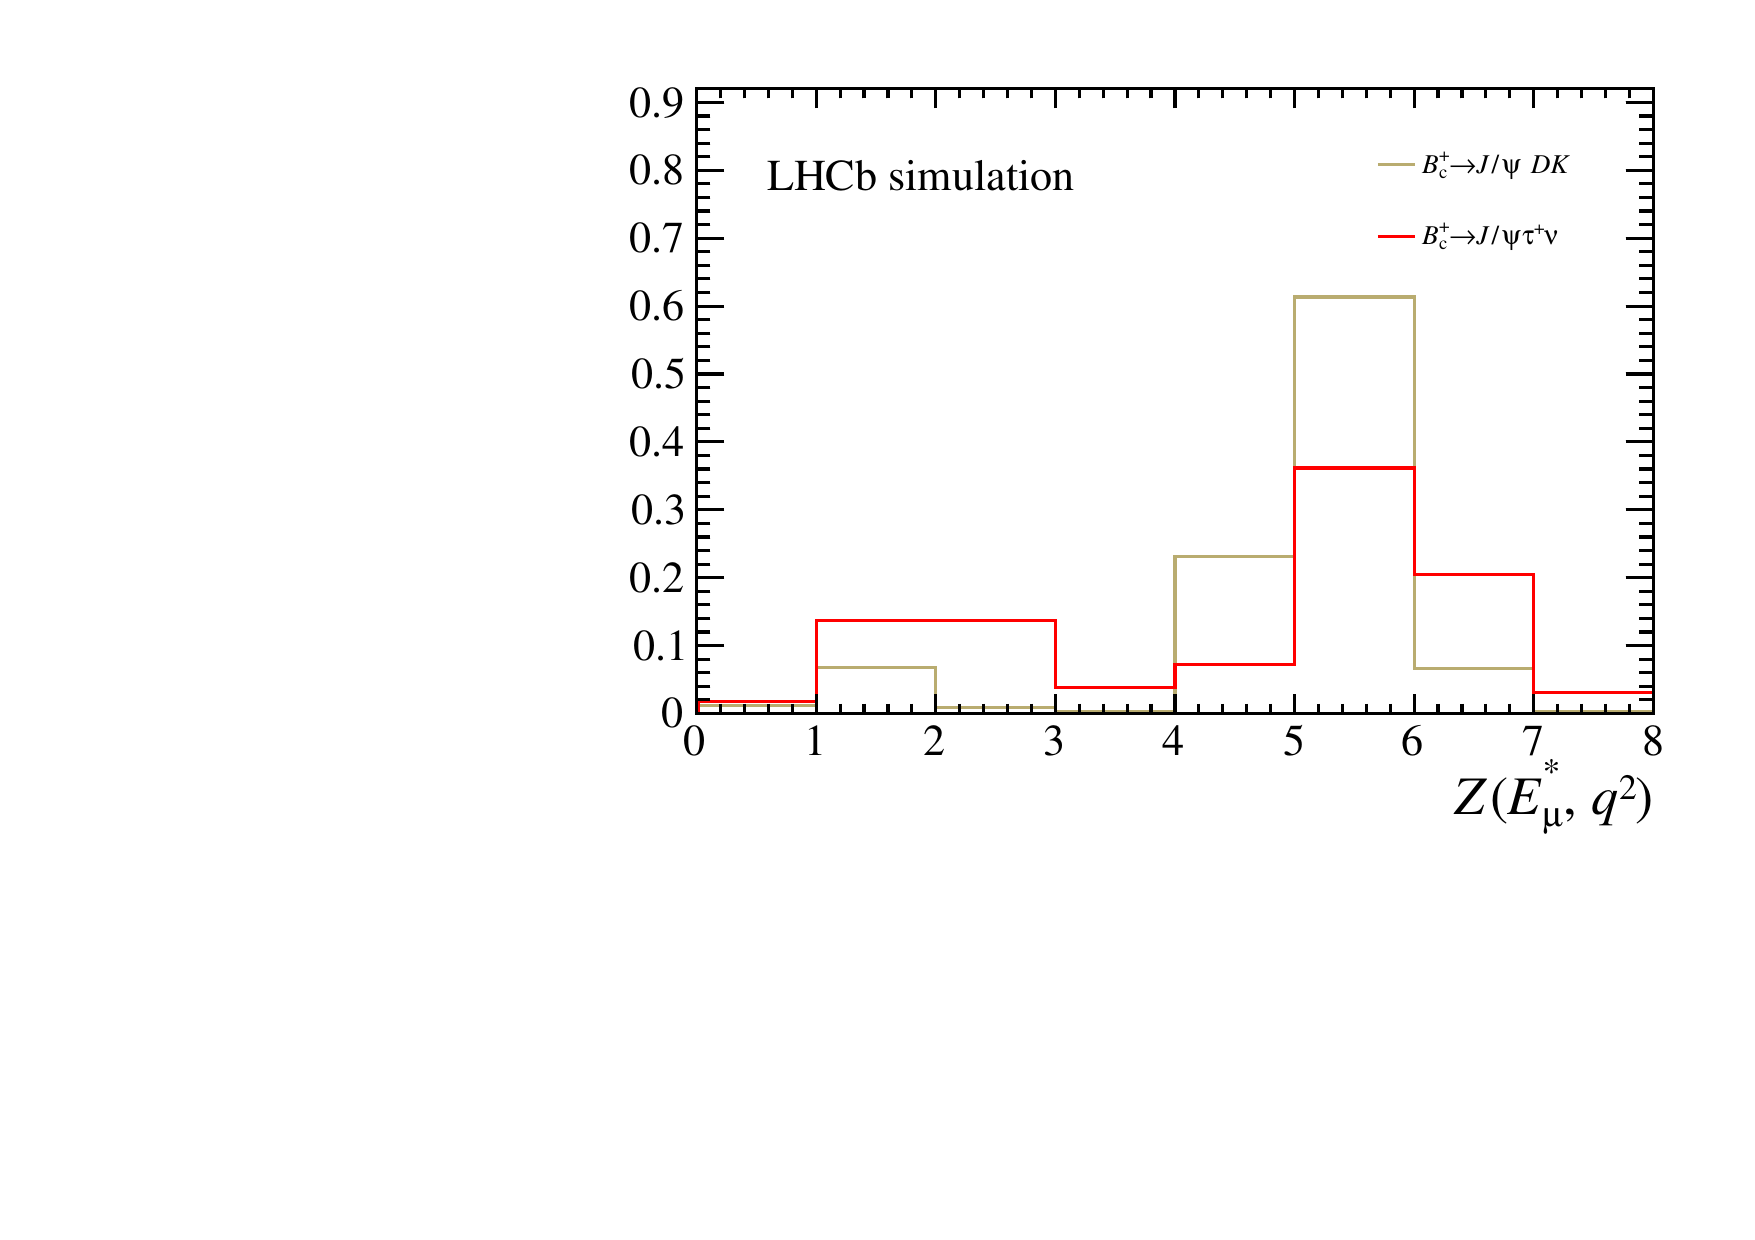}

    \caption{The distributions of rest-frame variables for the $B_{c}^+ \to J/\psi DX$ decays (green) compared with the signal mode (red). The top row shows two body decays, the center row shows quasi-two body decays, and the last row shows three body decays.}
    \label{fig:bc2jpsidx_templates}
\end{figure}

\begin{figure}
\centering
    \includegraphics[width=0.3\textwidth]{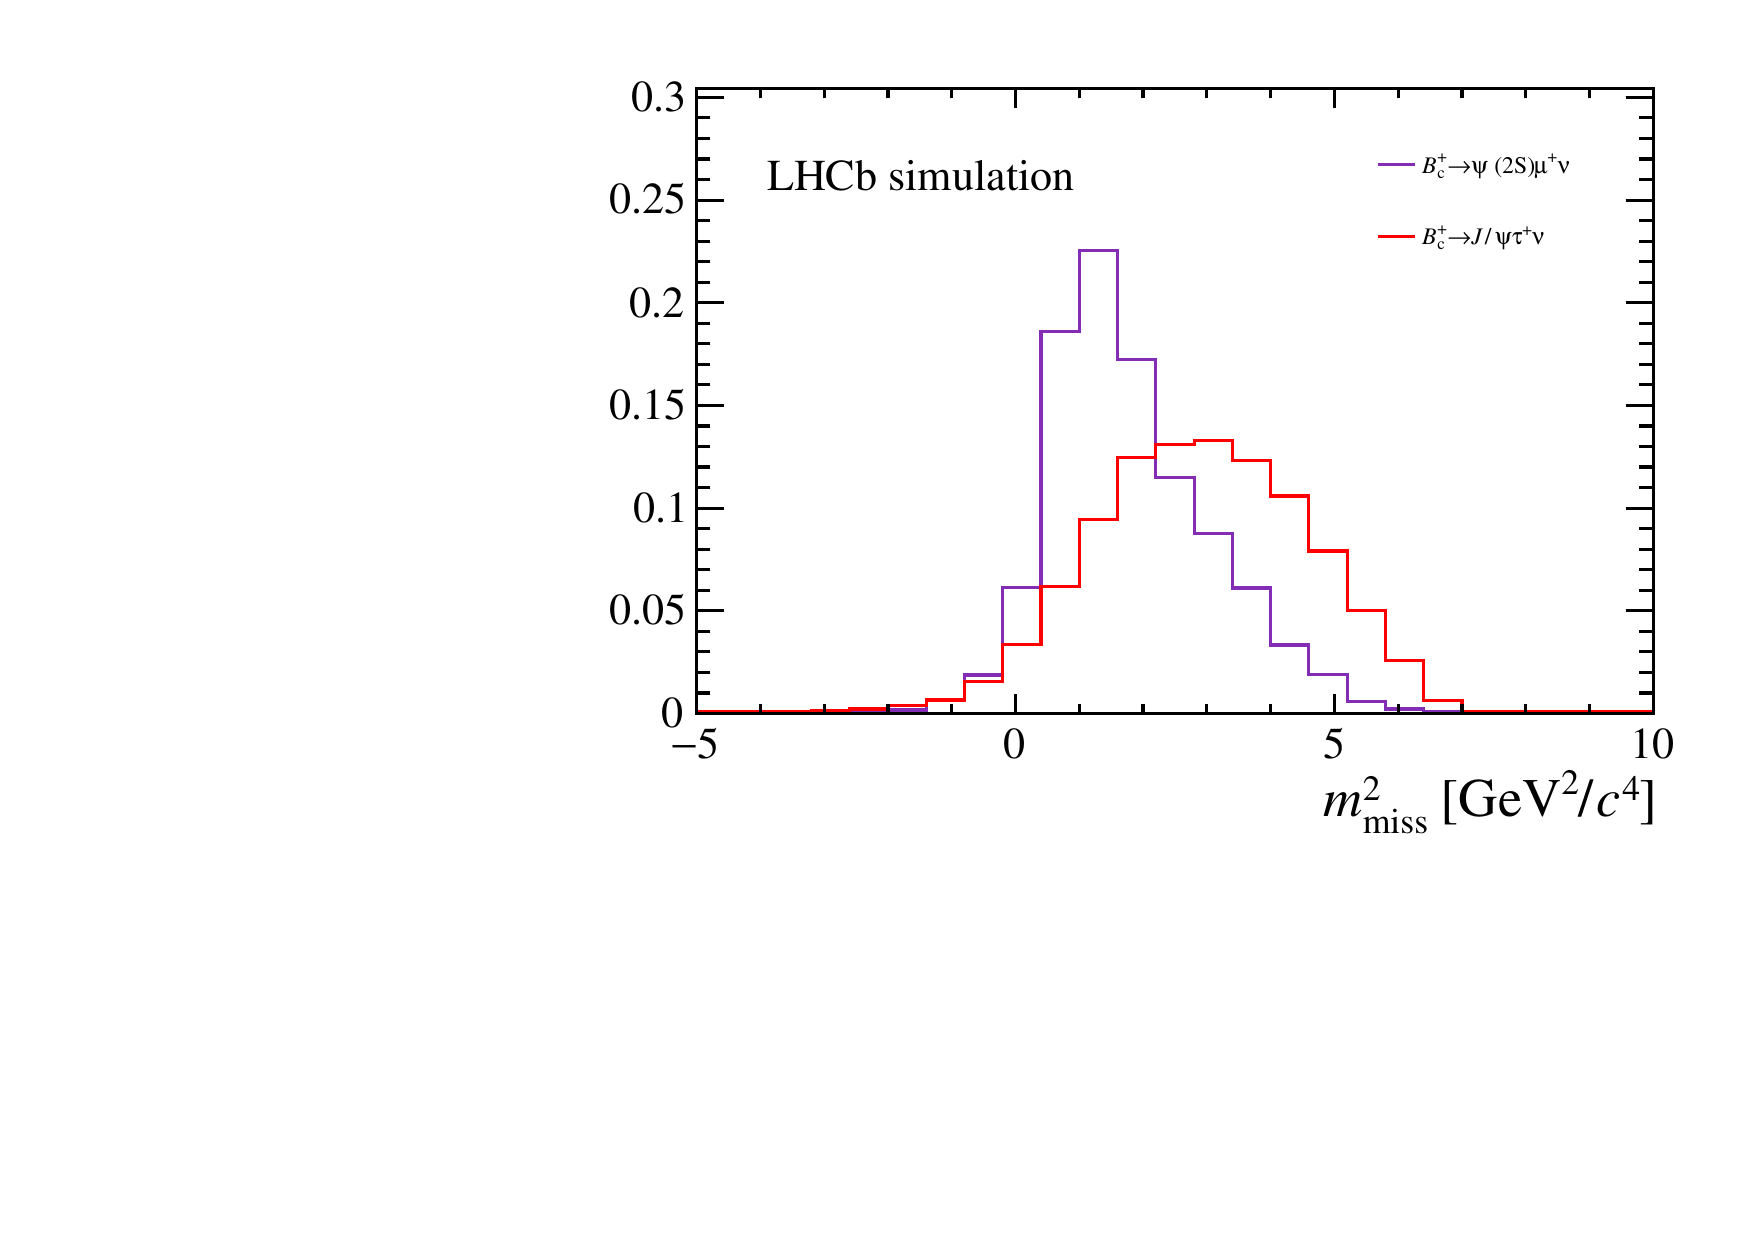}
    \includegraphics[width=0.3\textwidth]{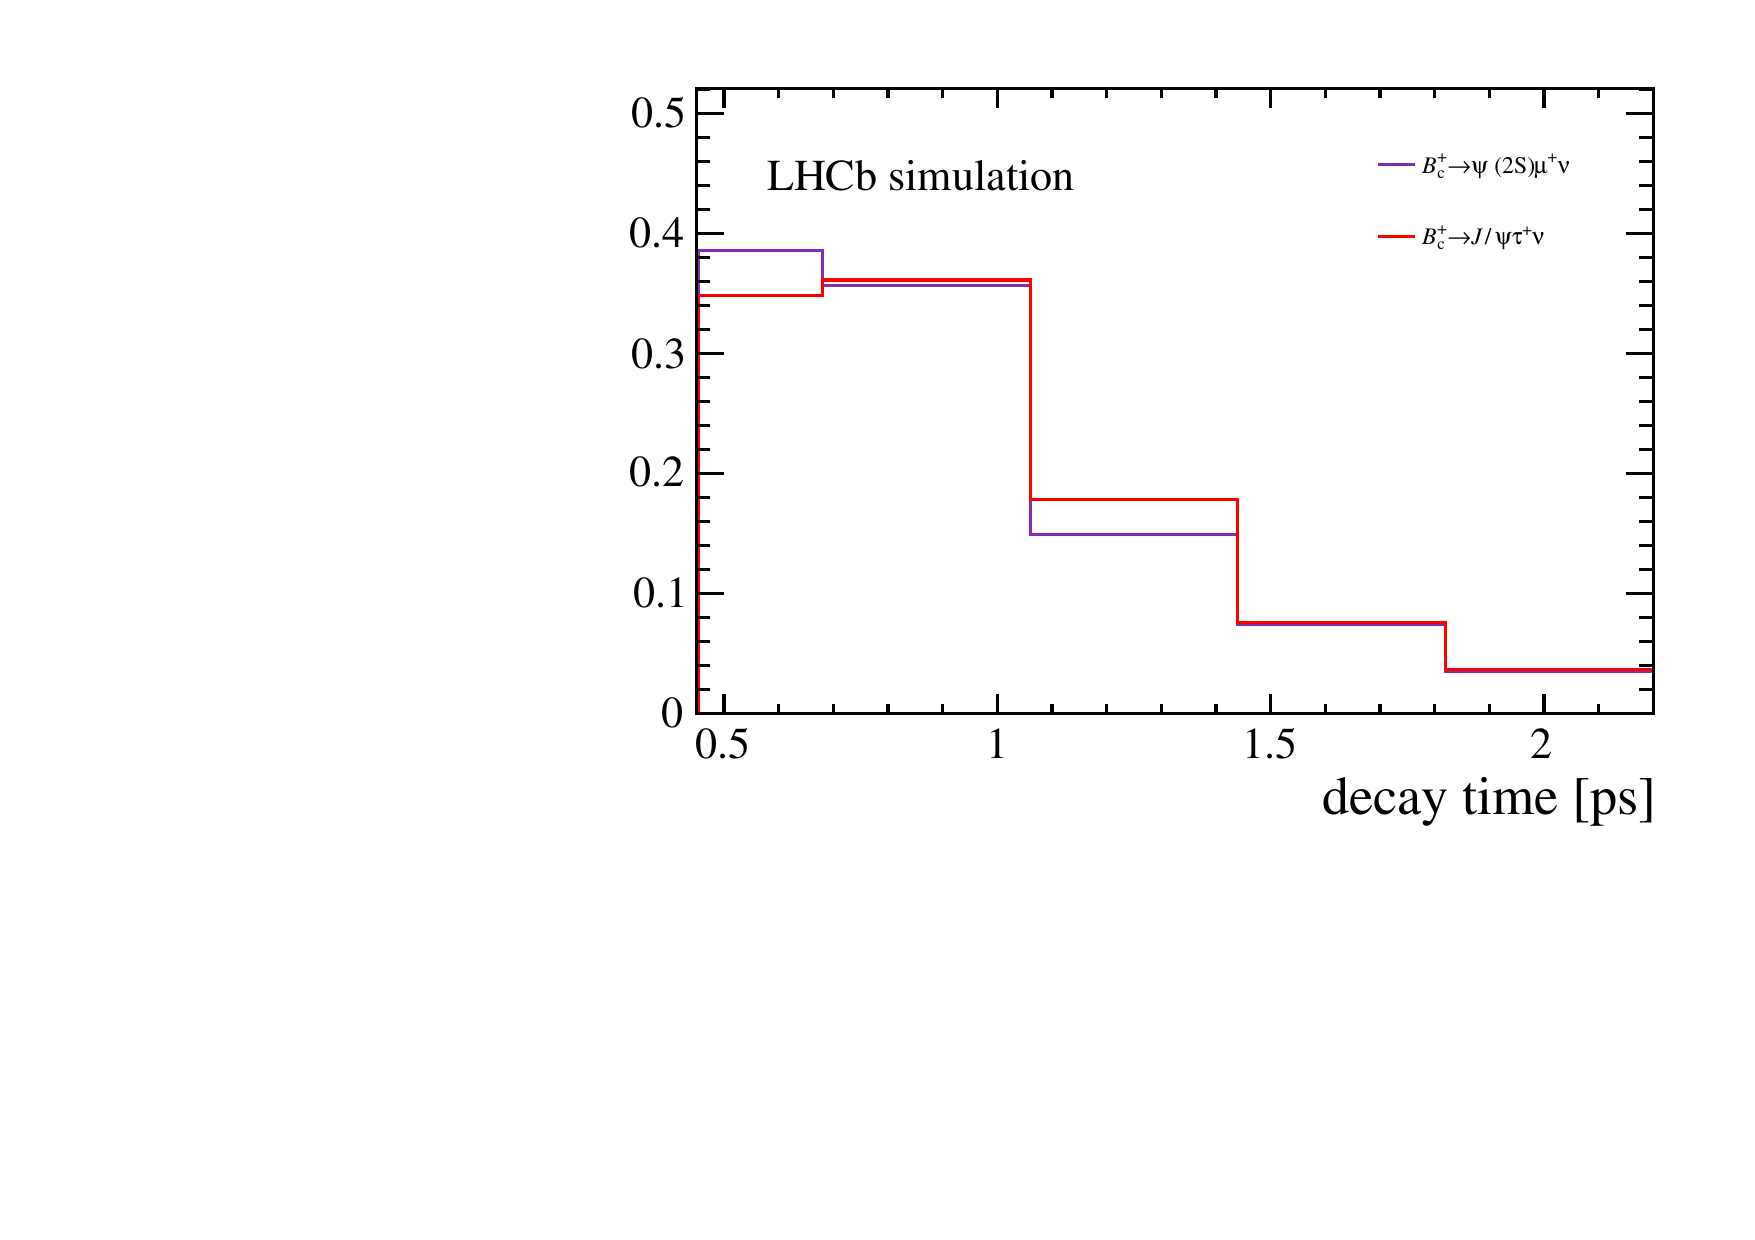}
    \includegraphics[width=0.3\textwidth]{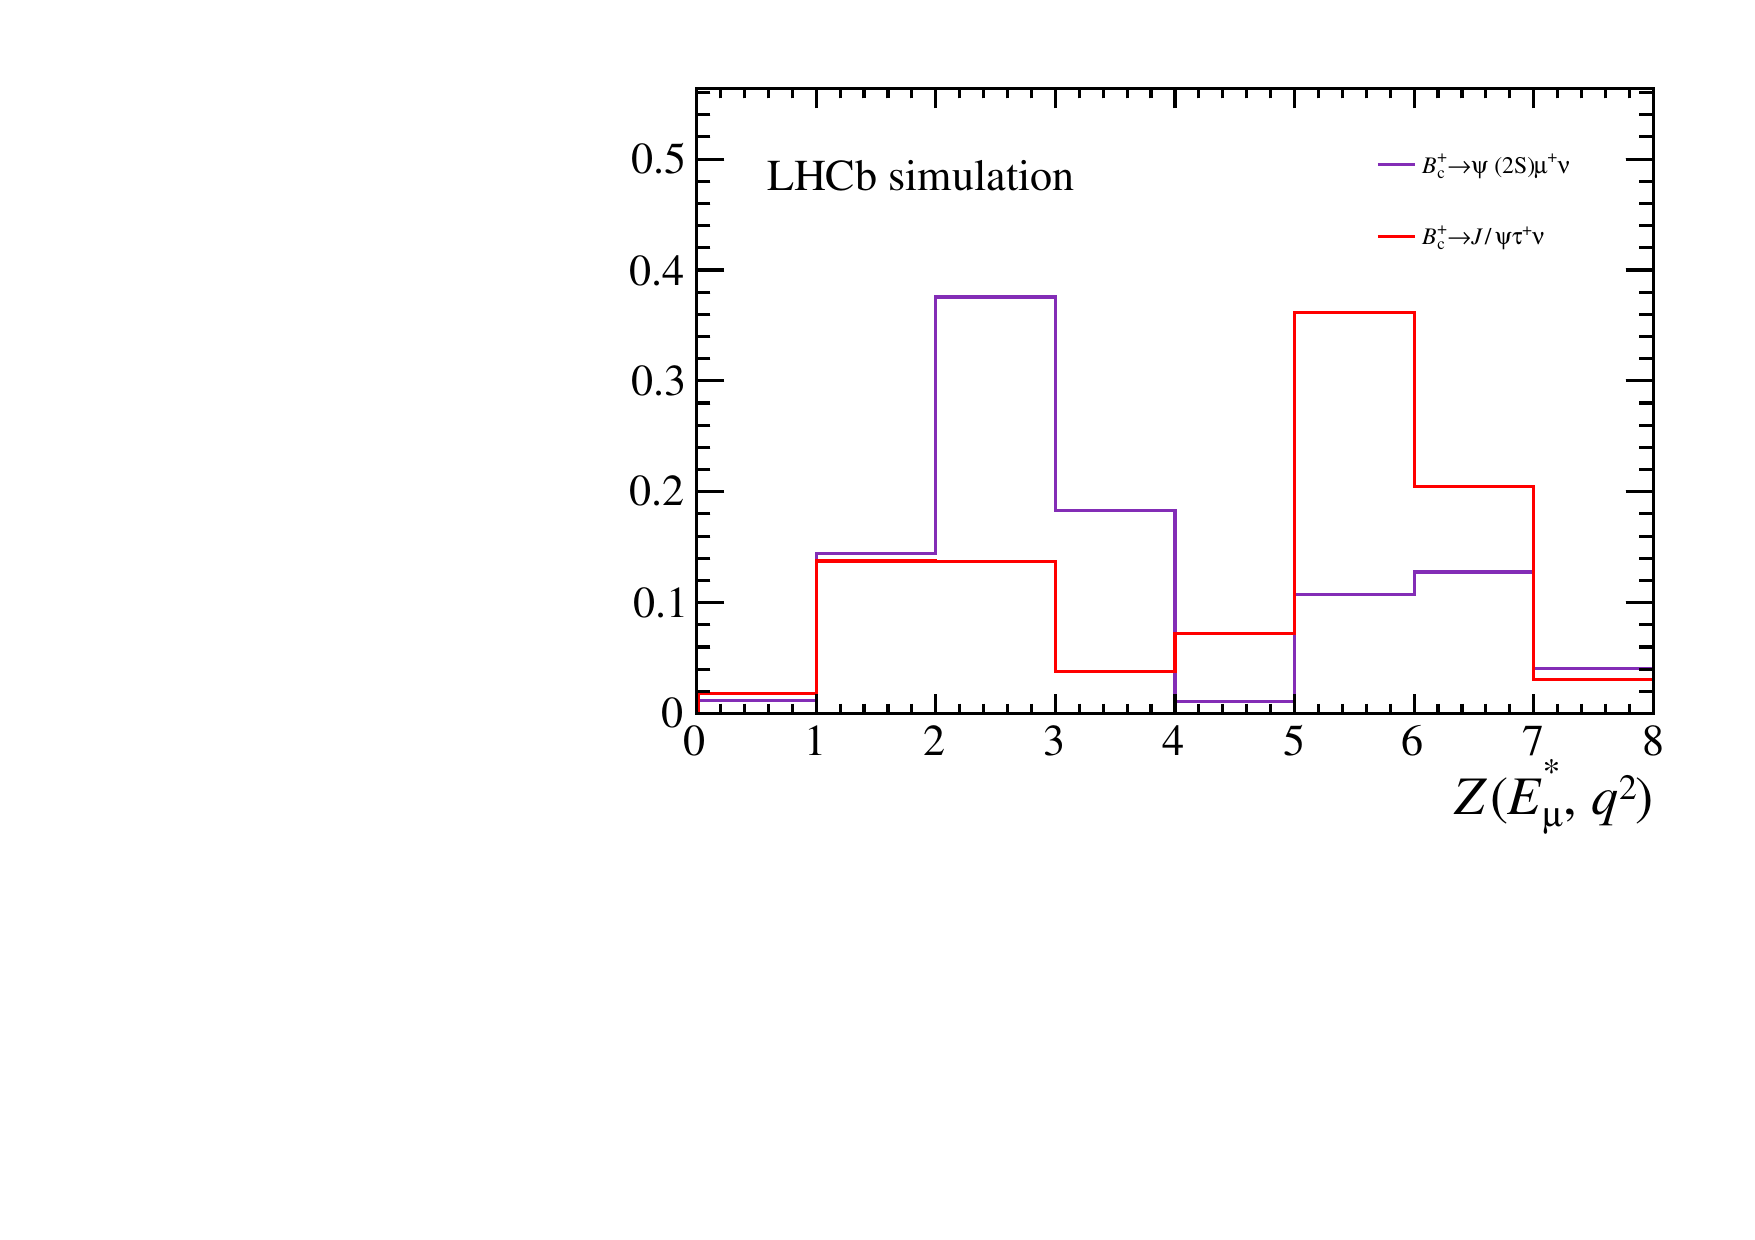}
    \includegraphics[width=0.3\textwidth]{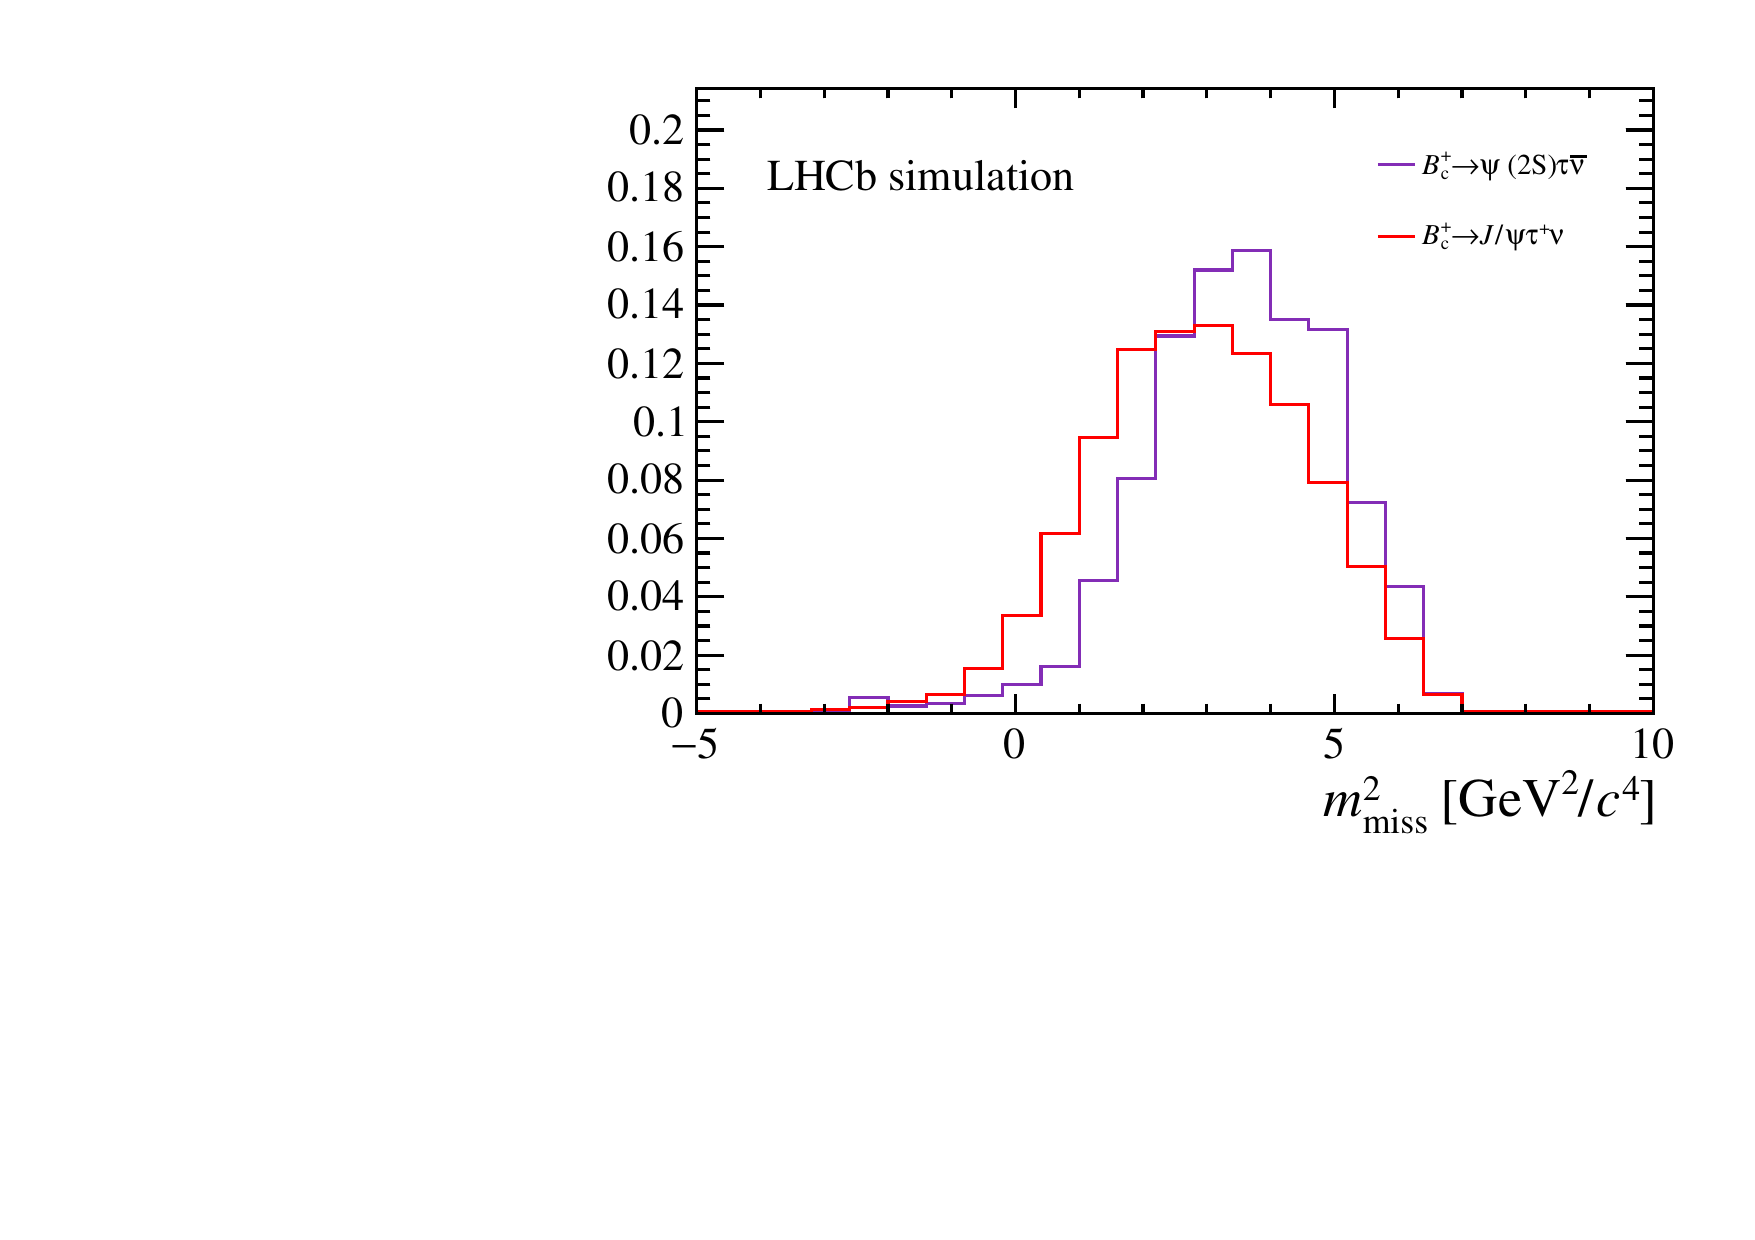}
    \includegraphics[width=0.3\textwidth]{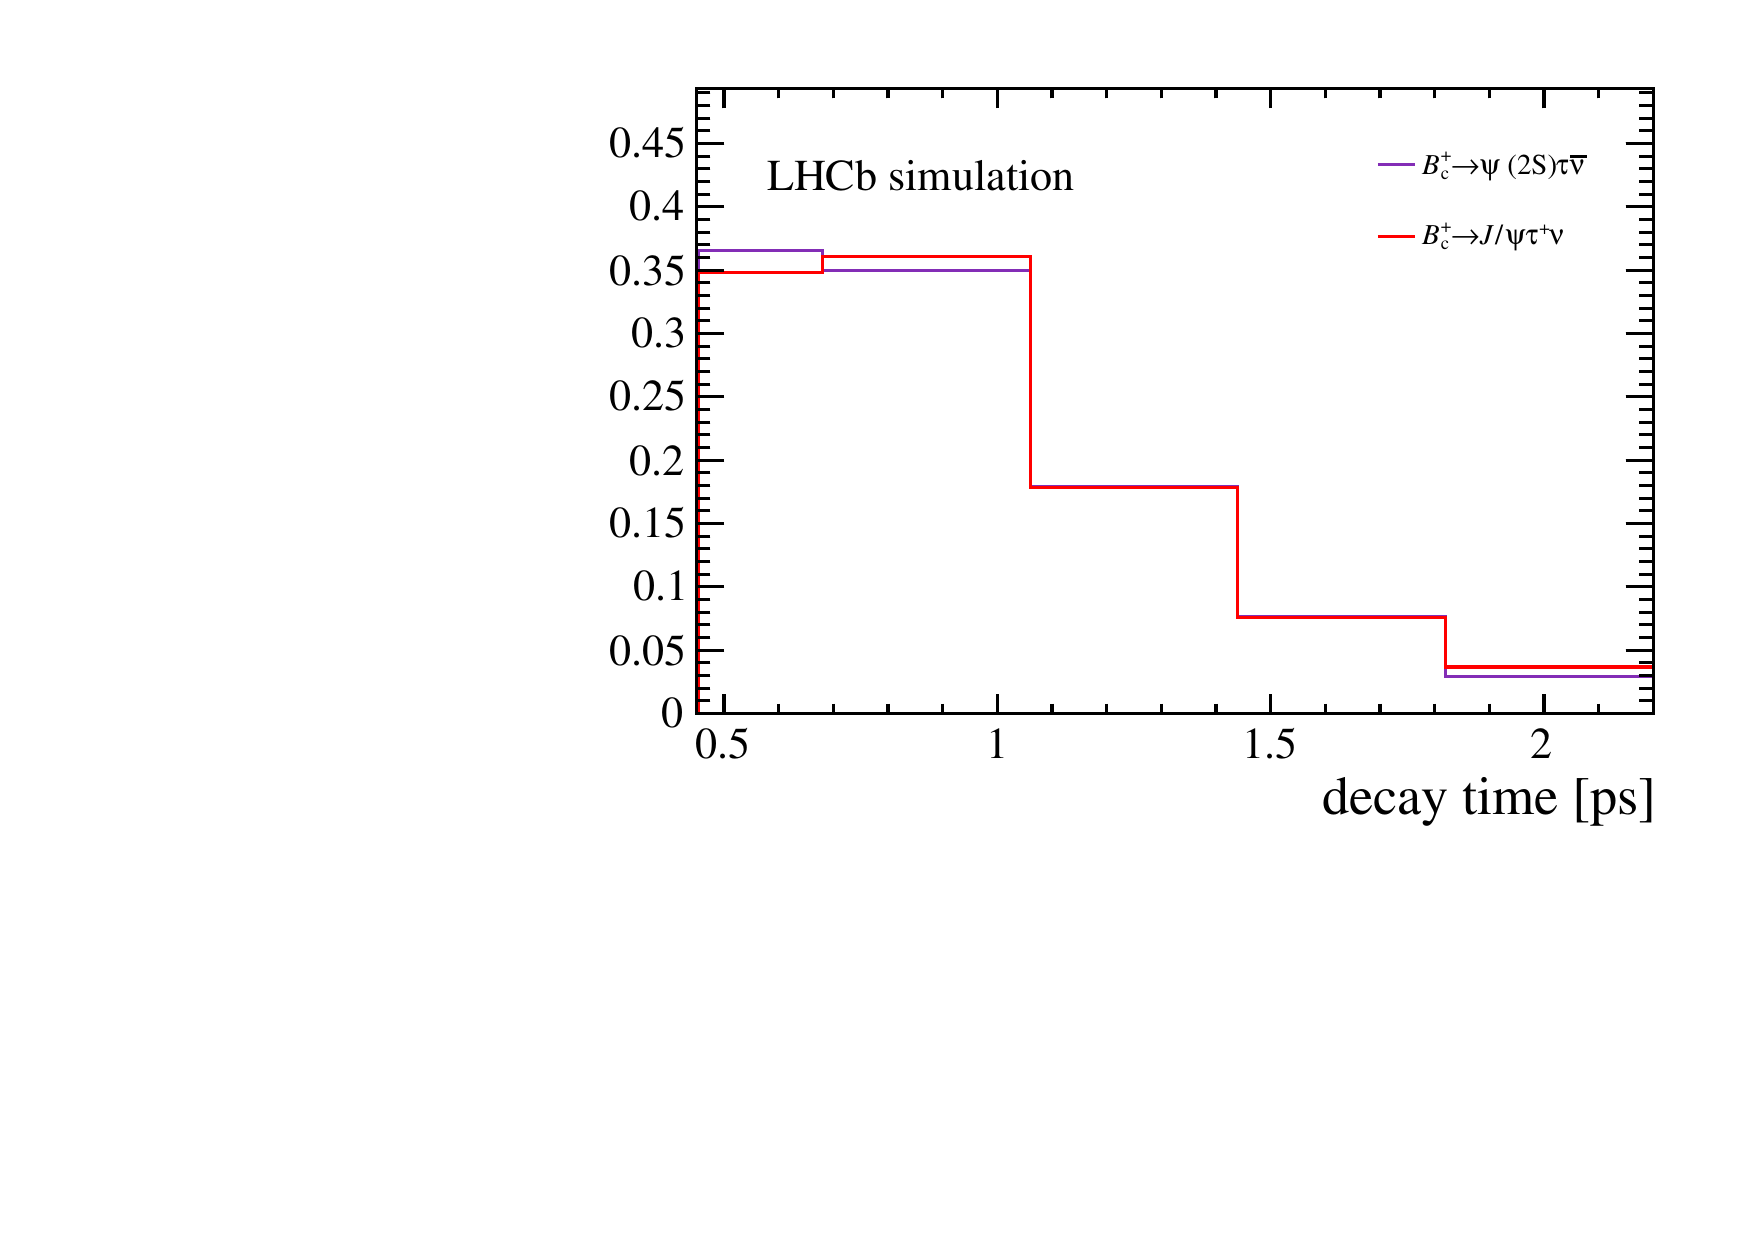}
    \includegraphics[width=0.3\textwidth]{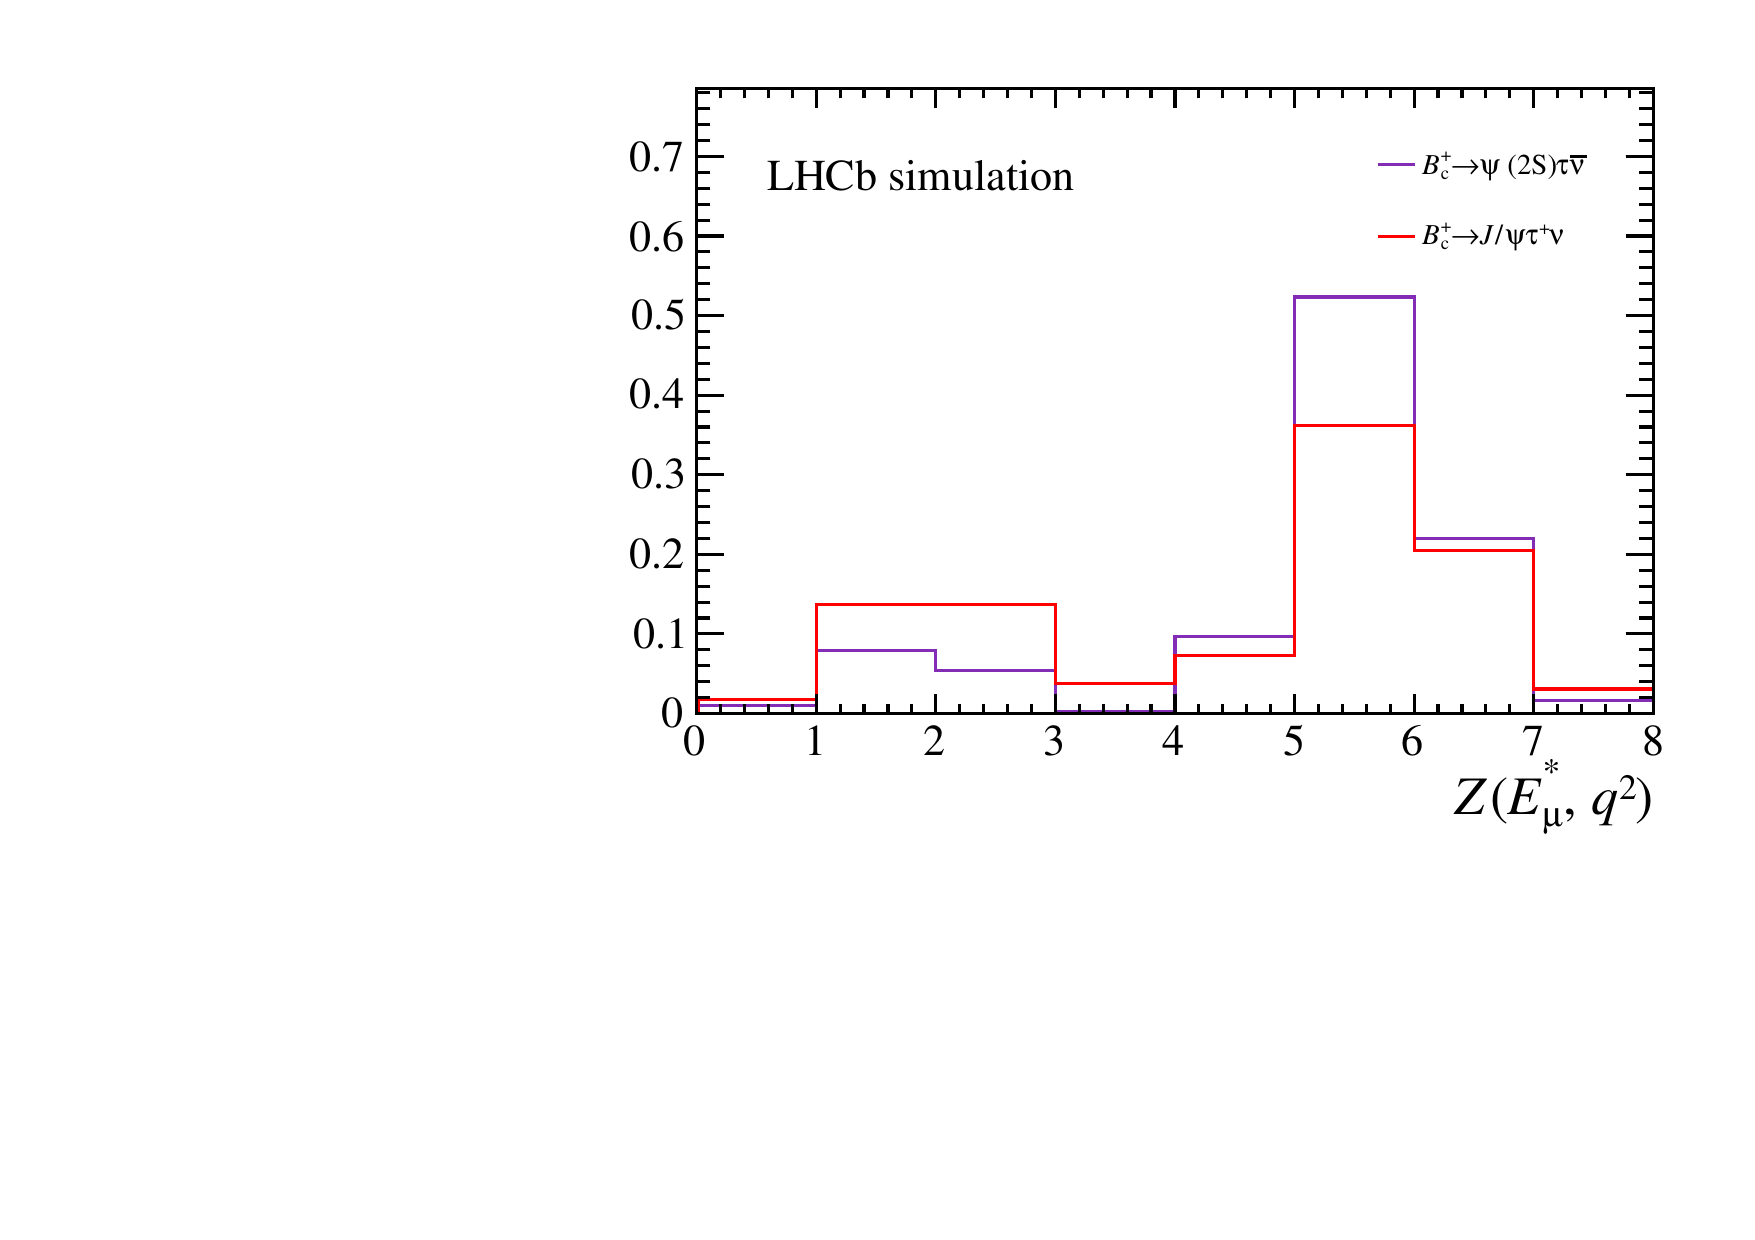}
    \caption{The distributions of rest-frame variables for the $B_c^+ \to \psi(2S) \mup \nu_{\mu}$ (top) and $B_c^+ \to \psi(2S) \tau^+ \nu_{\tau}$ background (bottom) (purple) compared with the signal mode (red).}
    \label{fig:bc2psi2s_templates}
\end{figure}

\begin{figure}
    \centering
    \includegraphics[width=0.3\textwidth]{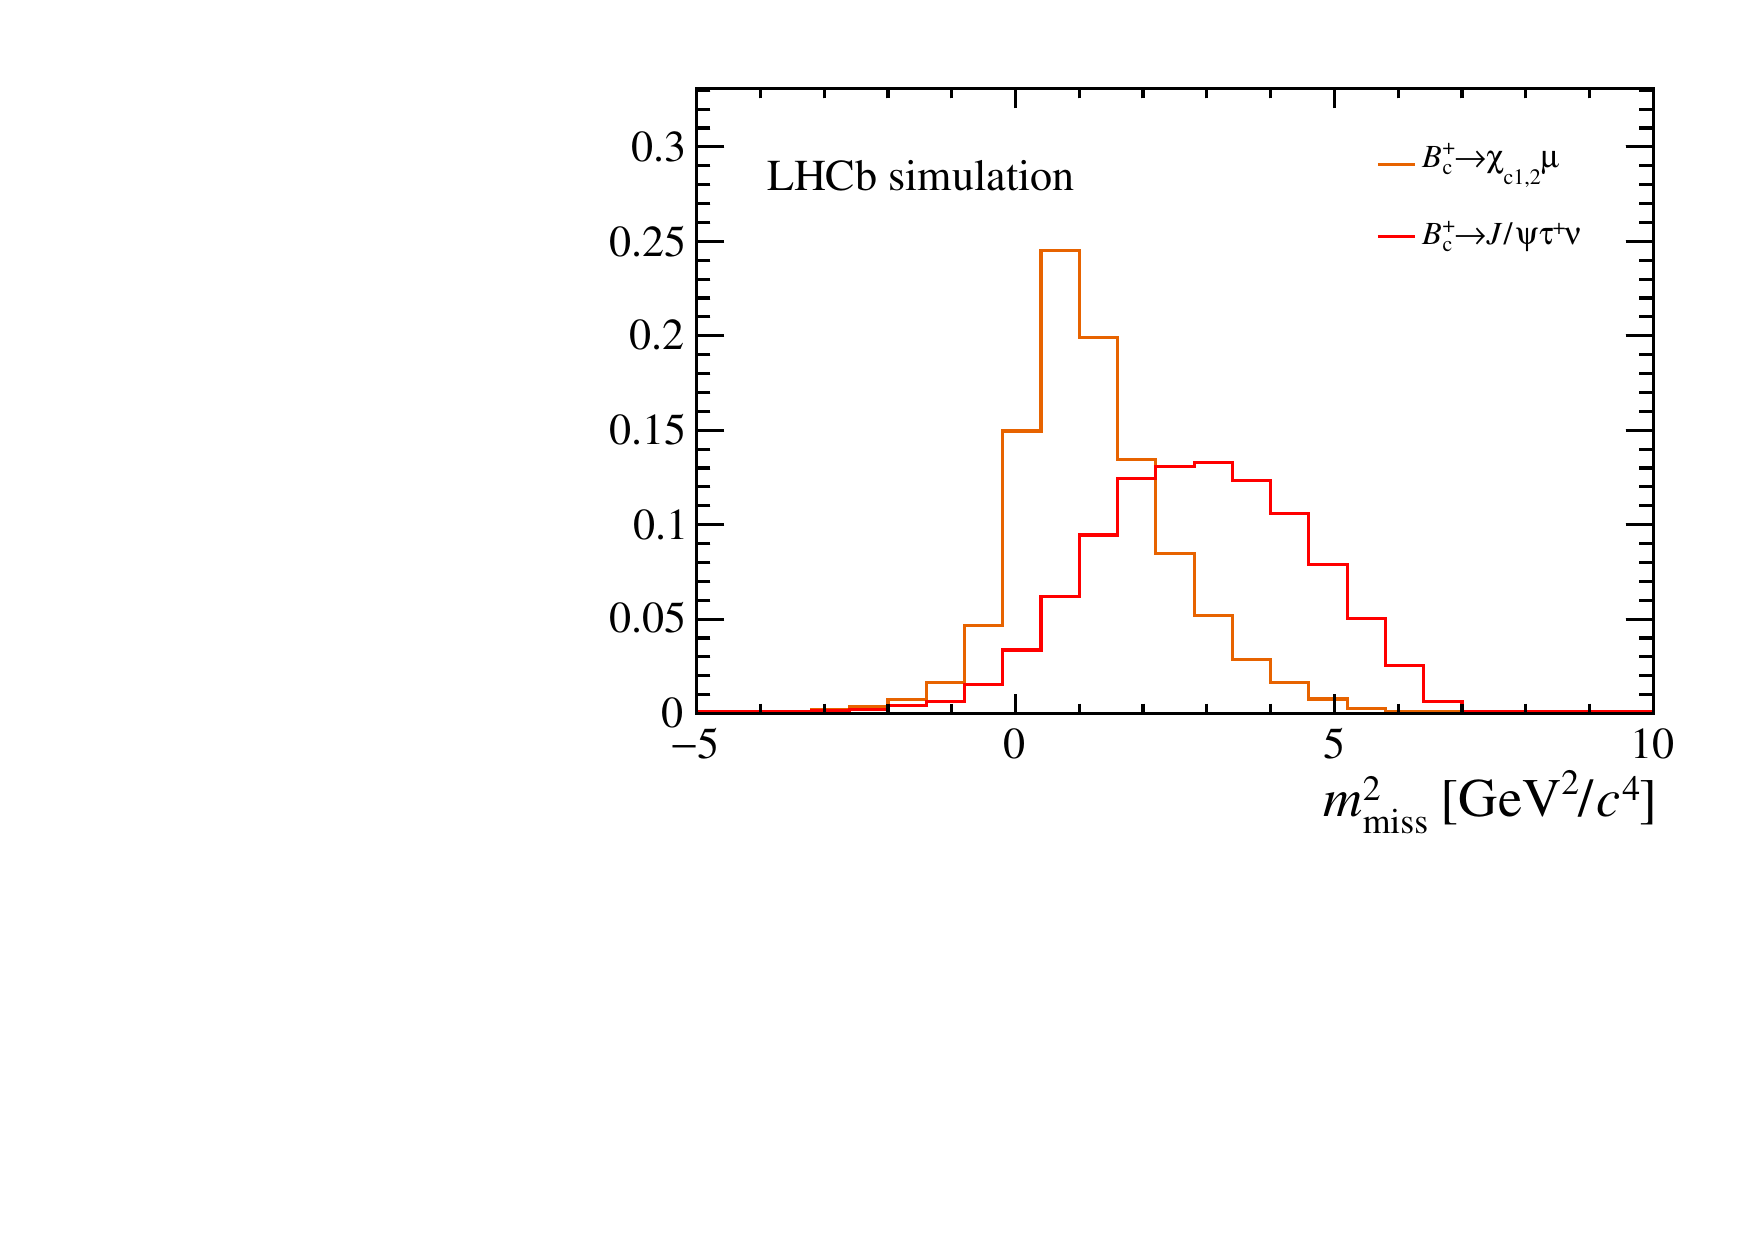}
    \includegraphics[width=0.3\textwidth]{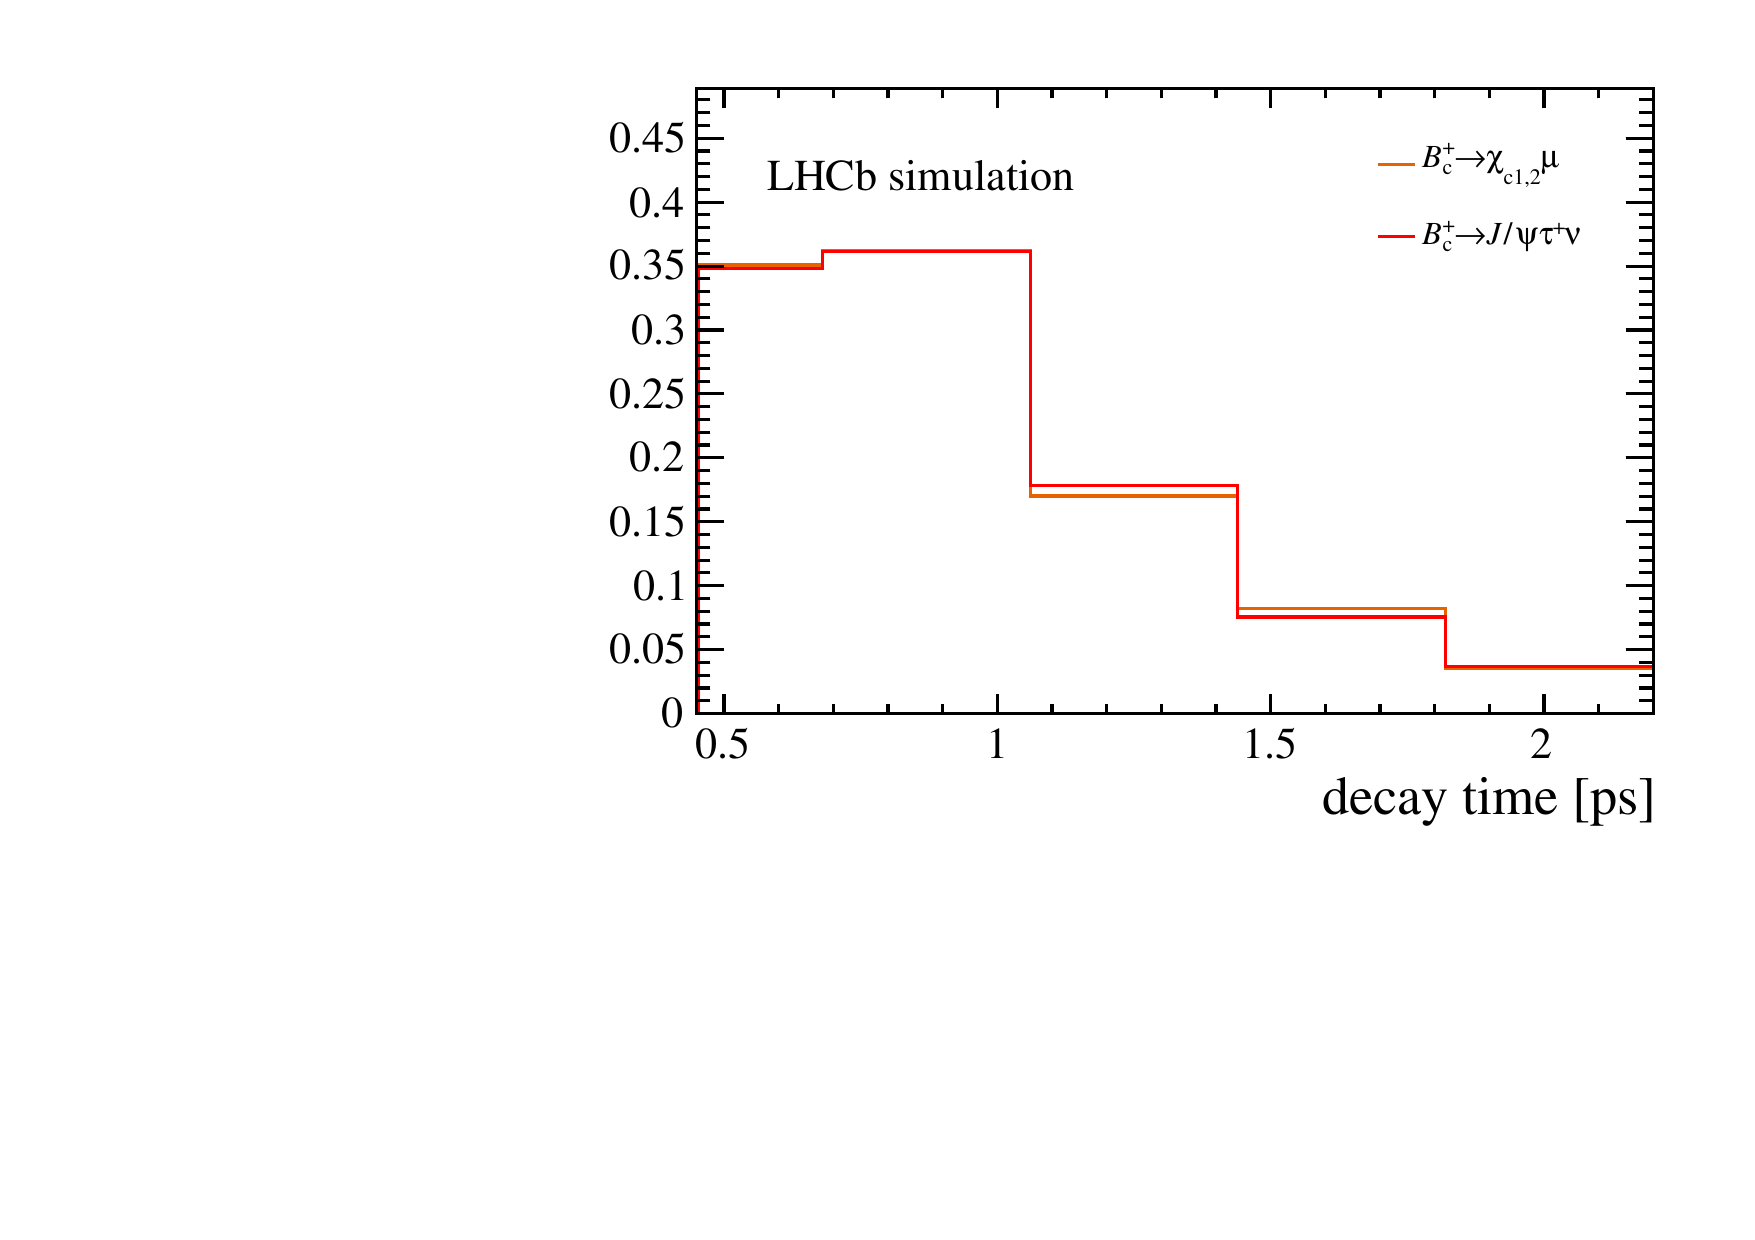}    \includegraphics[width=0.3\textwidth]{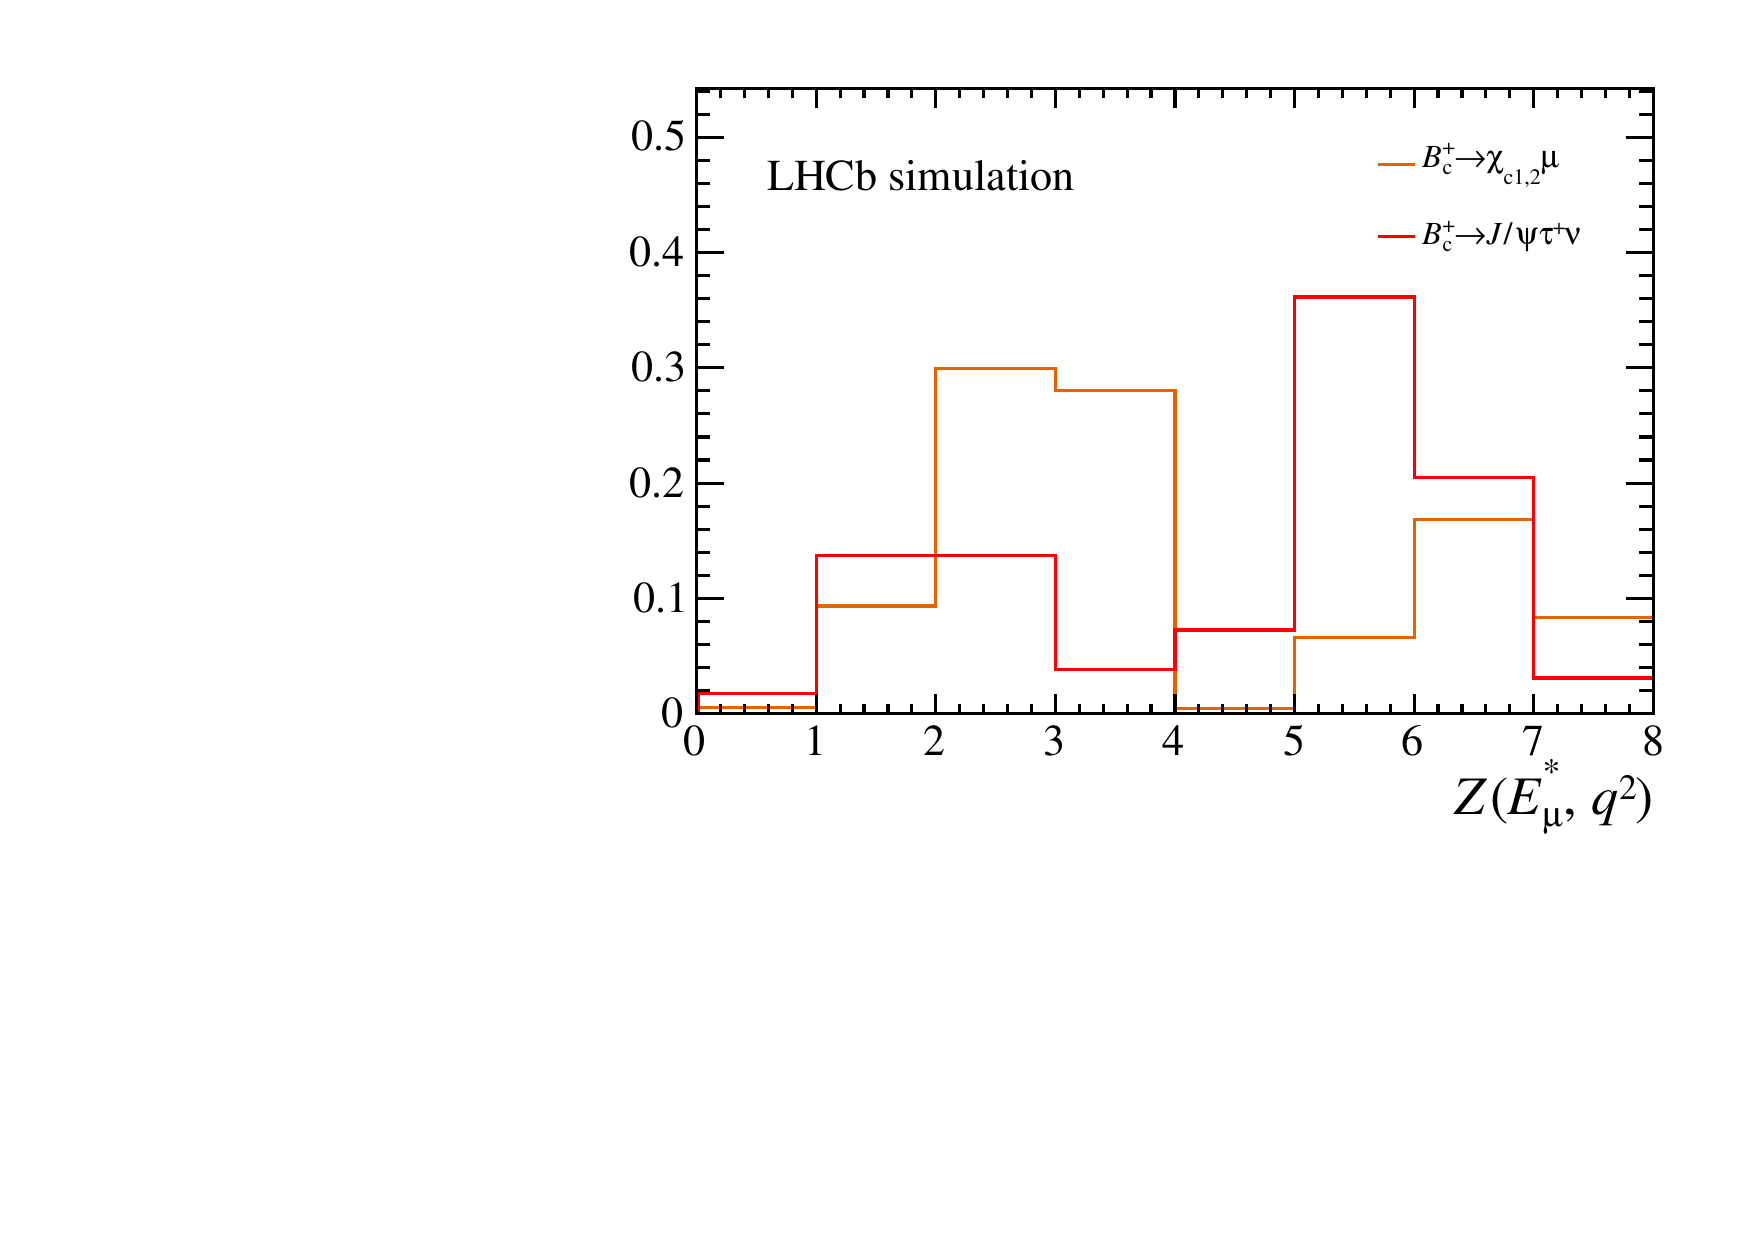}    
    \caption{The distributions of rest-frame variables for the $B_c^+ \to \chi_{c1,2} \mup \nu_{\mu}$ background (orange) compared with the signal mode (red).}
    \label{fig:bc2chicmu_templates}
\end{figure}

\begin{figure}
    \centering
    \includegraphics[width=0.5\linewidth]{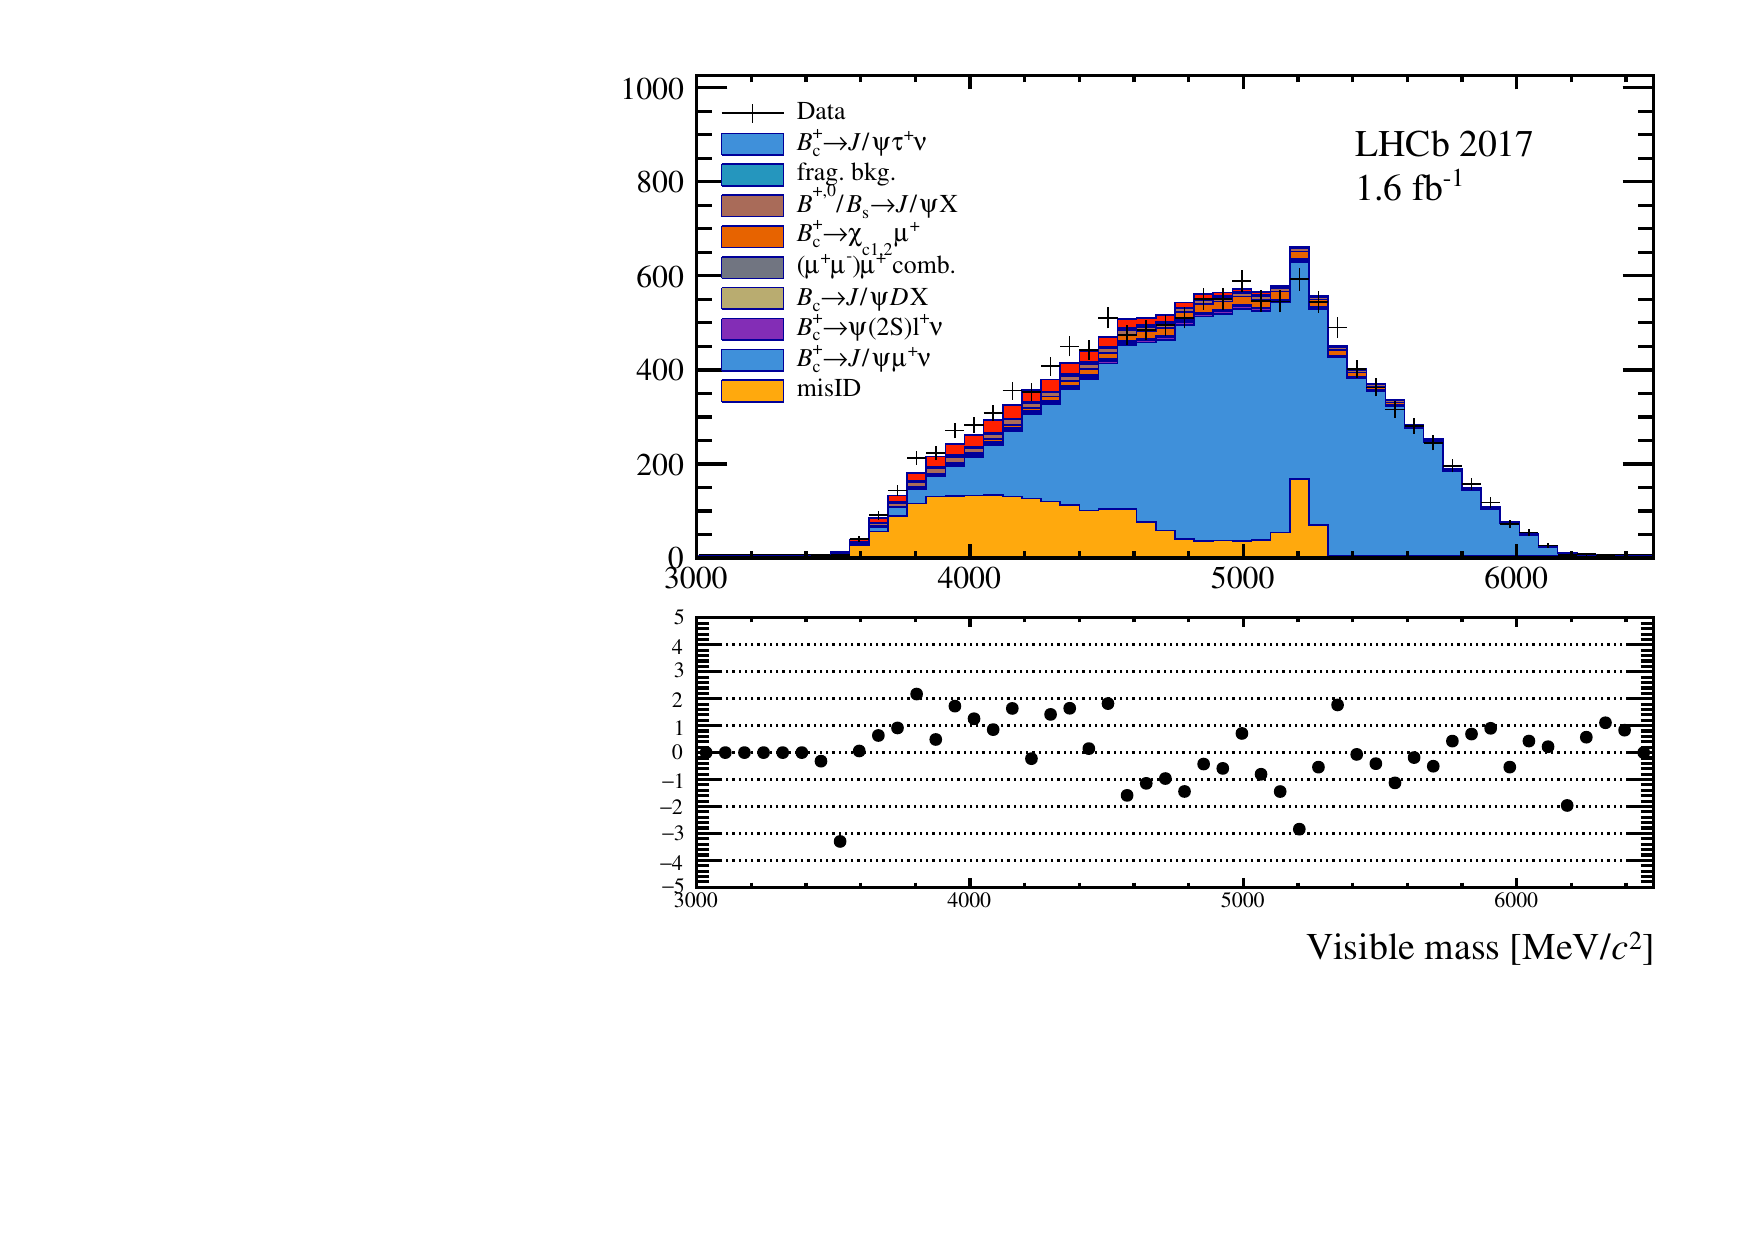}
    \caption{Postfit comparison of the visible mass distribution.}
    \label{fig:Bc_MM}
\end{figure}

\begin{figure}
    \centering
    \includegraphics[width=0.5\linewidth]{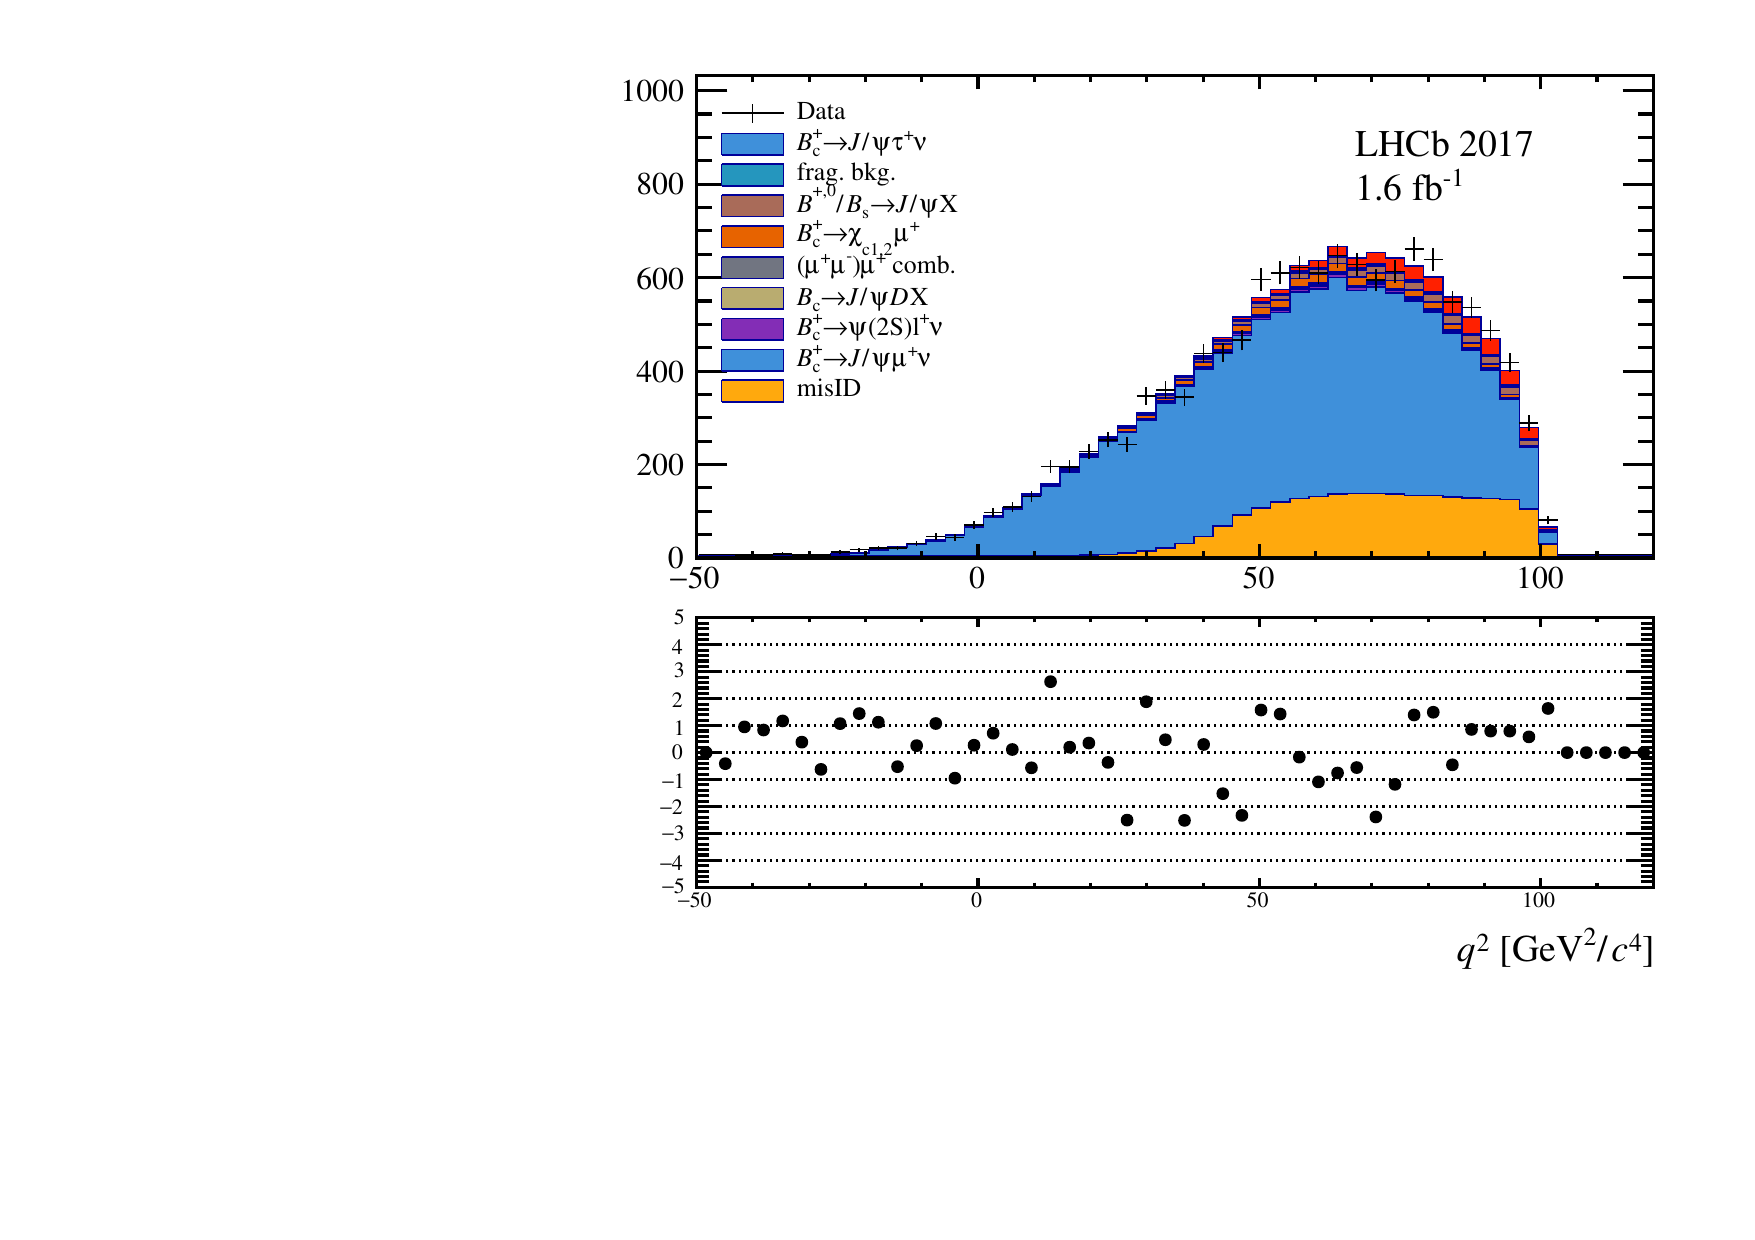}
    \caption{Postfit comparison of the $q^2$ distribution.}
    \label{fig:q2}
\end{figure}

\begin{figure}
    \centering
    \includegraphics[width=0.5\linewidth]{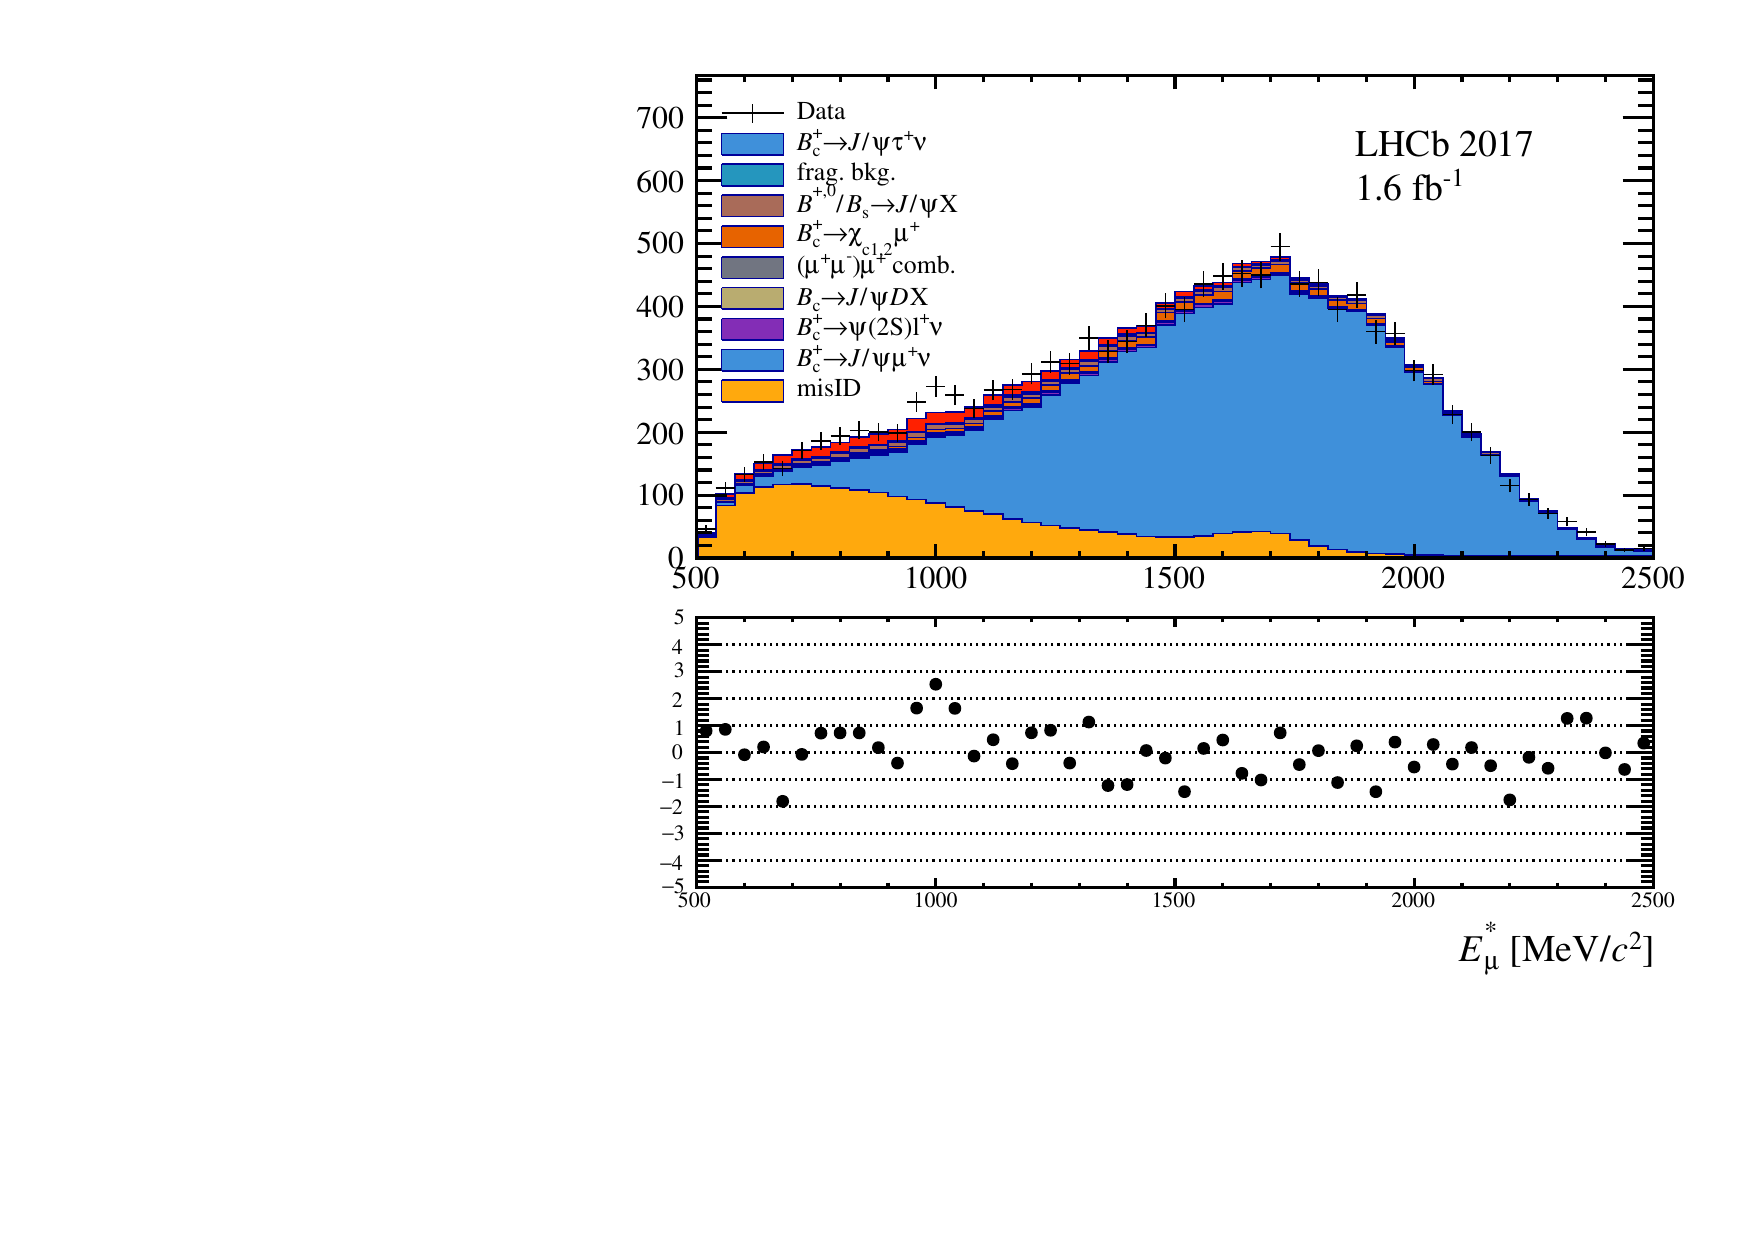}
    \caption{Postfit comparison of the $E_{\mu}^*$ distribution.}
    \label{fig:El}
\end{figure}

\clearpage
