# Supplementary material for: Measurement of the ratio of branching fractions $\mathcal{B}(B_c^+ \to J/\psi \tau^+ \nu_{\tau})/\mathcal{B}(B_c^+ \to J/\psi \mu^+ \nu_{\mu})$
Source: arXiv:2606.10018 source file (2026-10-01)
Supplement: Supplementary file 2 [file appendix.tex]

% ===============================================================================
% Purpose: appendix to the standard template: standard symbol alises from Ulrik
% Author: Tomasz Skwarnicki
% Created on: 2009-09-24
% ===============================================================================

%{\noindent\normalfont\bfseries\Large Appendices}
\clearpage
\section*{Appendices}

\appendix

\section{Justification for PRL}

This Letter presents the most precise measurement to date of the observable $\mathcal{R}(J/\psi)$ from any experiment, one of the key observables in the tests of lepton flavor universality, a fundamental element of the Standard Model~(SM). The current measurements primarily performed with light B mesons are in nearly four standard deviation tension with the SM predictions.
We believe the timeliness of the results due to the great interest in tests of lepton flavor universality and the significantly improved uncertainties of the new measurement, owing to a larger dataset and reduction of the systematic uncertainties by more than a factor of two, satisfies the requirements for publication in Physical Review Letters.

\section*{Word count}

\begin{itemize}
    \item Main body text: 3071 words
    \item Figure: $150 /$, aspect ratio (0.76) $ + 20$ =  215 words
    \item Table: $13+6.5 \times 18$ lines. 130 words.
    \item Total: 3416
\end{itemize}
